# Supplementary material for: Approaches For Multi-View Redescription Mining
Source: arXiv:2006.12227 source file (2020-11-17)
Supplement: Supplementary file 1 [file EM1.tex]

\documentclass[12pt]{article}
\usepackage[T1]{fontenc}
\usepackage[utf8]{inputenc}
\usepackage{graphicx}
\usepackage{url}
\usepackage{amsfonts}
\usepackage{bbm}
\usepackage[numbers]{natbib}
\usepackage{multirow}
\usepackage{amsmath}
\usepackage[numbers]{natbib}
\usepackage{algorithm}
\usepackage[noend]{algpseudocode}
\usepackage{color}
\usepackage{longtable} % To display tables on several pages
\usepackage{booktabs}

\usepackage[labelfont=bf,textfont=md]{caption}
\usepackage{subcaption}

\renewcommand\thetable{S\arabic{table}}

\captionsetup{
   labelsep = space,
%   justification = raggedright,
   font = {footnotesize},
   singlelinecheck=off,
%   skip=4pt,
   position=top}
   \setlength\LTcapwidth{\textwidth} % default value is 4in, I think

\title{Supplementary material to  - Multi-view redescription mining using tree-based multi-target prediction models}

\author{
        Matej Mihelčić, \\
        Department of Mathematics, Faculty of Science\\ 
        Bijenicka cesta 30, 10000 Zagreb, Croatia\\
        matmih@math.hr\\
		Sašo Džeroski \\
		Jožef Stefan Institute\\
		Jamova cesta 39, 1000 Ljubljana, Slovenia\\
		saso.dzeroski@ijs.si \\
		Tomislav Šmuc \\
                Ruđer Bošković Institute\\
		Bijenička cesta 54, 10000 Zagreb, Croatia\\
		tomislav.smuc@irb.hr 
}
\begin{document}
\maketitle

This document contains supplementary information for the manuscript \emph{Multi-view redescription mining using tree-based multi-target prediction models} submitted to the IEEE Access journal.

\section{Complete evaluation results of all approaches}

In this section, we present complete evaluation results of approaches presented in the manuscript \emph{Multi-view redescription mining using tree-based multi-target prediction models}. 

\subsection{Evaluating quality of produced redescription sets}
\label{sec:quality}
We present the results of evaluating our framework for multi-view redescription mining using one PCT as rule-generating model. We test the performance of this framework with different values of memory parameters (working and maximal allowed memory size). The result in boldface shows the best performing methodology for a given measure on a chosen dataset.  To shorten the notation, all results tables contain the following abbreviations: $AJ$ for the average Jaccard index of redescriptions contained in the redescription set, $AEJ$ for $AEJ_{sc}$, $AAJ$ for $AAJ_{sc}$, $ARC$ for $comp_{sc}$ and $RSS$ for the $total_{sc}$.  

\begin{figure}[H]
\centerline{\includegraphics[width=1.0\textwidth]{Figures/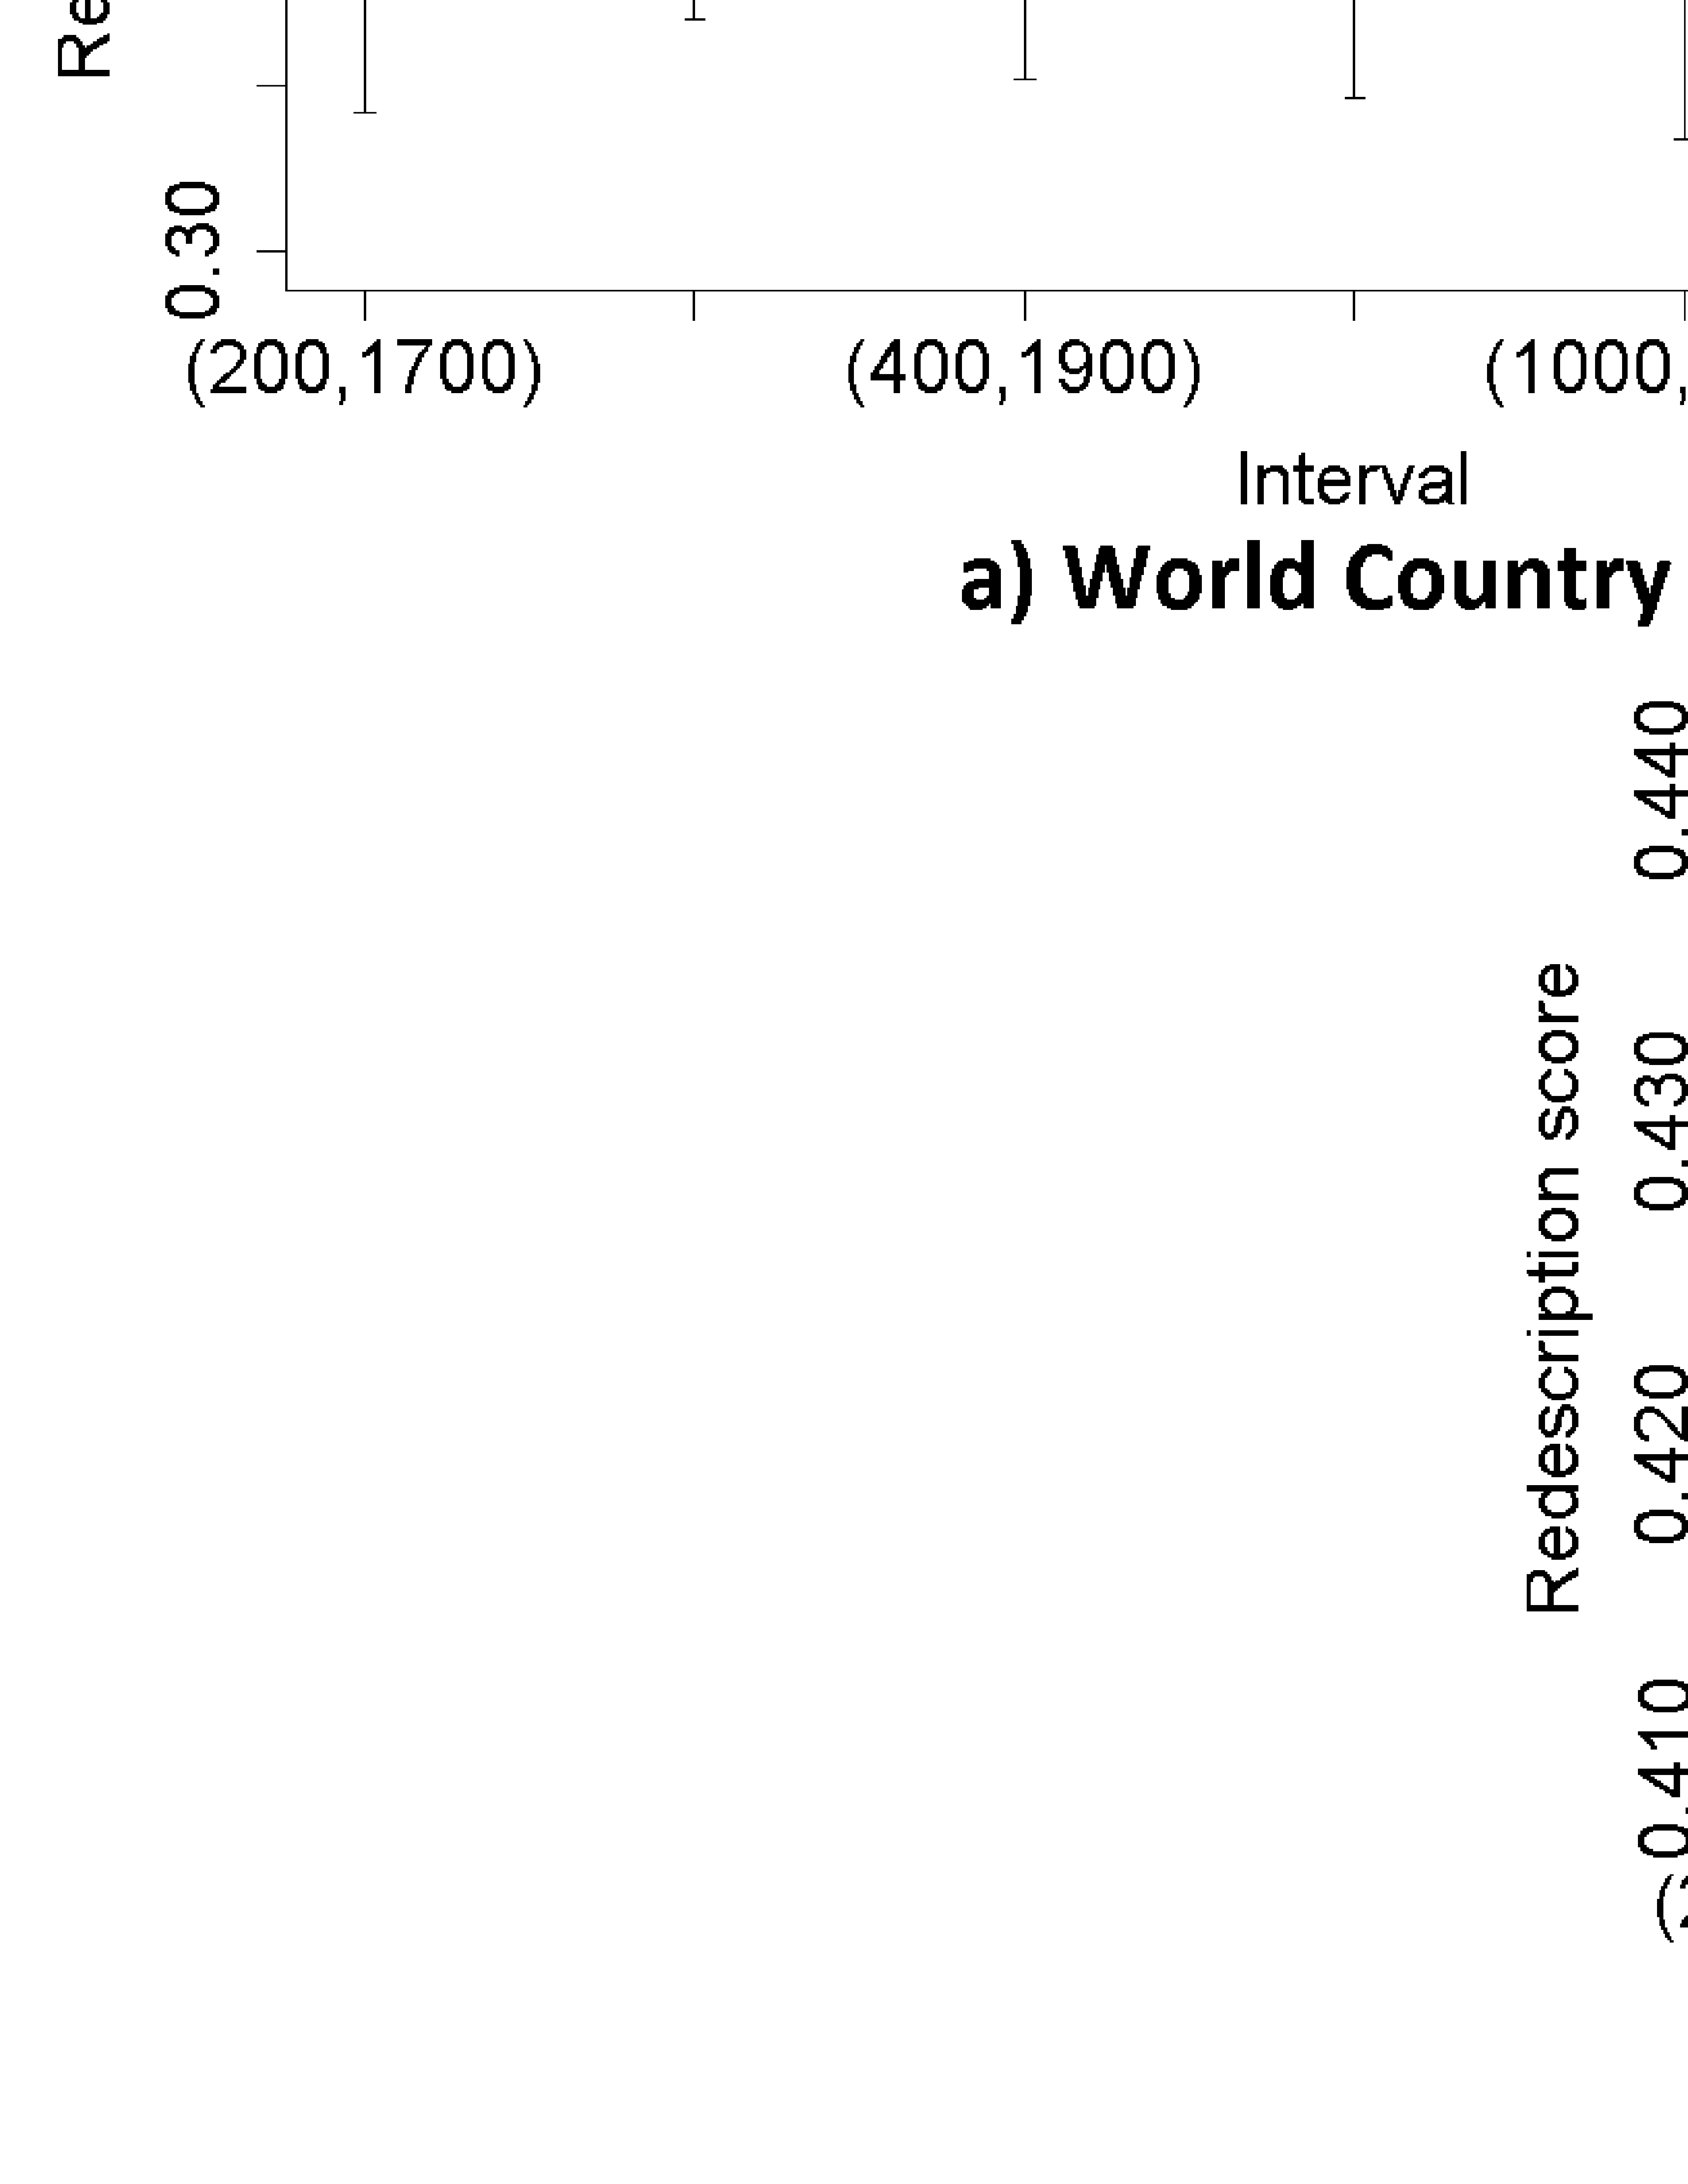}}
\caption{Overall score $\underline{total_{sc}}(\mathcal{R})$ obtained for the redescription set using a single rule-generating PCT model with different memory parameters.}
\label{fig:STRS}
\end{figure}

The results presented in Table \ref{tab:res1} show that the presented framework outperforms naive methods on the Country dataset (that allows creating large number of redescriptions) and it outperforms the naive methods on many measures even on the other two datasets (that allow creating very small number of highly accurate redescriptions). Results from Table \ref{tab:res1} and Figure \ref{fig:STRS} show that increasing the amount of memory allows obtaining redescription sets of higher quality. However, the difference in quality between the redescription set produced with the smallest memory setting ($200,\ 1700$) and the largest memory setting ($3000,\ 6000$) across $10$ runs is not significant, as computed by the one-sided Wilcoxon signed-rank test, for the Country ($p = 0.423$) and the Water ($p = 0.278 $) dataset but it is significant for the Phenotype dataset ($0.032$) with the significance level $0.05$. Increasing the amount of iterations used to create redescriptions mostly improves this result (see Figure $1$ from Supplementary document 1 and the corresponding significance analyses).  On two out of three datasets, the final memory setting (with the largest amount of memory) has the best overall redescription set score. The final redescription set score is very stable on the Slovenian Water and Phenotype datasets, but its standard deviation is significantly higher on the World Country dataset. The main reason for this is the inability of the framework to produce $200$ complete redescriptions for each of the $10$ different runs. This is also visible from different values of $RSS$ and \underline{$RSS$}. Increasing the number of iterations ($Iter.$) resolves this problem (see Figure $1$ from Supplementary document 1). The study of the execution time of the framework with various number of views is available in Section $2$ of Supplementary document $1$.

\begin{center}
\begin{footnotesize}
\LTcapwidth=\textwidth
\begin{longtable}[c]{|c|c|c|c|c|c|c|c|c|c|c|c|c|c|} % <-- Replaces
%\begin{table}[H]
%\footnotesize
\caption{Comparative results of a framework for multi-view redescription mining and naive implementations of multi-view redescription mining (NCLUS-RM, NReReMi) on three different datasets (C,W,P). Framework uses a single PCT model as a rule-generating model with different sizes of the working and maximal available memory. The $M$ column contains the name of the naive method or the memory configuration for the proposed framework.}%row -> measures, row+1->deviation
\label{tab:res1}\\
%\centering
%\begin{tabular}{ |c|c|c|c|c|c|c|c|c|c|c|c|c|c| }
\hline
$\mathcal{D}$ & $M$ & $AJ$ & $Ap_{sc}$ & $AEJ$ &$AAJ$ & $ARC$ & $RSS$& $\underline{AJ}$ & $\underline{Ap_{sc}}$ & $\underline{AEJ}$ & $\underline{AAJ}$ & $\underline{ARC}$ & $\underline{RSS}$ \\
\hline

\endfirsthead

\multicolumn{14}{c}%
        {{\textbf{ Table \thetable\ } Continued from previous page}} \\
        \hline

$\mathcal{D}$ & $M$ & $AJ$ & $Ap_{sc}$ & $AEJ$ &$AAJ$ & $ARC$ & $RSS$& $\underline{AJ}$ & $\underline{Ap_{sc}}$ & $\underline{AEJ}$ & $\underline{AAJ}$ & $\underline{ARC}$ & $\underline{RSS}$ \\
\hline

\endhead % <-- 
& NLUS-RM & $0.63$ & $0.43$ & $0.61$ & $\mathbf{0.08}$ & $0.77$ & $0.46$ & $0.58$ & $0.49$ & $0.66$ & $0.14$ & $0.79$ & $0.50$ \\
&  & $\mathbf{0.0}$ & $\mathbf{0.07}$ & $0.08$ & $\mathbf{0.01}$ & $0.08$ & $\mathbf{0.02}$ & $0.15$ & $\mathbf{0.14}$ & $0.10$ & $0.22$ & $0.09$ & $0.12$ \\
& NReReMi & $0.65$ & $0.74$ & $\mathbf{0.56}$ & $0.09$ & $0.82$ & $0.51$ & $0.65$ & $0.74$ & $\mathbf{0.56}$ & $\mathbf{0.09}$ & $0.82$ & $0.51$ \\
& $200$, $1700$ & $0.72$ & $0.25$ & $0.66$ & $0.20$ & $0.73$ & $0.42$ & $0.68$ & $0.29$ & $0.68$ & $0.25$ & $0.74$ & $0.46$ \\
&  & $0.03$ & $0.08$ & $0.07$ & $0.03$ & $0.08$ & $0.03$ & $0.14$ & $0.17$ & $0.09$ & $0.15$ & $0.09$ & $0.11$ \\
& $300$, $1800$ & $0.72$ & $0.27$ & $0.70$ & $0.20$ & $0.74$ & $0.44$ & $\mathbf{0.69}$ & $0.30$ & $0.69$ & $0.24$ & $0.75$ & $0.46$ \\
&  & $0.03$ & $0.09$ & $0.07$ & $0.04$ & $0.06$ & $0.02$ & $\mathbf{0.12}$ & $0.15$ & $\mathbf{0.08}$ & $\mathbf{0.12}$ & $\mathbf{0.07}$ & $\mathbf{0.09}$ \\
C & $400$, $1900$ & $\mathbf{0.73}$ & $0.28$ & $0.68$ & $0.21$ & $0.76$ & $0.44$ & $0.68$ & $0.32$ & $0.71$ & $0.26$ & $0.77$ & $0.48$ \\
&  & $0.03$ & $0.09$ & $0.08$ & $0.03$ & $0.05$ & $0.03$ & $0.16$ & $0.18$ & $0.10$ & $0.17$ & $0.08$ & $0.12$ \\
 & $500$, $2000$ & $0.73$ & $0.28$ & $0.67$ & $0.20$ & $0.76$ & $0.44$ & $0.68$ & $0.32$ & $0.69$ & $0.25$ & $0.73$ & $0.47$ \\
&  & $0.03$ & $0.08$ & $0.07$ & $0.03$ & $\mathbf{0.05}$ & $0.03$ & $0.16$ & $0.18$ & $0.09$ & $0.17$ & $0.07$ & $0.13$ \\
& $1000$, $4000$ & $0.72$ & $0.25$ & $0.69$ & $0.20$ & $0.71$ & $0.43$ & $0.67$ & $0.29$ & $0.71$ & $0.25$ & $0.73$& $0.46$\\
&  & $0.02$ & $0.09$ & $\mathbf{0.06}$ & $0.04$ & $0.06$ & $0.02$ & $0.16$ & $0.19$ & $0.09$ & $0.18$ & $0.09$& $0.13$ \\
& $2000$, $5000$ &  $0.72$ & $0.25$ & $0.67$ & $0.19$ & $0.71$ & $0.42$  & $0.67$ & $0.29$ & $0.69$ & $0.24$ &  $0.72$ & $0.46$\\
&  & $0.03$  & $0.08$ & $0.07$ & $0.03$ & $0.06$ & $0.03$  & $0.16$ & $0.19$ & $0.10$ & $0.18$ & $0.09$ & $0.13$\\
& $3000$, $6000$ & $0.72$ & $\mathbf{0.24}$ & $0.67$& $0.19$ & $\mathbf{0.70}$ &  $\mathbf{0.42}$ & $0.67$ & $\mathbf{0.29}$ & $0.69$ & $0.24$ & $\mathbf{0.71}$ & $\mathbf{0.45}$\\ 
& & $0.02$ & $0.10$ & $0.07$& $0.03$ & $0.06$ & $0.03$  & $0.15$ & $0.19$ & $0.09$ & $0.18$ & $0.09$ & $0.13$\\ \hline
& NCLUS-RM & $0.62$ & $\mathbf{0.56}$ & $\mathbf{0.51}$ & $\mathbf{0.16}$ & $0.60$ & $\mathbf{0.44}$ & $0.33$ & $\mathbf{0.79}$ & $0.74$ & $0.55$ & $0.79$ & $0.71$ \\
&  & $0.03$ & $0.11$ & $0.06$ & $\mathbf{0.03}$ & $\mathbf{0.04}$ & $\mathbf{0.02}$ & $0.11$ & $0.09$ & $0.08$ & $0.14$ & $0.07$ & $0.09$ \\
& NReReMi & $0.0$ & $1.0$ & $1.0$ & $1.0$ & $1.0$ & $1.0$ & $0.0$ & $1.0$ & $1.0$ & $1.0$ & $1.0$ & $1.0$ \\
& $200$, $1700$ & $0.68$ & $0.80$ & $0.64$ & $0.37$ & $0.57$ & $0.54$ & $0.68$ & $0.80$ & $\mathbf{0.64}$ & $\mathbf{0.37}$ & $0.57$ & $0.54$\\
&  & $0.02$ & $\mathbf{0.03}$ & $0.05$ & $0.07$ & $0.05$ & $0.03$ & $0.02$ & $\mathbf{0.03}$ & $0.05$ & $0.07$ & $\mathbf{0.05}$ & $\mathbf{0.03}$ \\
& $300$, $1800$ & $0.68$ & $0.80$ & $0.64$ & $0.38$ & $\mathbf{0.57}$ & $0.54$ & $0.68$ & $0.80$ & $0.64$ & $0.38$ & $\mathbf{0.57}$ & $0.54$ \\
& & $0.02$ & $0.04$ & $0.05$ & $0.07$ & $0.06$ & $0.03$ & $0.02$ & $0.04$ & $0.05$ & $0.07$ & $0.06$ & $0.03$ \\
W & $400$, $1900$ & $0.68$ & $0.80$ & $0.64$ & $0.38$ & $0.57$ & $0.54$ &$0.68$ & $0.80$ & $0.64$ & $0.38$ & $0.57$ & $\mathbf{0.54}$ \\
& &$0.02$ & $0.04$ & $0.05$ & $0.07$ & $0.06$ & $0.03$  & $0.02$ & $0.04$ & $0.05$ & $0.07$ & $0.06$ & $0.03$ \\
& $500$, $2000$ & $\mathbf{0.68}$ & $0.80$ & $0.64$ & $0.38$ & $0.57$ & $0.54$ &  $\mathbf{0.68}$ & $0.80$ & $0.64$ & $0.38$ & $0.57$ & $0.54$ \\
& & $\mathbf{0.02}$ & $0.04$ & $0.05$ & $0.07$ & $0.06$ &  $0.03$  &  $\mathbf{0.02}$ & $0.04$ & $0.05$ & $0.07$ & $0.06$ &  $0.03$ \\
& $1000$, $4000$ & $0.68$ & $0.80$ & $0.64$ & $0.38$ & $0.57$ & $0.54$  & $0.68$ & $0.80$ & $0.64$ & $0.38$ & $0.57$ & $0.54$\\ 
& & $0.02$ & $0.04$ & $\mathbf{0.05}$ & $0.07$ & $0.05$ & $0.03$ & $0.02$ & $0.04$ & $\mathbf{0.05}$ & $\mathbf{0.07}$ & $0.05$ & $0.03$\\
& $2000$, $5000$ & $0.68$ & $0.80$ & $0.64$ & $0.38$ & $0.57$ & $0.54$  &  $0.68$ & $0.80$ & $0.64$ & $0.38$ & $0.57$ & $0.54$ \\
& & $0.02$ & $0.04$ & $\mathbf{0.05}$ & $0.07$ & $0.05$ & $0.03$ & $0.02$ & $0.04$ & $\mathbf{0.05}$ & $\mathbf{0.07}$ & $0.05$ & $0.03$ \\
& $3000$, $6000$ & $0.68$ & $0.80$ & $0.64$ & $0.38$ & $0.57$ & $0.54$ & $0.68$ & $0.80$ & $0.64$ & $0.38$ & $0.57$ & $0.54$ \\
& & $0.02$ & $0.04$ & $\mathbf{0.05}$ & $0.07$ & $0.05$ & $0.03$ & $0.02$ & $0.04$ & $\mathbf{0.05}$ & $\mathbf{0.07}$ & $0.05$ & $0.03$ \\ \hline
& NCLUS-RM & $0.19$ & $0.78$ & $0.11$ & $\mathbf{0.02}$ & $0.64$ & $0.47$ & $0.19$ & $0.78$ & $0.11$ & $\mathbf{0.02}$ & $0.64$ & $0.47$ \\
&  & $\mathbf{0.01}$ & $\mathbf{0.01}$ & $\mathbf{0.01}$ & $\mathbf{0.0}$ & $0.05$ & $0.01$ & $\mathbf{0.01}$ & $\mathbf{0.01}$ & $\mathbf{0.01}$ & $\mathbf{0.0}$ & $0.05$ & $0.01$ \\
& NReReMi & $\mathbf{0.27}$ & $0.82$ & $0.27$ & $0.04$ & $\mathbf{0.31}$ & $0.43$ & $\mathbf{0.27}$ & $0.82$ & $0.27$ & $0.04$ & $\mathbf{0.31}$ & $0.43$ \\
& $200$, $1700$ & $0.20$ & $0.78$ & $0.10$ & $0.05$ & $0.40$ & $0.43$ & $0.20$ & $0.78$ & $0.10$ & $0.05$ & $0.40$ & $0.43$\\
& & $0.02$ & $0.02$ & $0.02$ & $0.01$ & $0.03$ & $0.01$ & $0.02$ & $0.02$ & $0.02$ & $0.01$ & $0.03$ & $0.01$ \\
& $300$, $1800$ & $0.20$ & $0.78$ & $0.10$ & $0.05$ & $0.40$ & $0.42$ & $0.20$ & $0.78$ & $0.10$ & $0.05$ & $0.40$ & $0.42$ \\
& & $0.02$ & $0.02$ & $0.02$& $0.01$ & $0.03$ & $0.01$  & $0.02$ & $0.02$ & $0.02$& $0.01$ & $0.03$ & $0.01$\\
P & $400$, $1900$ & $0.21$ & $0.78$ & $0.11$ & $0.05$ & $0.39$ & $0.42$ & $0.21$ & $0.78$ & $0.11$ & $0.05$ & $0.39$ & $0.42$\\
& & $0.03$ & $0.02$ & $0.01$ & $0.01$ & $0.01$ & $0.01$ &$0.03$ & $0.02$ & $0.01$ & $0.01$ & $0.01$ & $0.01$ \\
 & $500$, $2000$ & $0.20$ & $0.78$ & $0.10$ & $0.05$ & $0.40$ & $0.42$ &$0.20$ & $0.78$ & $0.10$ & $0.05$ & $0.40$ & $0.42$ \\
& & $0.02$ & $0.02$ & $0.01$ & $0.01$ & $\mathbf{0.02}$ & $0.01$ & $0.02$ & $0.02$ & $0.01$ & $0.01$ & $\mathbf{0.02}$ & $0.01$\\
& $1000$, $4000$ & $0.21$& $0.77$ & $\mathbf{0.10}$ & $0.04$ & $0.40$ & $0.42$ & $0.21$& $0.77$ & $\mathbf{0.10}$ & $0.04$ & $0.40$ & $0.42$ \\
& & $0.03$& $0.02$ & $0.01$ & $0.01$ & $0.02$ & $\mathbf{0.01}$ & $0.03$& $0.02$ & $0.01$ & $0.01$ & $0.02$ & $\mathbf{0.01}$ \\
& $2000$, $5000$ & $0.21$ & $0.77$ & $0.10$ & $0.04$ & $0.40$ & $0.42$  &$0.21$ & $0.77$ & $0.10$ & $0.04$ & $0.40$ & $0.42$\\
& & $0.03$ & $0.02$ & $0.01$ & $0.01$ & $0.02$ & $0.01$  & $0.03$ & $0.02$ & $0.01$ & $0.01$ & $0.02$ & $0.01$\\
& $3000$, $6000$ & $0.21$ & $\mathbf{0.77}$ & $0.10$ & $0.04$ & $0.40$ & $\mathbf{0.42}$  & $0.21$ & $\mathbf{0.77}$ & $0.10$ & $0.04$ & $0.40$ & $\mathbf{0.42}$\\ 
& & $0.03$ & $0.02$ & $0.01$ & $0.01$ & $0.03$ & $0.01$  & $0.03$ & $0.02$ & $0.01$ & $0.01$ & $0.03$ & $0.01$\\\hline
%\end{tabular}
%\end{table} 
\end{longtable}
\end{footnotesize}
\end{center}

\subsection{Using Random Forest of supplementing models}

We evaluate the effects of using a Random Forest of supplementing models on the quality of the produced redescription set. We use different redescription set evaluation measures and denote in boldface the best performing method for each memory interval. We test the performance when using Random attribute subspace selection with Predictive Clustering trees \cite{KocevSO}, Random Forest of Predictive Clustering trees with random output selections \cite{BreskvarROS} and using Random Forest of Extra trees \cite{KocevET}.

\begin{center}
\begin{footnotesize}
\LTcapwidth=\textwidth
\begin{longtable}[c]{|c|c|c|c|c|c|c|c|c|c|c|c|c|c|} % <-- Replaces \begin{table}, alignment must be 
 \caption{Quality of redescription sets produced on the World Country dataset using the framework for multi-view redescription mining with a Random Forest supplementing model containing $50$ trees, given different memory sizes (work size, maximal memory size).}
  \label{tab:Supp1}\\
 \hline
 $M$ & $\mathcal{M}$ & $AJ$ & $Ap_{sc}$ & $AEJ$ &$AAJ$ & $ARC$ & $RSS$& $\underline{AJ}$ & $\underline{Ap_{sc}}$ & $\underline{AEJ}$ & $\underline{AAJ}$ & $\underline{ARC}$ & $\underline{RSS}$ \\  \hline
 
 \endfirsthead

\multicolumn{14}{c}%
        {{\textbf{ Table \thetable\ } Continued from previous page}} \\
        \hline
        
   $M$ & $\mathcal{M}$ & $AJ$ & $Ap_{sc}$ & $AEJ$ &$AAJ$ & $ARC$ & $RSS$& $\underline{AJ}$ & $\underline{Ap_{sc}}$ & $\underline{AEJ}$ & $\underline{AAJ}$ & $\underline{ARC}$ & $\underline{RSS}$ \\  \hline      

  \endhead % <--  
& $PCT$ &$0.71$ & $0.39$ & $0.79$ & $0.35$ & $\mathbf{0.62}$ &$0.49$ & $0.32$ & $0.7$ & $0.9$ & $0.68$ & $0.82$ & $0.76$\\
& & $0.04$ & $0.15$ & $0.1$ & $0.13$ & $0.05$ & $0.04$ & $0.23$ & $0.27$ & $0.1$ & $0.24$ & $0.13$ & $0.19$\\
& $PCT_{Sub}$ &$0.75$ & $0.32$ & $0.73$ & $\mathbf{0.11}$ &$0.71$ & $\mathbf{0.42}$ &$0.75$ & $0.32$ & $0.73$ & $\mathbf{0.11}$ &$\mathbf{0.71}$ &$\mathbf{0.42}$\\
\parbox[t]{2mm}{\multirow{2}{*}{\rotatebox[origin=c]{90}{$200$, $1700$}}}& & $0.02$ & $\mathbf{0.11}$ &$0.07$ & $\mathbf{0.01}$ &$0.07$ & $0.02$ & $\mathbf{0.02}$ &$\mathbf{0.11}$ &$\mathbf{0.07}$ &$\mathbf{0.01}$ &$0.07$ & $0.02$\\
& $PCT_{ET}$ &$0.74$ & $0.38$ & $0.77$ & $0.17$ & $0.74$ & $0.47$ & $0.69$ & $0.41$ & $0.78$ & $0.22$ & $0.76$ & $0.5$\\
& & $\mathbf{0.01}$ &$0.16$ & $\mathbf{0.06}$ &$0.04$ & $\mathbf{0.04}$ &$0.03$ & $0.14$ & $0.2$ & $0.07$ & $0.17$ & $\mathbf{0.07}$ &$0.11$\\
& $PCT_{ROS}$ &$\mathbf{0.76}$ &$\mathbf{0.31}$ &$\mathbf{0.71}$ &$0.12$ & $0.74$ & $0.43$ & $\mathbf{0.76}$ &$\mathbf{0.31}$ &$\mathbf{0.71}$ &$0.12$ & $0.74$ & $0.43$\\
& & $0.02$ & $0.12$ & $0.08$ & $0.02$ & $0.08$ & $\mathbf{0.02}$ &$0.02$ & $0.12$ & $0.08$ & $0.02$ & $0.08$ & $\mathbf{0.02}$\\\hline
& $PCT$ &$0.7$ & $0.39$ & $0.79$ & $0.36$ & $\mathbf{0.62}$ &$0.49$ & $0.34$ & $0.69$ & $0.9$ & $0.67$ & $0.82$ & $0.75$\\
& & $0.04$ & $0.14$ & $0.1$ & $0.13$ & $\mathbf{0.05}$ &$0.05$ & $0.24$ & $0.28$ & $0.11$ & $0.25$ & $0.12$ & $0.19$\\
& $PCT_{Sub}$ &$0.75$ & $\mathbf{0.31}$ &$0.75$ & $\mathbf{0.12}$ &$0.72$ & $0.43$ & $0.75$ & $\mathbf{0.31}$ &$0.75$ & $\mathbf{0.12}$ &$\mathbf{0.72}$ &$0.43$\\
\parbox[t]{2mm}{\multirow{2}{*}{\rotatebox[origin=c]{90}{$300$, $1800$}}}& & $0.02$ & $0.15$ & $0.08$ & $\mathbf{0.02}$ &$0.08$ & $0.02$ & $0.02$ & $0.15$ & $\mathbf{0.08}$ &$\mathbf{0.02}$ &$0.08$ & $0.02$\\
& $PCT_{ET}$ &$0.74$ & $0.37$ & $0.76$ & $0.17$ & $0.76$ & $0.46$ & $0.7$ & $0.4$ & $0.78$ & $0.21$ & $0.77$ & $0.49$\\
& & $0.02$ & $0.15$ & $\mathbf{0.08}$ &$0.03$ & $0.05$ & $0.03$ & $0.14$ & $0.2$ & $0.09$ & $0.17$ & $\mathbf{0.07}$ &$0.11$\\
& $PCT_{ROS}$ &$\mathbf{0.76}$ &$0.32$ & $\mathbf{0.7}$ &$0.12$ & $0.74$ & $\mathbf{0.42}$ &$\mathbf{0.76}$ &$0.32$ & $\mathbf{0.7}$ &$0.12$ & $0.74$ & $\mathbf{0.42}$\\
& & $\mathbf{0.02}$ &$\mathbf{0.11}$ &$0.09$ & $0.02$ & $0.07$ & $\mathbf{0.02}$ &$\mathbf{0.02}$ &$\mathbf{0.11}$ &$0.09$ & $0.02$ & $0.07$ & $\mathbf{0.02}$\\\hline
& $PCT$ &$0.7$ & $0.39$ & $0.79$ & $0.35$ & $\mathbf{0.62}$ &$0.49$ & $0.35$ & $0.68$ & $0.89$ & $0.65$ & $0.81$ & $0.74$\\
& & $0.04$ & $0.15$ & $0.1$ & $0.14$ & $0.07$ & $0.05$ & $0.24$ & $0.29$ & $0.11$ & $0.26$ & $0.14$ & $0.2$\\
& $PCT_{Sub}$ &$0.75$ & $\mathbf{0.29}$ &$0.75$ & $0.12$ & $0.72$ & $\mathbf{0.43}$ &$0.75$ & $\mathbf{0.29}$ &$0.75$ & $0.12$ & $\mathbf{0.72}$ &$\mathbf{0.43}$\\
\parbox[t]{2mm}{\multirow{2}{*}{\rotatebox[origin=c]{90}{$400$, $1900$}}}& & $0.02$ & $0.16$ & $\mathbf{0.07}$ &$0.03$ & $0.09$ & $0.02$ & $0.02$ & $0.16$ & $\mathbf{0.07}$ &$0.03$ & $0.09$ & $0.02$\\
& $PCT_{ET}$ &$0.74$ & $0.37$ & $0.77$ & $0.16$ & $0.75$ & $0.46$ & $0.7$ & $0.4$ & $0.78$ & $0.21$ & $0.76$ & $0.49$\\
& & $\mathbf{0.01}$ &$0.15$ & $0.07$ & $0.02$ & $\mathbf{0.05}$ &$0.03$ & $0.13$ & $0.2$ & $0.08$ & $0.15$ & $\mathbf{0.07}$ &$0.1$\\
& $PCT_{ROS}$ &$\mathbf{0.76}$ &$0.32$ & $\mathbf{0.7}$ &$\mathbf{0.12}$ &$0.76$ & $0.43$ & $\mathbf{0.76}$ &$0.32$ & $\mathbf{0.7}$ &$\mathbf{0.12}$ &$0.76$ & $0.43$\\
& & $0.02$ & $\mathbf{0.12}$ &$0.08$ & $\mathbf{0.02}$ &$0.07$ & $\mathbf{0.02}$ &$\mathbf{0.02}$ &$\mathbf{0.12}$ &$0.08$ & $\mathbf{0.02}$ &$0.07$ & $\mathbf{0.02}$\\\hline
& $PCT$ &$0.7$ & $0.39$ & $0.79$ & $0.34$ & $\mathbf{0.62}$ &$0.49$ & $0.35$ & $0.69$ & $0.89$ & $0.65$ & $0.81$ & $0.74$\\
& & $0.04$ & $0.15$ & $0.1$ & $0.14$ & $0.07$ & $0.05$ & $0.25$ & $0.28$ & $0.1$ & $0.26$ & $0.14$ & $0.2$\\
& $PCT_{Sub}$ &$0.75$ & $\mathbf{0.31}$ &$0.75$ & $0.12$ & $0.72$ & $0.43$ & $0.75$ & $\mathbf{0.31}$ &$0.75$ & $0.12$ & $\mathbf{0.72}$ &$0.43$\\
\parbox[t]{2mm}{\multirow{2}{*}{\rotatebox[origin=c]{90}{$500$, $2000$}}}& & $\mathbf{0.01}$ &$0.15$ & $\mathbf{0.07}$ &$0.03$ & $0.09$ & $0.02$ & $\mathbf{0.01}$ &$0.15$ & $\mathbf{0.07}$ &$0.03$ & $0.09$ & $0.02$\\
& $PCT_{ET}$ &$0.75$ & $0.37$ & $0.76$ & $0.16$ & $0.76$ & $0.46$ & $0.71$ & $0.39$ & $0.78$ & $0.21$ & $0.78$ & $0.49$\\
& & $0.02$ & $0.15$ & $0.07$ & $0.02$ & $\mathbf{0.06}$ &$0.03$ & $0.13$ & $0.19$ & $0.08$ & $0.15$ & $\mathbf{0.07}$ &$0.1$\\
& $PCT_{ROS}$ &$\mathbf{0.76}$ &$0.33$ & $\mathbf{0.71}$ &$\mathbf{0.11}$ &$0.75$ & $\mathbf{0.43}$ &$\mathbf{0.76}$ &$0.33$ & $\mathbf{0.71}$ &$\mathbf{0.11}$ &$0.75$ & $\mathbf{0.43}$\\
& & $0.02$ & $\mathbf{0.11}$ &$0.08$ & $\mathbf{0.02}$ &$0.08$ & $\mathbf{0.02}$ &$0.02$ & $\mathbf{0.11}$ &$0.08$ & $\mathbf{0.02}$ &$0.08$ & $\mathbf{0.02}$\\\hline
& $PCT$ &$0.7$ & $0.39$ & $0.79$ & $0.34$ & $\mathbf{0.61}$ &$0.49$ & $0.34$ & $0.69$ & $0.89$ & $0.65$ & $0.81$ & $0.74$\\
& & $0.04$ & $0.15$ & $0.09$ & $0.14$ & $0.07$ & $0.05$ & $0.24$ & $0.28$ & $0.1$ & $0.26$ & $0.14$ & $0.2$\\
& $PCT_{Sub}$ &$\mathbf{0.75}$ &$0.3$ & $0.76$ & $0.12$ & $0.71$ & $0.43$ & $\mathbf{0.75}$ &$0.3$ & $0.76$ & $0.12$ & $\mathbf{0.71}$ &$0.43$\\
\parbox[t]{2mm}{\multirow{2}{*}{\rotatebox[origin=c]{90}{$1000$, $4000$}}}& & $0.02$ & $0.13$ & $\mathbf{0.06}$ &$\mathbf{0.02}$ &$0.08$ & $\mathbf{0.02}$ &$\mathbf{0.02}$ &$\mathbf{0.13}$ &$\mathbf{0.06}$ &$\mathbf{0.02}$ &$0.08$ & $\mathbf{0.02}$\\
& $PCT_{ET}$ &$0.75$ & $0.36$ & $0.75$ & $0.15$ & $0.75$ & $0.45$ & $0.71$ & $0.38$ & $0.77$ & $0.19$ & $0.76$ & $0.48$\\
& & $\mathbf{0.01}$ &$\mathbf{0.1}$ &$0.09$ & $0.02$ & $\mathbf{0.07}$ &$0.03$ & $0.12$ & $0.16$ & $0.09$ & $0.14$ & $\mathbf{0.08}$ &$0.09$\\
& $PCT_{ROS}$ &$0.75$ & $\mathbf{0.28}$ &$\mathbf{0.72}$ &$\mathbf{0.11}$ &$0.72$ & $\mathbf{0.42}$ &$0.75$ & $\mathbf{0.28}$ &$\mathbf{0.72}$ &$\mathbf{0.11}$ &$0.72$ & $\mathbf{0.42}$\\
& & $0.02$ & $0.13$ & $0.08$ & $0.02$ & $0.1$ & $0.02$ & $0.02$ & $0.13$ & $0.08$ & $0.02$ & $0.1$ & $0.02$\\\hline
& $PCT$ &$0.7$ & $0.4$ & $\mathbf{0.73}$ &$0.32$ & $\mathbf{0.59}$ &$0.47$ & $0.32$ & $0.7$ & $0.9$ & $0.67$ & $0.82$ & $0.75$\\
& & $0.05$ & $0.16$ & $0.27$ & $0.18$ & $0.08$ & $0.08$ & $0.27$ & $0.3$ & $0.11$ & $0.29$ & $0.15$ & $0.22$\\
& $PCT_{Sub}$ &$\mathbf{0.75}$ &$\mathbf{0.26}$ &$0.76$ & $0.12$ & $0.71$ & $0.42$ & $\mathbf{0.75}$ &$\mathbf{0.26}$ &$0.76$ & $0.12$ & $0.71$ & $0.42$\\
\parbox[t]{2mm}{\multirow{2}{*}{\rotatebox[origin=c]{90}{$2000$, $5000$}}}& & $0.02$ & $0.14$ & $\mathbf{0.06}$ &$\mathbf{0.02}$ &$0.1$ & $0.02$ & $0.02$ & $0.14$ & $\mathbf{0.06}$ &$\mathbf{0.02}$ &$0.1$ & $0.02$\\
& $PCT_{ET}$ &$0.75$ & $0.34$ & $0.76$ & $0.15$ & $0.73$ & $0.45$ & $0.75$ & $0.34$ & $0.76$ & $0.15$ & $0.73$ & $0.45$\\
& & $\mathbf{0.01}$ &$\mathbf{0.12}$ &$0.09$ & $0.02$ & $0.07$ & $0.02$ & $\mathbf{0.01}$ &$\mathbf{0.12}$ &$0.09$ & $0.02$ & $0.07$ & $0.02$\\
& $PCT_{ROS}$ &$0.75$ & $0.28$ & $0.73$ & $\mathbf{0.11}$ &$0.7$ & $\mathbf{0.42}$ &$0.75$ & $0.28$ & $\mathbf{0.73}$ &$\mathbf{0.11}$ &$\mathbf{0.7}$ &$\mathbf{0.42}$\\
& & $0.02$ & $0.14$ & $0.07$ & $0.03$ & $\mathbf{0.07}$ &$\mathbf{0.02}$ &$0.02$ & $0.14$ & $0.07$ & $0.03$ & $\mathbf{0.07}$ &$\mathbf{0.02}$\\\hline
& $PCT$ &$0.7$ & $0.4$ & $0.73$ & $0.32$ & $\mathbf{0.59}$ &$0.47$ & $0.32$ & $0.7$ & $0.9$ & $0.67$ & $0.82$ & $0.75$\\
& & $0.05$ & $0.16$ & $0.27$ & $0.18$ & $0.08$ & $0.08$ & $0.27$ & $0.3$ & $0.11$ & $0.29$ & $0.15$ & $0.22$\\
& $PCT_{Sub}$ &$0.74$ & $\mathbf{0.25}$ &$0.76$ & $0.12$ & $0.69$ & $\mathbf{0.41}$ &$0.74$ & $\mathbf{0.25}$ &$0.76$ & $0.12$ & $\mathbf{0.69}$ &$\mathbf{0.41}$\\
\parbox[t]{2mm}{\multirow{2}{*}{\rotatebox[origin=c]{90}{$3000$, $6000$}}}& & $0.02$ & $0.16$ & $\mathbf{0.07}$ &$\mathbf{0.02}$ &$0.09$ & $\mathbf{0.02}$ &$0.02$ & $0.16$ & $\mathbf{0.07}$ &$\mathbf{0.02}$ &$0.09$ & $\mathbf{0.02}$\\
& $PCT_{ET}$ &$\mathbf{0.75}$ &$0.34$ & $0.75$ & $0.15$ & $0.73$ & $0.44$ & $\mathbf{0.75}$ &$0.34$ & $0.75$ & $0.15$ & $0.73$ & $0.44$\\
& & $\mathbf{0.01}$ &$\mathbf{0.12}$ &$0.09$ & $0.02$ & $\mathbf{0.06}$ &$0.02$ & $\mathbf{0.01}$ &$\mathbf{0.12}$ &$0.09$ & $0.02$ & $\mathbf{0.06}$ &$0.02$\\
& $PCT_{ROS}$ &$0.75$ & $0.28$ & $\mathbf{0.72}$ &$\mathbf{0.11}$ &$0.71$ & $0.42$ & $0.75$ & $0.28$ & $\mathbf{0.72}$ &$\mathbf{0.11}$ &$0.71$ & $0.42$\\
& & $0.02$ & $0.13$ & $0.08$ & $0.03$ & $0.09$ & $0.02$ & $0.02$ & $0.13$ & $0.08$ & $0.03$ & $0.09$ & $0.02$\\\hline
\end{longtable}
\end{footnotesize}
\end{center}

The results obtained on the World Country dataset, presented in Table \ref{tab:Supp1} show that the framework for multi-view redescription mining with a Random Forest using random attribute subspaces (Sub) and random output (target) selections (ROS) supplementing models achieves the best performance. On smaller and medium memory size parameters, the framework with Sub achieves best performance in attribute diversity, occasionally significance score and overall redescription set score, while the framework with ROS achieves best performance in redescription accuracy, entity diversity and occasionally significance score. Using larger memory parameters allows the framework with Extra multi-target PCT to achieve competitive accuracy score but the overall best performance is divided between the Sub and the ROS. 

The results on the Slovenian Water quality dataset (see Table \ref{tab:Supp2}) show that using a single PCT model has the best performance on many different redescription set quality measures, however this is the artefact that occurs due to very small number of produced redescriptions (visible in the large standard deviation for this approach). The $\underline{underline}$ scores show the true difference between the approaches. Supplementing models create a much larger number of redescriptions and the quality of the finally produced redescription set is almost twice better. When using smaller amount of memory, our framework with the Sub and the ROS supplementing models achieves the best performance, but using a larger amount of memory allows the framework with the Extra multi-target PCTs to outperform the other approaches.

\begin{center}
\begin{footnotesize}
\LTcapwidth=\textwidth
\begin{longtable}[c]{|c|c|c|c|c|c|c|c|c|c|c|c|c|c|} % <-- Replaces \begin{table}, alignment must be 
 \caption{Quality of redescription sets produced on the Slovenian Water dataset using the framework for multi-view redescription mining with a Random Forest supplementing model containing $50$ trees, given different memory sizes (work size, maximal memory size).}
  \label{tab:Supp2}\\
 \hline
 $M$ & $\mathcal{M}$ & $AJ$ & $Ap_{sc}$ & $AEJ$ &$AAJ$ & $ARC$ & $RSS$& $\underline{AJ}$ & $\underline{Ap_{sc}}$ & $\underline{AEJ}$ & $\underline{AAJ}$ & $\underline{ARC}$ & $\underline{RSS}$ \\  \hline
 
  \endfirsthead

\multicolumn{14}{c}%
        {{\textbf{ Table \thetable\ } Continued from previous page}} \\
        \hline
        
 $M$ & $\mathcal{M}$ & $AJ$ & $Ap_{sc}$ & $AEJ$ &$AAJ$ & $ARC$ & $RSS$& $\underline{AJ}$ & $\underline{Ap_{sc}}$ & $\underline{AEJ}$ & $\underline{AAJ}$ & $\underline{ARC}$ & $\underline{RSS}$ \\  \hline 

  \endhead % <--  
& $PCT$ &$0.61$ & $\mathbf{0.67}$ &$\mathbf{0.63}$ &$0.46$ & $\mathbf{0.52}$ &$0.53$ & $0.11$ & $0.95$ & $0.96$ & $0.92$ & $0.92$ & $0.93$\\
& & $0.22$ & $0.26$ & $0.35$ & $0.26$ & $0.21$ & $0.16$ & $0.15$ & $0.05$ & $0.06$ & $0.11$ & $0.08$ & $0.09$\\
& $PCT_{Sub}$ &$0.69$ & $0.8$ & $0.67$ & $\mathbf{0.34}$ &$0.52$ & $\mathbf{0.53}$ &$0.66$ & $0.81$ & $\mathbf{0.69}$ &$\mathbf{0.36}$ &$\mathbf{0.54}$ &$\mathbf{0.55}$\\
\parbox[t]{2mm}{\multirow{2}{*}{\rotatebox[origin=c]{90}{$200$, $1700$}}}& & $0.02$ & $\mathbf{0.02}$ &$0.04$ & $0.06$ & $\mathbf{0.03}$ &$\mathbf{0.02}$ &$0.1$ & $\mathbf{0.03}$ &$0.05$ & $0.11$ & $0.07$ & $0.07$\\
& $PCT_{ET}$ &$0.66$ & $0.76$ & $0.73$ & $0.37$ & $0.56$ & $0.55$ & $0.58$ & $0.79$ & $0.76$ & $0.44$ & $0.61$ & $0.6$\\
& & $\mathbf{0.01}$ &$0.05$ & $0.04$ & $0.09$ & $0.07$ & $0.03$ & $0.19$ & $0.08$ & $0.09$ & $0.21$ & $0.15$ & $0.14$\\
& $PCT_{ROS}$ &$\mathbf{0.69}$ &$0.76$ & $0.69$ & $0.35$ & $0.6$ & $0.54$ & $\mathbf{0.67}$ &$\mathbf{0.77}$ &$0.7$ & $0.37$ & $0.61$ & $0.55$\\
& & $0.02$ & $0.03$ & $\mathbf{0.04}$ &$\mathbf{0.05}$ &$0.06$ & $0.03$ & $\mathbf{0.07}$ &$0.04$ & $\mathbf{0.05}$ &$\mathbf{0.09}$ &$\mathbf{0.07}$ &$\mathbf{0.06}$\\\hline
& $PCT$ &$0.61$ & $\mathbf{0.67}$ &$\mathbf{0.63}$ &$0.46$ & $\mathbf{0.52}$ &$0.53$ & $0.11$ & $0.95$ & $0.96$ & $0.92$ & $0.92$ & $0.93$\\
& & $0.22$ & $0.26$ & $0.35$ & $0.26$ & $0.21$ & $0.16$ & $0.15$ & $0.05$ & $0.06$ & $0.11$ & $0.08$ & $0.09$\\
& $PCT_{Sub}$ &$0.69$ & $0.8$ & $0.67$ & $\mathbf{0.33}$ &$0.52$ & $\mathbf{0.53}$ &$0.66$ & $0.81$ & $\mathbf{0.69}$ &$\mathbf{0.35}$ &$\mathbf{0.53}$ &$\mathbf{0.54}$\\
\parbox[t]{2mm}{\multirow{2}{*}{\rotatebox[origin=c]{90}{$300$, $1800$}}}& & $0.02$ & $\mathbf{0.02}$ &$0.04$ & $\mathbf{0.06}$ &$\mathbf{0.03}$ &$\mathbf{0.02}$ &$0.1$ & $\mathbf{0.03}$ &$0.05$ & $0.11$ & $\mathbf{0.07}$ &$0.07$\\
& $PCT_{ET}$ &$0.66$ & $0.76$ & $0.73$ & $0.37$ & $0.55$ & $0.55$ & $0.57$ & $0.79$ & $0.76$ & $0.44$ & $0.6$ & $0.6$\\
& & $\mathbf{0.02}$ &$0.05$ & $0.04$ & $0.09$ & $0.08$ & $0.04$ & $0.19$ & $0.08$ & $0.09$ & $0.21$ & $0.16$ & $0.14$\\
& $PCT_{ROS}$ &$\mathbf{0.69}$ &$0.77$ & $0.69$ & $0.35$ & $0.6$ & $0.54$ & $\mathbf{0.67}$ &$\mathbf{0.77}$ &$0.7$ & $0.36$ & $0.61$ & $0.55$\\
& & $0.02$ & $0.03$ & $\mathbf{0.04}$ &$0.06$ & $0.06$ & $0.03$ & $\mathbf{0.07}$ &$0.04$ & $\mathbf{0.05}$ &$\mathbf{0.09}$ &$0.08$ & $\mathbf{0.06}$\\\hline
& $PCT$ &$0.61$ & $\mathbf{0.67}$ &$\mathbf{0.63}$ &$0.46$ & $\mathbf{0.52}$ &$0.53$ & $0.11$ & $0.95$ & $0.96$ & $0.92$ & $0.92$ & $0.93$\\
& & $0.22$ & $0.26$ & $0.35$ & $0.26$ & $0.21$ & $0.16$ & $0.15$ & $0.05$ & $0.06$ & $0.11$ & $0.08$ & $0.09$\\
& $PCT_{Sub}$ &$\mathbf{0.69}$ &$0.8$ & $0.67$ & $\mathbf{0.33}$ &$0.52$ & $\mathbf{0.52}$ &$\mathbf{0.67}$ &$0.8$ & $\mathbf{0.68}$ &$\mathbf{0.34}$ &$\mathbf{0.53}$ &$\mathbf{0.54}$\\
\parbox[t]{2mm}{\multirow{2}{*}{\rotatebox[origin=c]{90}{$400$, $1900$}}}& & $0.02$ & $\mathbf{0.02}$ &$\mathbf{0.03}$ &$\mathbf{0.06}$ &$\mathbf{0.03}$ &$\mathbf{0.02}$ &$0.08$ & $\mathbf{0.03}$ &$\mathbf{0.04}$ &$0.1$ & $\mathbf{0.07}$ &$0.06$\\
& $PCT_{ET}$ &$0.66$ & $0.76$ & $0.73$ & $0.38$ & $0.56$ & $0.55$ & $0.57$ & $0.79$ & $0.76$ & $0.44$ & $0.61$ & $0.61$\\
& & $\mathbf{0.01}$ &$0.05$ & $0.05$ & $0.09$ & $0.08$ & $0.04$ & $0.19$ & $0.08$ & $0.09$ & $0.22$ & $0.16$ & $0.14$\\
& $PCT_{ROS}$ &$0.69$ & $0.76$ & $0.69$ & $0.34$ & $0.58$ & $0.54$ & $0.67$ & $\mathbf{0.76}$ &$0.7$ & $0.36$ & $0.59$ & $0.55$\\
& & $0.02$ & $0.04$ & $0.04$ & $0.06$ & $0.07$ & $0.03$ & $\mathbf{0.07}$ &$0.05$ & $0.04$ & $\mathbf{0.09}$ &$0.08$ & $\mathbf{0.06}$\\\hline
& $PCT$ &$0.61$ & $\mathbf{0.67}$ &$\mathbf{0.63}$ &$0.46$ & $0.52$ & $0.53$ & $0.11$ & $0.95$ & $0.96$ & $0.92$ & $0.92$ & $0.93$\\
& & $0.22$ & $0.26$ & $0.35$ & $0.26$ & $0.21$ & $0.16$ & $0.15$ & $0.05$ & $0.06$ & $0.11$ & $0.08$ & $0.09$\\
& $PCT_{Sub}$ &$0.69$ & $0.8$ & $0.67$ & $\mathbf{0.33}$ &$\mathbf{0.52}$ &$\mathbf{0.53}$ &$\mathbf{0.67}$ &$0.8$ & $\mathbf{0.68}$ &$\mathbf{0.34}$ &$\mathbf{0.53}$ &$\mathbf{0.54}$\\
\parbox[t]{2mm}{\multirow{2}{*}{\rotatebox[origin=c]{90}{$500$, $2000$}}}& & $0.02$ & $\mathbf{0.02}$ &$\mathbf{0.04}$ &$\mathbf{0.05}$ &$\mathbf{0.03}$ &$\mathbf{0.02}$ &$0.07$ & $\mathbf{0.03}$ &$\mathbf{0.04}$ &$\mathbf{0.09}$ &$\mathbf{0.05}$ &$\mathbf{0.05}$\\
& $PCT_{ET}$ &$0.66$ & $0.76$ & $0.73$ & $0.38$ & $0.56$ & $0.55$ & $0.57$ & $0.79$ & $0.76$ & $0.44$ & $0.61$ & $0.61$\\
& & $0.02$ & $0.05$ & $0.05$ & $0.09$ & $0.07$ & $0.04$ & $0.2$ & $0.08$ & $0.09$ & $0.21$ & $0.15$ & $0.14$\\
& $PCT_{ROS}$ &$\mathbf{0.69}$ &$0.76$ & $0.69$ & $0.34$ & $0.59$ & $0.54$ & $0.67$ & $\mathbf{0.77}$ &$0.7$ & $0.36$ & $0.59$ & $0.55$\\
& & $\mathbf{0.02}$ &$0.04$ & $0.04$ & $0.06$ & $0.06$ & $0.03$ & $\mathbf{0.07}$ &$0.05$ & $0.04$ & $0.09$ & $0.08$ & $0.06$\\\hline
& $PCT$ &$0.61$ & $\mathbf{0.67}$ &$\mathbf{0.63}$ &$0.46$ & $0.52$ & $0.53$ & $0.11$ & $0.95$ & $0.96$ & $0.92$ & $0.92$ & $0.93$\\
& & $0.22$ & $0.26$ & $0.35$ & $0.26$ & $0.21$ & $0.16$ & $0.15$ & $0.05$ & $0.06$ & $0.11$ & $0.08$ & $0.09$\\
& $PCT_{Sub}$ &$\mathbf{0.69}$ &$0.8$ & $0.67$ & $0.32$ & $0.52$ & $0.52$ & $0.67$ & $0.81$ & $\mathbf{0.68}$ &$0.34$ & $0.53$ & $0.54$\\
\parbox[t]{2mm}{\multirow{2}{*}{\rotatebox[origin=c]{90}{$1000$, $4000$}}}& & $0.02$ & $\mathbf{0.02}$ &$0.04$ & $0.05$ & $\mathbf{0.03}$ &$0.02$ & $0.09$ & $\mathbf{0.03}$ &$0.05$ & $0.11$ & $0.07$ & $0.06$\\
& $PCT_{ET}$ &$0.67$ & $0.76$ & $0.72$ & $\mathbf{0.3}$ &$\mathbf{0.47}$ &$\mathbf{0.51}$ &$\mathbf{0.67}$ &$\mathbf{0.76}$ &$0.72$ & $\mathbf{0.3}$ &$\mathbf{0.47}$ &$\mathbf{0.51}$\\
& & $\mathbf{0.01}$ &$0.03$ & $\mathbf{0.04}$ &$\mathbf{0.03}$ &$0.04$ & $\mathbf{0.02}$ &$\mathbf{0.01}$ &$0.03$ & $\mathbf{0.04}$ &$\mathbf{0.03}$ &$\mathbf{0.04}$ &$\mathbf{0.02}$\\
& $PCT_{ROS}$ &$0.69$ & $0.76$ & $0.7$ & $0.33$ & $0.56$ & $0.53$ & $0.67$ & $0.76$ & $0.7$ & $0.34$ & $0.57$ & $0.54$\\
& & $0.01$ & $0.04$ & $0.04$ & $0.06$ & $0.07$ & $0.03$ & $0.06$ & $0.05$ & $0.05$ & $0.1$ & $0.09$ & $0.06$\\\hline
& $PCT$ &$0.61$ & $\mathbf{0.67}$ &$\mathbf{0.63}$ &$0.46$ & $0.52$ & $0.53$ & $0.11$ & $0.95$ & $0.96$ & $0.92$ & $0.92$ & $0.93$\\
& & $0.22$ & $0.26$ & $0.35$ & $0.26$ & $0.21$ & $0.16$ & $0.15$ & $0.05$ & $0.06$ & $0.11$ & $0.08$ & $0.09$\\
& $PCT_{Sub}$ &$0.69$ & $0.8$ & $0.67$ & $0.33$ & $0.52$ & $0.52$ & $0.67$ & $0.81$ & $\mathbf{0.68}$ &$0.35$ & $0.53$ & $0.54$\\
\parbox[t]{2mm}{\multirow{2}{*}{\rotatebox[origin=c]{90}{$2000$, $5000$}}}& & $0.02$ & $\mathbf{0.02}$ &$0.04$ & $0.05$ & $0.03$ & $0.02$ & $0.09$ & $0.03$ & $0.05$ & $0.11$ & $0.07$ & $0.06$\\
& $PCT_{ET}$ &$0.67$ & $0.78$ & $0.72$ & $\mathbf{0.25}$ &$\mathbf{0.42}$ &$\mathbf{0.5}$ &$0.67$ & $0.78$ & $0.72$ & $\mathbf{0.25}$ &$\mathbf{0.42}$ &$\mathbf{0.5}$\\
& & $\mathbf{0.01}$ &$0.03$ & $\mathbf{0.03}$ &$\mathbf{0.01}$ &$\mathbf{0.01}$ &$\mathbf{0.01}$ &$\mathbf{0.01}$ &$\mathbf{0.03}$ &$\mathbf{0.03}$ &$\mathbf{0.01}$ &$\mathbf{0.01}$ &$\mathbf{0.01}$\\
& $PCT_{ROS}$ &$\mathbf{0.69}$ &$0.76$ & $0.69$ & $0.31$ & $0.54$ & $0.52$ & $\mathbf{0.69}$ &$\mathbf{0.76}$ &$0.69$ & $0.31$ & $0.54$ & $0.52$\\
& & $0.01$ & $0.03$ & $0.04$ & $0.06$ & $0.08$ & $0.03$ & $0.01$ & $0.03$ & $0.04$ & $0.06$ & $0.08$ & $0.03$\\\hline
& $PCT$ &$0.61$ & $\mathbf{0.67}$ &$\mathbf{0.63}$ &$0.46$ & $0.52$ & $0.53$ & $0.11$ & $0.95$ & $0.96$ & $0.92$ & $0.92$ & $0.93$\\
& & $0.22$ & $0.26$ & $0.35$ & $0.26$ & $0.21$ & $0.16$ & $0.15$ & $0.05$ & $0.06$ & $0.11$ & $0.08$ & $0.09$\\
& $PCT_{Sub}$ &$0.69$ & $0.8$ & $0.67$ & $0.33$ & $0.52$ & $0.52$ & $0.67$ & $0.81$ & $\mathbf{0.68}$ &$0.35$ & $0.53$ & $0.54$\\
\parbox[t]{2mm}{\multirow{2}{*}{\rotatebox[origin=c]{90}{$3000$, $6000$}}}& & $0.02$ & $\mathbf{0.02}$ &$0.04$ & $0.05$ & $0.03$ & $0.02$ & $0.09$ & $0.03$ & $0.05$ & $0.11$ & $0.07$ & $0.06$\\
& $PCT_{ET}$ &$0.68$ & $0.78$ & $0.72$ & $\mathbf{0.24}$ &$\mathbf{0.41}$ &$\mathbf{0.49}$ &$0.68$ & $0.78$ & $0.72$ & $\mathbf{0.24}$ &$\mathbf{0.41}$ &$\mathbf{0.49}$\\
& & $\mathbf{0.01}$ &$0.02$ & $\mathbf{0.02}$ &$\mathbf{0.01}$ &$\mathbf{0.02}$ &$\mathbf{0.01}$ &$\mathbf{0.01}$ &$\mathbf{0.02}$ &$\mathbf{0.02}$ &$\mathbf{0.01}$ &$\mathbf{0.02}$ &$\mathbf{0.01}$\\
& $PCT_{ROS}$ &$\mathbf{0.69}$ &$0.75$ & $0.7$ & $0.29$ & $0.5$ & $0.51$ & $\mathbf{0.69}$ &$\mathbf{0.75}$ &$0.7$ & $0.29$ & $0.5$ & $0.51$\\
& & $0.01$ & $0.03$ & $0.04$ & $0.06$ & $0.08$ & $0.03$ & $0.01$ & $0.03$ & $0.04$ & $0.06$ & $0.08$ & $0.03$\\\hline
\end{longtable}
\end{footnotesize}
\end{center}

On the Phenotype dataset (see Table \ref{tab:Supp3}) the framework manages to create very small number of redescriptions, satisfying predefined constraints, without using supplementing models. This causes the approach to have a relatively favourable averages, but very high standard deviation. Thus, the $\underline{underline}$ scores show the true performance difference between using the framework with and without supplementing models. The framework using the Sub supplementing model outperforms the other approaches on the Phenotype dataset.

\begin{center}
\begin{footnotesize}
\LTcapwidth=\textwidth
\begin{longtable}[c]{|c|c|c|c|c|c|c|c|c|c|c|c|c|c|} % <-- Replaces \begin{table}, alignment must be 
 \caption{Quality of redescription sets produced on the Phenotype dataset using the framework for multi-view redescription mining with a Random Forest supplementing model containing $50$ trees, given different memory sizes (work size, maximal memory size).}
  \label{tab:Supp3}\\
 \hline
 $M$ & $\mathcal{M}$ & $AJ$ & $Ap_{sc}$ & $AEJ$ &$AAJ$ & $ARC$ & $RSS$& $\underline{AJ}$ & $\underline{Ap_{sc}}$ & $\underline{AEJ}$ & $\underline{AAJ}$ & $\underline{ARC}$ & $\underline{RSS}$ \\  \hline
 
   \endfirsthead

\multicolumn{14}{c}%
        {{\textbf{ Table \thetable\ } Continued from previous page}} \\
        \hline
        
   $M$ & $\mathcal{M}$ & $AJ$ & $Ap_{sc}$ & $AEJ$ &$AAJ$ & $ARC$ & $RSS$& $\underline{AJ}$ & $\underline{Ap_{sc}}$ & $\underline{AEJ}$ & $\underline{AAJ}$ & $\underline{ARC}$ & $\underline{RSS}$ \\  \hline

  \endhead % <--  
& $PCT$ &$0.34$ & $\mathbf{0.36}$ &$\mathbf{0.06}$ &$0.03$ & $\mathbf{0.16}$ &$\mathbf{0.25}$ &$0.0$ & $0.99$ & $0.99$ & $0.99$ & $0.99$ & $0.99$\\
& & $0.37$ & $0.42$ & $0.12$ & $0.07$ & $0.17$ & $0.09$ & $\mathbf{0.0}$ &$\mathbf{0.0}$ &$\mathbf{0.0}$ &$0.01$ & $\mathbf{0.0}$ &$\mathbf{0.0}$\\
& $PCT_{Sub}$ &$\mathbf{0.74}$ &$0.84$ & $0.58$ & $\mathbf{0.02}$ &$0.38$ & $0.42$ & $\mathbf{0.74}$ &$\mathbf{0.84}$ &$\mathbf{0.58}$ &$\mathbf{0.02}$ &$\mathbf{0.38}$ &$\mathbf{0.42}$\\
\parbox[t]{2mm}{\multirow{2}{*}{\rotatebox[origin=c]{90}{$200$, $1700$}}}& & $\mathbf{0.02}$ &$0.02$ & $0.04$ & $\mathbf{0.0}$ &$\mathbf{0.02}$ &$0.01$ & $0.02$ & $0.02$ & $0.04$ & $\mathbf{0.0}$ &$0.02$ & $0.01$\\
& $PCT_{ET}$ &$0.74$ & $0.86$ & $0.64$ & $0.04$ & $0.43$ & $0.45$ & $0.69$ & $0.87$ & $0.67$ & $0.09$ & $0.47$ & $0.48$\\
& & $0.04$ & $\mathbf{0.0}$ &$\mathbf{0.04}$ &$0.01$ & $0.03$ & $\mathbf{0.01}$ &$0.13$ & $0.02$ & $0.05$ & $0.15$ & $0.08$ & $0.08$\\
& $PCT_{ROS}$ &$0.73$ & $0.86$ & $0.63$ & $0.04$ & $0.39$ & $0.44$ & $0.7$ & $0.87$ & $0.65$ & $0.09$ & $0.42$ & $0.47$\\
& & $0.04$ & $0.01$ & $0.04$ & $0.02$ & $0.03$ & $0.01$ & $0.11$ & $0.01$ & $0.05$ & $0.12$ & $0.09$ & $0.07$\\\hline
& $PCT$ &$0.34$ & $\mathbf{0.36}$ &$\mathbf{0.06}$ &$0.03$ & $\mathbf{0.16}$ &$\mathbf{0.25}$ &$0.0$ & $0.99$ & $0.99$ & $0.99$ & $0.99$ & $0.99$\\
& & $0.37$ & $0.42$ & $0.12$ & $0.07$ & $0.17$ & $0.09$ & $\mathbf{0.0}$ &$\mathbf{0.0}$ &$\mathbf{0.0}$ &$0.01$ & $\mathbf{0.0}$ &$\mathbf{0.0}$\\
& $PCT_{Sub}$ &$\mathbf{0.74}$ &$0.84$ & $0.58$ & $\mathbf{0.02}$ &$0.38$ & $0.42$ & $\mathbf{0.74}$ &$\mathbf{0.84}$ &$\mathbf{0.58}$ &$\mathbf{0.02}$ &$\mathbf{0.38}$ &$\mathbf{0.42}$\\
\parbox[t]{2mm}{\multirow{2}{*}{\rotatebox[origin=c]{90}{$300$, $1800$}}}& & $\mathbf{0.02}$ &$0.02$ & $0.05$ & $\mathbf{0.0}$ &$\mathbf{0.02}$ &$0.01$ & $0.02$ & $0.02$ & $0.05$ & $\mathbf{0.0}$ &$0.02$ & $0.01$\\
& $PCT_{ET}$ &$0.74$ & $0.86$ & $0.64$ & $0.04$ & $0.43$ & $0.45$ & $0.69$ & $0.87$ & $0.67$ & $0.09$ & $0.47$ & $0.48$\\
& & $0.04$ & $\mathbf{0.0}$ &$\mathbf{0.04}$ &$0.01$ & $0.03$ & $\mathbf{0.01}$ &$0.13$ & $0.02$ & $0.05$ & $0.15$ & $0.08$ & $0.08$\\
& $PCT_{ROS}$ &$0.73$ & $0.86$ & $0.63$ & $0.04$ & $0.39$ & $0.44$ & $0.7$ & $0.87$ & $0.65$ & $0.09$ & $0.42$ & $0.47$\\
& & $0.04$ & $0.01$ & $0.04$ & $0.02$ & $0.03$ & $0.01$ & $0.11$ & $0.01$ & $0.04$ & $0.12$ & $0.09$ & $0.07$\\\hline
& $PCT$ &$0.34$ & $\mathbf{0.36}$ &$\mathbf{0.06}$ &$0.03$ & $\mathbf{0.16}$ &$\mathbf{0.25}$ &$0.0$ & $0.99$ & $0.99$ & $0.99$ & $0.99$ & $0.99$\\
& & $0.37$ & $0.42$ & $0.12$ & $0.07$ & $0.17$ & $0.09$ & $\mathbf{0.0}$ &$\mathbf{0.0}$ &$\mathbf{0.0}$ &$\mathbf{0.01}$ &$\mathbf{0.0}$ &$\mathbf{0.0}$\\
& $PCT_{Sub}$ &$\mathbf{0.74}$ &$0.84$ & $0.58$ & $\mathbf{0.02}$ &$0.37$ & $0.41$ & $\mathbf{0.74}$ &$\mathbf{0.84}$ &$\mathbf{0.58}$ &$\mathbf{0.02}$ &$\mathbf{0.37}$ &$\mathbf{0.41}$\\
\parbox[t]{2mm}{\multirow{2}{*}{\rotatebox[origin=c]{90}{$400$, $1900$}}}& & $\mathbf{0.02}$ &$0.02$ & $0.05$ & $\mathbf{0.01}$ &$\mathbf{0.02}$ &$0.01$ & $0.02$ & $0.02$ & $0.05$ & $0.01$ & $0.02$ & $0.01$\\
& $PCT_{ET}$ &$0.73$ & $0.86$ & $0.64$ & $0.04$ & $0.44$ & $0.45$ & $0.68$ & $0.87$ & $0.67$ & $0.11$ & $0.48$ & $0.49$\\
& & $0.04$ & $\mathbf{0.0}$ &$\mathbf{0.04}$ &$0.02$ & $0.03$ & $0.01$ & $0.14$ & $0.02$ & $0.05$ & $0.16$ & $0.09$ & $0.09$\\
& $PCT_{ROS}$ &$0.73$ & $0.86$ & $0.63$ & $0.04$ & $0.39$ & $0.44$ & $0.7$ & $0.87$ & $0.65$ & $0.09$ & $0.42$ & $0.47$\\
& & $0.04$ & $0.01$ & $0.04$ & $0.02$ & $0.03$ & $\mathbf{0.01}$ &$0.11$ & $0.01$ & $0.05$ & $0.12$ & $0.09$ & $0.07$\\\hline
& $PCT$ &$0.34$ & $\mathbf{0.36}$ &$\mathbf{0.06}$ &$0.03$ & $\mathbf{0.16}$ &$\mathbf{0.25}$ &$0.0$ & $0.99$ & $0.99$ & $0.99$ & $0.99$ & $0.99$\\
& & $0.37$ & $0.42$ & $0.12$ & $0.07$ & $0.17$ & $0.09$ & $\mathbf{0.0}$ &$\mathbf{0.0}$ &$\mathbf{0.0}$ &$\mathbf{0.01}$ &$\mathbf{0.0}$ &$\mathbf{0.0}$\\
& $PCT_{Sub}$ &$0.74$ & $0.84$ & $0.58$ & $\mathbf{0.02}$ &$0.37$ & $0.42$ & $\mathbf{0.74}$ &$\mathbf{0.84}$ &$\mathbf{0.58}$ &$\mathbf{0.02}$ &$\mathbf{0.37}$ &$\mathbf{0.42}$\\
\parbox[t]{2mm}{\multirow{2}{*}{\rotatebox[origin=c]{90}{$500$, $2000$}}}& & $\mathbf{0.02}$ &$0.02$ & $0.05$ & $\mathbf{0.01}$ &$\mathbf{0.02}$ &$0.01$ & $0.02$ & $0.02$ & $0.05$ & $0.01$ & $0.02$ & $0.01$\\
& $PCT_{ET}$ &$\mathbf{0.74}$ &$0.86$ & $0.65$ & $0.04$ & $0.44$ & $0.45$ & $0.66$ & $0.88$ & $0.69$ & $0.15$ & $0.5$ & $0.51$\\
& & $0.03$ & $0.01$ & $0.04$ & $0.02$ & $0.03$ & $0.01$ & $0.16$ & $0.02$ & $0.07$ & $0.2$ & $0.11$ & $0.11$\\
& $PCT_{ROS}$ &$0.73$ & $0.86$ & $0.64$ & $0.04$ & $0.39$ & $0.44$ & $0.7$ & $0.87$ & $0.66$ & $0.08$ & $0.42$ & $0.46$\\
& & $0.04$ & $\mathbf{0.0}$ &$\mathbf{0.04}$ &$0.02$ & $0.03$ & $\mathbf{0.01}$ &$0.1$ & $0.01$ & $0.05$ & $0.11$ & $0.08$ & $0.06$\\\hline
& $PCT$ &$0.34$ & $\mathbf{0.36}$ &$\mathbf{0.06}$ &$0.03$ & $\mathbf{0.16}$ &$\mathbf{0.25}$ &$0.0$ & $0.99$ & $0.99$ & $0.99$ & $0.99$ & $0.99$\\
& & $0.37$ & $0.42$ & $0.12$ & $0.07$ & $0.17$ & $0.09$ & $\mathbf{0.0}$ &$\mathbf{0.0}$ &$\mathbf{0.0}$ &$0.01$ & $\mathbf{0.0}$ &$\mathbf{0.0}$\\
& $PCT_{Sub}$ &$0.73$ & $0.84$ & $0.58$ & $\mathbf{0.02}$ &$0.36$ & $0.41$ & $\mathbf{0.73}$ &$\mathbf{0.84}$ &$\mathbf{0.58}$ &$\mathbf{0.02}$ &$\mathbf{0.36}$ &$\mathbf{0.41}$\\
\parbox[t]{2mm}{\multirow{2}{*}{\rotatebox[origin=c]{90}{$1000$, $4000$}}}& & $0.03$ & $0.02$ & $0.04$ & $\mathbf{0.01}$ &$\mathbf{0.02}$ &$\mathbf{0.01}$ &$0.03$ & $0.02$ & $0.04$ & $\mathbf{0.01}$ &$0.02$ & $0.01$\\
& $PCT_{ET}$ &$\mathbf{0.74}$ &$0.86$ & $0.65$ & $0.05$ & $0.44$ & $0.45$ & $0.65$ & $0.88$ & $0.7$ & $0.16$ & $0.51$ & $0.52$\\
& & $\mathbf{0.02}$ &$0.01$ & $\mathbf{0.03}$ &$0.03$ & $0.03$ & $0.01$ & $0.18$ & $0.03$ & $0.09$ & $0.24$ & $0.13$ & $0.13$\\
& $PCT_{ROS}$ &$0.74$ & $0.86$ & $0.64$ & $0.04$ & $0.39$ & $0.44$ & $0.69$ & $0.87$ & $0.66$ & $0.09$ & $0.43$ & $0.47$\\
& & $0.04$ & $\mathbf{0.0}$ &$0.03$ & $0.02$ & $0.03$ & $0.01$ & $0.11$ & $0.02$ & $0.05$ & $0.13$ & $0.09$ & $0.08$\\\hline
& $PCT$ &$0.34$ & $\mathbf{0.36}$ &$\mathbf{0.06}$ &$0.03$ & $\mathbf{0.16}$ &$\mathbf{0.25}$ &$0.0$ & $0.99$ & $0.99$ & $0.99$ & $0.99$ & $0.99$\\
& & $0.37$ & $0.42$ & $0.12$ & $0.07$ & $0.17$ & $0.09$ & $\mathbf{0.0}$ &$\mathbf{0.0}$ &$\mathbf{0.0}$ &$\mathbf{0.01}$ &$\mathbf{0.0}$ &$\mathbf{0.0}$\\
& $PCT_{Sub}$ &$0.74$ & $0.84$ & $0.58$ & $\mathbf{0.02}$ &$0.36$ & $0.41$ & $\mathbf{0.74}$ &$\mathbf{0.84}$ &$\mathbf{0.58}$ &$\mathbf{0.02}$ &$\mathbf{0.36}$ &$\mathbf{0.41}$\\
\parbox[t]{2mm}{\multirow{2}{*}{\rotatebox[origin=c]{90}{$2000$, $5000$}}}& & $\mathbf{0.02}$ &$0.01$ & $0.04$ & $\mathbf{0.01}$ &$\mathbf{0.02}$ &$\mathbf{0.01}$ &$0.02$ & $0.01$ & $0.04$ & $0.01$ & $0.02$ & $0.01$\\
& $PCT_{ET}$ &$\mathbf{0.75}$ &$0.86$ & $0.65$ & $0.04$ & $0.44$ & $0.45$ & $0.65$ & $0.88$ & $0.7$ & $0.16$ & $0.52$ & $0.52$\\
& & $0.03$ & $\mathbf{0.0}$ &$0.04$ & $0.02$ & $0.03$ & $0.01$ & $0.19$ & $0.03$ & $0.09$ & $0.24$ & $0.14$ & $0.13$\\
& $PCT_{ROS}$ &$0.74$ & $0.86$ & $0.64$ & $0.04$ & $0.39$ & $0.44$ & $0.69$ & $0.87$ & $0.66$ & $0.1$ & $0.43$ & $0.47$\\
& & $0.04$ & $0.0$ & $\mathbf{0.04}$ &$0.02$ & $0.04$ & $0.01$ & $0.11$ & $0.02$ & $0.06$ & $0.14$ & $0.1$ & $0.08$\\\hline
& $PCT$ &$0.34$ & $\mathbf{0.36}$ &$\mathbf{0.06}$ &$0.03$ & $\mathbf{0.16}$ &$\mathbf{0.25}$ &$0.0$ & $0.99$ & $0.99$ & $0.99$ & $0.99$ & $0.99$\\
& & $0.37$ & $0.42$ & $0.12$ & $0.07$ & $0.17$ & $0.09$ & $\mathbf{0.0}$ &$\mathbf{0.0}$ &$\mathbf{0.0}$ &$\mathbf{0.01}$ &$\mathbf{0.0}$ &$\mathbf{0.0}$\\
& $PCT_{Sub}$ &$0.74$ & $0.84$ & $0.58$ & $\mathbf{0.02}$ &$0.36$ & $0.41$ & $\mathbf{0.74}$ &$\mathbf{0.84}$ &$\mathbf{0.58}$ &$\mathbf{0.02}$ &$\mathbf{0.36}$ &$\mathbf{0.41}$\\
\parbox[t]{2mm}{\multirow{2}{*}{\rotatebox[origin=c]{90}{$3000$, $6000$}}}& & $\mathbf{0.02}$ &$0.01$ & $0.04$ & $\mathbf{0.01}$ &$\mathbf{0.02}$ &$\mathbf{0.01}$ &$0.02$ & $0.01$ & $0.04$ & $0.01$ & $0.02$ & $0.01$\\
& $PCT_{ET}$ &$\mathbf{0.75}$ &$0.86$ & $0.65$ & $0.04$ & $0.44$ & $0.45$ & $0.65$ & $0.88$ & $0.7$ & $0.16$ & $0.52$ & $0.52$\\
& & $0.03$ & $\mathbf{0.0}$ &$0.04$ & $0.02$ & $0.03$ & $0.01$ & $0.19$ & $0.03$ & $0.09$ & $0.24$ & $0.14$ & $0.13$\\
& $PCT_{ROS}$ &$0.74$ & $0.86$ & $0.64$ & $0.04$ & $0.39$ & $0.44$ & $0.69$ & $0.87$ & $0.66$ & $0.1$ & $0.43$ & $0.47$\\
& & $0.04$ & $0.0$ & $\mathbf{0.04}$ &$0.02$ & $0.04$ & $0.01$ & $0.11$ & $0.02$ & $0.06$ & $0.14$ & $0.1$ & $0.08$\\\hline
\end{longtable}
\end{footnotesize}
\end{center}

\begin{figure}[H]
\centerline{\includegraphics[width=1.0\textwidth]{Figures/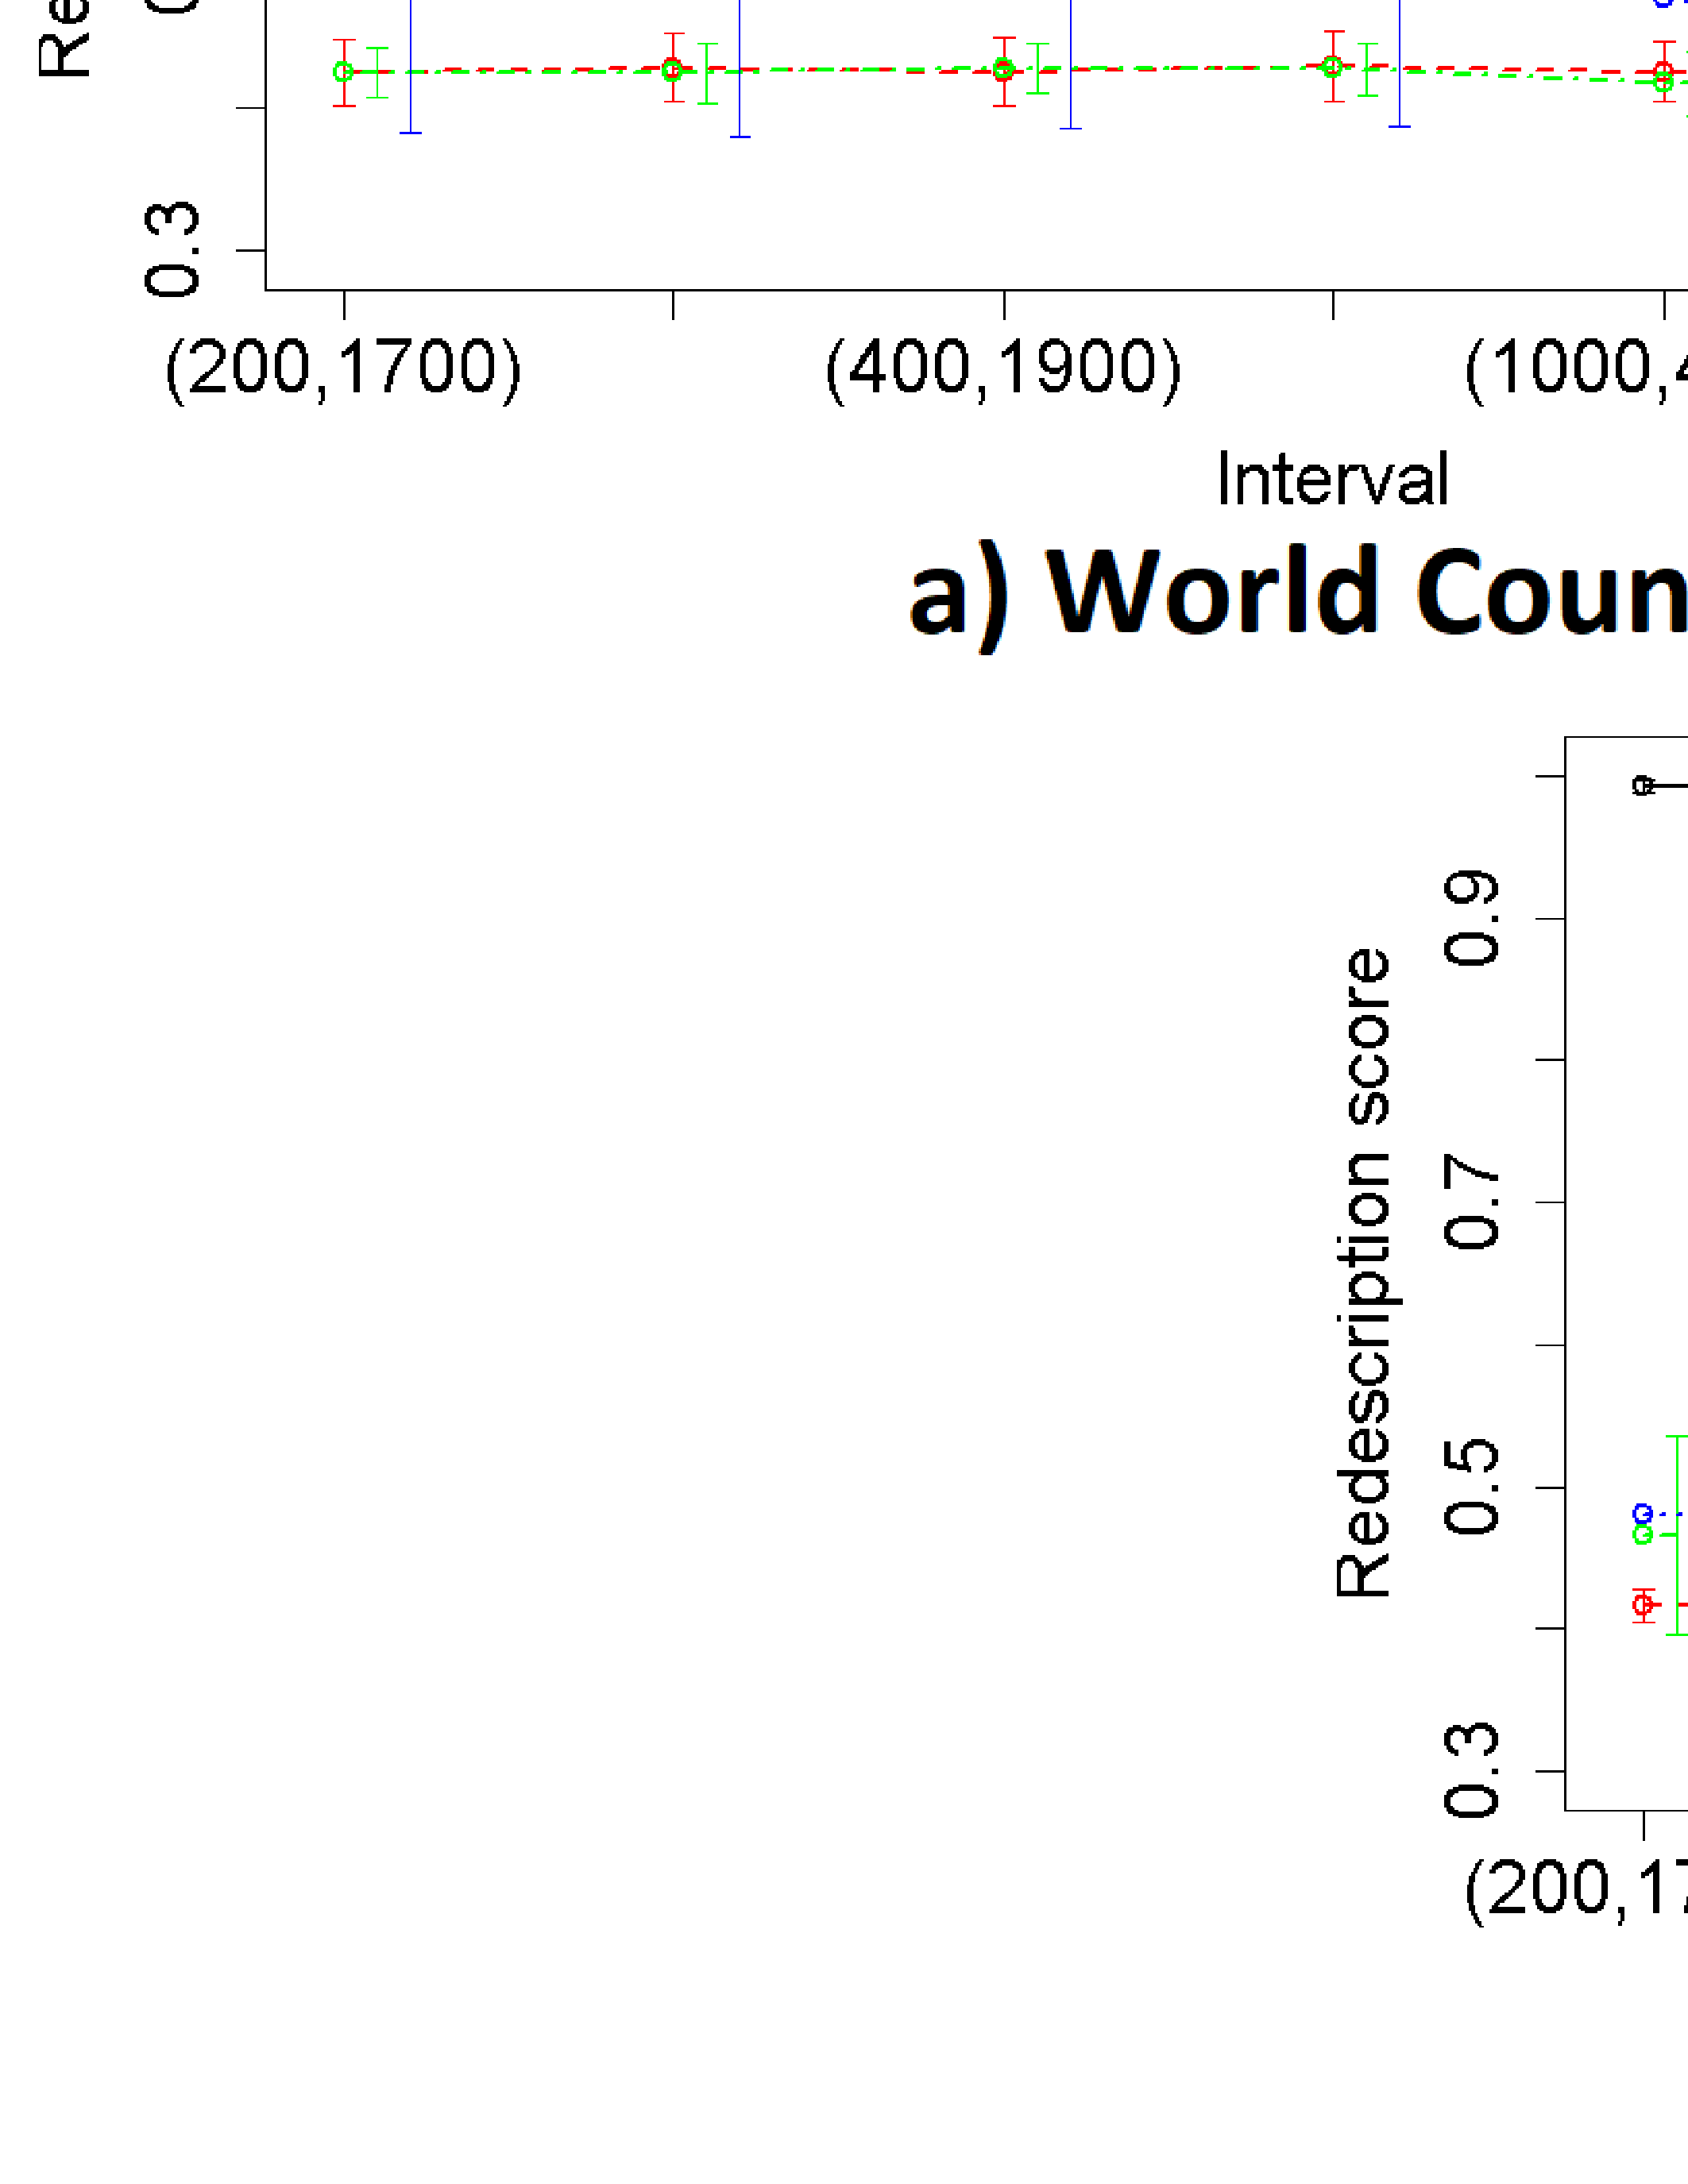}}\caption{Overall redescription set score $\underline{total_{sc}}(\mathcal{R})$ obtained using a single rule-generating PCT model and a supplementing model containing $50$ trees with different memory parameters.}
\label{fig:SM}
\end{figure}

It is visible from Tables \ref{tab:Supp1}, \ref{tab:Supp2} and \ref{tab:Supp3}, as well as Figure \ref{fig:SM}, that using supplementing models significantly increases the performance of the proposed framework (both with respect to accuracy and stability). The corresponding $p$-values of the difference in mean value of the average redescription set score achieved using a supplementing model compared to using only a single rule-generating PCT at each memory setting, according to the one-sided Wilcoxon signed-rank test, are: $p_{(PCT_{Sub},PCT)}= 7.8\cdot 10^{-3} $, $p_{(PCT_{ET}, PCT)}= 7.8\cdot 10^{-3} $, $p_{(PCT_{ROS}, PCT)}= 7.8\cdot 10^{-3}$ on the World Country dataset, $p_{(PCT_{Sub},PCT)}= 0.011 $, $p_{(PCT_{ET}, PCT)}= 7.8\cdot 10^{-3} $, $p_{(PCT_{ROS}, PCT)}= 7.8\cdot 10^{-3}$ on the Slovenian Water dataset and $p_{(PCT_{Sub},PCT)}= 7.8\cdot 10^{-3} $, $p_{(PCT_{ET}, PCT)}= 0.011 $, $p_{(PCT_{ROS}, PCT)}= 7.8\cdot 10^{-3}$ on the Phenotype dataset. 
%use paired test, because memory parameters are the same???
Figure \ref{fig:SM} shows that increasing the memory parameters increases performance of the framework with supplementing model on the World Country and the Slovenian Water dataset, while the performance slightly degrades when the Extra multi-target PCTs are used as a supplementing model, with the increased memory parameters, on the Phenotype dataset. The main reason is the instability that occurs due to the model inability to produce $200$ redescriptions at each run.

Tables and Figures containing results of using supplementing models \cite{MihelcicRF2017} with $20$ trees are presented below.

\begin{center}
\begin{footnotesize}
\LTcapwidth=\textwidth
\begin{longtable}[c]{|c|c|c|c|c|c|c|c|c|c|c|c|c|c|} % <-- Replaces \begin{table}, alignment must be 
 \caption{Quality of redescription sets produced on the World Country dataset using the framework for multi-view redescription mining with a Random Forest supplementing model containing $20$ trees. We denote memory parameters with numbers, $1$ denoting work size of $200$ and maximal memory size of $1700$ and $7$ denoting $3000$, $6000$ memory parameters.}
  \label{tab:Supp1}\\
 \hline
 $M$ & $\mathcal{M}$ & $AJ$ & $Ap_{sc}$ & $AEJ$ &$AAJ$ & $ARC$ & $RSS$& $\underline{AJ}$ & $\underline{Ap_{sc}}$ & $\underline{AEJ}$ & $\underline{AAJ}$ & $\underline{ARC}$ & $\underline{RSS}$ \\  \hline

  \endhead % <--  
& $PCT$ &$0.71$ & $0.41$ & $0.78$ & $0.34$ & $\mathbf{0.63}$ &$0.49$ & $0.37$ & $0.68$ & $0.89$ & $0.63$ & $0.81$ & $0.73$\\
& & $0.04$ & $0.14$ & $0.1$ & $0.13$ & $\mathbf{0.06}$ &$0.05$ & $0.27$ & $0.28$ & $0.1$ & $0.28$ & $0.13$ & $0.2$\\
& $PCT_{Sub}$ &$\mathbf{0.75}$ &$\mathbf{0.35}$ &$0.75$ & $0.13$ & $0.71$ & $0.44$ & $\mathbf{0.75}$ &$\mathbf{0.35}$ &$0.75$ & $0.13$ & $\mathbf{0.71}$ &$0.44$\\
1& & $0.02$ & $0.14$ & $0.08$ & $0.02$ & $0.09$ & $\mathbf{0.02}$ &$\mathbf{0.02}$ &$0.14$ & $0.08$ & $0.02$ & $0.09$ & $\mathbf{0.02}$\\
& $PCT_{ET}$ &$0.75$ & $0.36$ & $0.78$ & $0.18$ & $0.75$ & $0.47$ & $0.72$ & $0.39$ & $0.79$ & $0.21$ & $0.75$ & $0.48$\\
& & $\mathbf{0.01}$ &$0.14$ & $0.08$ & $0.05$ & $0.08$ & $0.03$ & $0.07$ & $0.1$ & $0.08$ & $0.1$ & $0.09$ & $0.05$\\
& $PCT_{ROS}$ &$0.75$ & $0.36$ & $\mathbf{0.72}$ &$\mathbf{0.12}$ &$0.71$ & $\mathbf{0.43}$ &$0.75$ & $0.36$ & $\mathbf{0.72}$ &$\mathbf{0.12}$ &$0.71$ & $\mathbf{0.43}$\\
& & $0.02$ & $\mathbf{0.1}$ &$\mathbf{0.07}$ &$\mathbf{0.02}$ &$0.07$ & $0.02$ & $0.02$ & $\mathbf{0.1}$ &$\mathbf{0.07}$ &$\mathbf{0.02}$ &$\mathbf{0.07}$ &$0.02$\\\hline
& $PCT$ &$0.7$ & $0.41$ & $0.79$ & $0.34$ & $\mathbf{0.62}$ &$0.49$ & $0.37$ & $0.68$ & $0.89$ & $0.63$ & $0.81$ & $0.73$\\
& & $0.03$ & $0.14$ & $0.1$ & $0.14$ & $\mathbf{0.06}$ &$0.05$ & $0.27$ & $0.28$ & $0.11$ & $0.28$ & $0.13$ & $0.21$\\
& $PCT_{Sub}$ &$\mathbf{0.75}$ &$0.35$ & $\mathbf{0.74}$ &$\mathbf{0.13}$ &$0.7$ & $\mathbf{0.43}$ &$\mathbf{0.75}$ &$0.35$ & $\mathbf{0.74}$ &$\mathbf{0.13}$ &$\mathbf{0.7}$ &$\mathbf{0.43}$\\
2& & $0.02$ & $0.15$ & $0.07$ & $0.03$ & $0.07$ & $0.03$ & $\mathbf{0.02}$ &$0.15$ & $0.07$ & $0.03$ & $0.07$ & $0.03$\\
& $PCT_{ET}$ &$0.75$ & $0.37$ & $0.78$ & $0.18$ & $0.75$ & $0.46$ & $0.7$ & $0.41$ & $0.79$ & $0.23$ & $0.76$ & $0.5$\\
& & $\mathbf{0.01}$ &$0.14$ & $0.07$ & $0.05$ & $0.09$ & $0.03$ & $0.11$ & $0.13$ & $\mathbf{0.07}$ &$0.13$ & $0.1$ & $0.08$\\
& $PCT_{ROS}$ &$0.75$ & $\mathbf{0.34}$ &$0.74$ & $0.13$ & $0.71$ & $0.44$ & $0.75$ & $\mathbf{0.34}$ &$0.74$ & $0.13$ & $0.71$ & $0.44$\\
& & $0.02$ & $\mathbf{0.12}$ &$\mathbf{0.07}$ &$\mathbf{0.03}$ &$0.06$ & $\mathbf{0.02}$ &$0.02$ & $\mathbf{0.12}$ &$0.07$ & $\mathbf{0.03}$ &$\mathbf{0.06}$ &$\mathbf{0.02}$\\\hline
& $PCT$ &$0.7$ & $0.4$ & $0.79$ & $0.34$ & $\mathbf{0.61}$ &$0.49$ & $0.36$ & $0.68$ & $0.89$ & $0.63$ & $0.8$ & $0.73$\\
& & $0.03$ & $0.15$ & $0.1$ & $0.14$ & $\mathbf{0.06}$ &$0.05$ & $0.26$ & $0.29$ & $0.11$ & $0.29$ & $0.15$ & $0.21$\\
& $PCT_{Sub}$ &$0.75$ & $0.36$ & $0.74$ & $\mathbf{0.12}$ &$0.69$ & $0.43$ & $0.75$ & $0.36$ & $0.74$ & $\mathbf{0.12}$ &$\mathbf{0.69}$ &$0.43$\\
3& & $0.02$ & $0.14$ & $0.07$ & $0.03$ & $0.07$ & $\mathbf{0.02}$ &$\mathbf{0.02}$ &$0.14$ & $0.07$ & $0.03$ & $0.07$ & $\mathbf{0.02}$\\
& $PCT_{ET}$ &$\mathbf{0.75}$ &$0.35$ & $0.78$ & $0.18$ & $0.75$ & $0.46$ & $0.72$ & $0.39$ & $0.78$ & $0.21$ & $0.75$ & $0.48$\\
& & $\mathbf{0.01}$ &$0.14$ & $0.09$ & $0.05$ & $0.08$ & $0.03$ & $0.1$ & $\mathbf{0.1}$ &$0.1$ & $0.14$ & $0.09$ & $0.08$\\
& $PCT_{ROS}$ &$0.75$ & $\mathbf{0.33}$ &$\mathbf{0.73}$ &$0.13$ & $0.71$ & $\mathbf{0.43}$ &$\mathbf{0.75}$ &$\mathbf{0.33}$ &$\mathbf{0.73}$ &$0.13$ & $0.71$ & $\mathbf{0.43}$\\
& & $0.02$ & $\mathbf{0.13}$ &$\mathbf{0.07}$ &$\mathbf{0.02}$ &$0.07$ & $0.02$ & $0.02$ & $0.13$ & $\mathbf{0.07}$ &$\mathbf{0.02}$ &$\mathbf{0.07}$ &$0.02$\\\hline
& $PCT$ &$0.7$ & $0.41$ & $0.79$ & $0.34$ & $\mathbf{0.61}$ &$0.49$ & $0.36$ & $0.68$ & $0.89$ & $0.63$ & $0.8$ & $0.73$\\
& & $0.03$ & $0.15$ & $0.1$ & $0.14$ & $\mathbf{0.06}$ &$0.05$ & $0.27$ & $0.28$ & $0.11$ & $0.29$ & $0.15$ & $0.21$\\
& $PCT_{Sub}$ &$0.75$ & $0.35$ & $0.73$ & $\mathbf{0.12}$ &$0.7$ & $0.43$ & $0.75$ & $0.35$ & $0.73$ & $\mathbf{0.12}$ &$\mathbf{0.7}$ &$0.43$\\
4& & $0.01$ & $0.14$ & $0.07$ & $0.03$ & $0.07$ & $\mathbf{0.02}$ &$\mathbf{0.01}$ &$0.14$ & $0.07$ & $0.03$ & $0.07$ & $\mathbf{0.02}$\\
& $PCT_{ET}$ &$0.75$ & $\mathbf{0.34}$ &$0.78$ & $0.18$ & $0.75$ & $0.46$ & $0.72$ & $0.38$ & $0.78$ & $0.21$ & $0.75$ & $0.48$\\
& & $\mathbf{0.01}$ &$0.13$ & $0.09$ & $0.05$ & $0.09$ & $0.03$ & $0.1$ & $\mathbf{0.09}$ &$0.1$ & $0.14$ & $0.1$ & $0.08$\\
& $PCT_{ROS}$ &$\mathbf{0.75}$ &$0.34$ & $\mathbf{0.72}$ &$0.13$ & $0.72$ & $\mathbf{0.43}$ &$\mathbf{0.75}$ &$\mathbf{0.34}$ &$\mathbf{0.72}$ &$0.13$ & $0.72$ & $\mathbf{0.43}$\\
& & $0.02$ & $\mathbf{0.12}$ &$\mathbf{0.06}$ &$\mathbf{0.02}$ &$0.06$ & $0.02$ & $0.02$ & $0.12$ & $\mathbf{0.06}$ &$\mathbf{0.02}$ &$\mathbf{0.06}$ &$0.02$\\\hline
& $PCT$ &$0.7$ & $0.4$ & $0.79$ & $0.34$ & $\mathbf{0.61}$ &$0.49$ & $0.36$ & $0.68$ & $0.89$ & $0.63$ & $0.8$ & $0.73$\\
& & $0.03$ & $0.15$ & $0.09$ & $0.14$ & $0.06$ & $0.05$ & $0.26$ & $0.29$ & $0.11$ & $0.29$ & $0.15$ & $0.21$\\
& $PCT_{Sub}$ &$0.74$ & $0.34$ & $0.75$ & $\mathbf{0.13}$ &$0.67$ & $0.43$ & $0.74$ & $0.34$ & $0.76$ & $0.14$ & $\mathbf{0.68}$ &$0.44$\\
5& & $0.02$ & $0.16$ & $0.09$ & $0.02$ & $0.06$ & $0.03$ & $0.03$ & $0.16$ & $0.08$ & $0.04$ & $0.07$ & $0.04$\\
& $PCT_{ET}$ &$\mathbf{0.75}$ &$0.33$ & $0.78$ & $0.17$ & $0.73$ & $0.45$ & $0.72$ & $0.37$ & $0.79$ & $0.2$ & $0.74$ & $0.47$\\
& & $\mathbf{0.01}$ &$0.12$ & $\mathbf{0.07}$ &$0.06$ & $0.07$ & $0.03$ & $0.09$ & $\mathbf{0.09}$ &$0.08$ & $0.13$ & $0.08$ & $0.07$\\
& $PCT_{ROS}$ &$0.75$ & $\mathbf{0.3}$ &$\mathbf{0.73}$ &$0.13$ & $0.7$ & $\mathbf{0.42}$ &$\mathbf{0.75}$ &$\mathbf{0.3}$ &$\mathbf{0.73}$ &$\mathbf{0.13}$ &$0.7$ & $\mathbf{0.42}$\\
& & $0.02$ & $\mathbf{0.09}$ &$0.07$ & $\mathbf{0.02}$ &$\mathbf{0.06}$ &$\mathbf{0.02}$ &$\mathbf{0.02}$ &$0.09$ & $\mathbf{0.07}$ &$\mathbf{0.02}$ &$\mathbf{0.06}$ &$\mathbf{0.02}$\\\hline
& $PCT$ &$0.7$ & $0.4$ & $0.78$ & $0.34$ & $\mathbf{0.61}$ &$0.49$ & $0.36$ & $0.68$ & $0.88$ & $0.62$ & $0.8$ & $0.72$\\
& & $0.03$ & $0.15$ & $0.09$ & $0.14$ & $0.06$ & $0.05$ & $0.27$ & $0.29$ & $0.11$ & $0.29$ & $0.14$ & $0.21$\\
& $PCT_{Sub}$ &$0.74$ & $0.33$ & $0.74$ & $0.13$ & $0.66$ & $0.42$ & $0.73$ & $0.33$ & $0.75$ & $0.14$ & $\mathbf{0.66}$ &$0.43$\\
6& & $0.02$ & $0.15$ & $0.08$ & $0.03$ & $\mathbf{0.03}$ &$0.03$ & $0.03$ & $0.16$ & $\mathbf{0.07}$ &$0.04$ & $\mathbf{0.04}$ &$0.04$\\
& $PCT_{ET}$ &$0.75$ & $0.33$ & $0.79$ & $0.18$ & $0.72$ & $0.45$ & $0.72$ & $0.37$ & $0.79$ & $0.2$ & $0.73$ & $0.47$\\
& & $\mathbf{0.01}$ &$0.12$ & $\mathbf{0.08}$ &$0.06$ & $0.08$ & $0.03$ & $0.09$ & $\mathbf{0.09}$ &$0.08$ & $0.13$ & $0.09$ & $0.08$\\
& $PCT_{ROS}$ &$\mathbf{0.75}$ &$\mathbf{0.3}$ &$\mathbf{0.73}$ &$\mathbf{0.12}$ &$0.69$ & $\mathbf{0.42}$ &$\mathbf{0.75}$ &$\mathbf{0.3}$ &$\mathbf{0.73}$ &$\mathbf{0.12}$ &$0.69$ & $\mathbf{0.42}$\\
& & $0.02$ & $\mathbf{0.11}$ &$0.08$ & $\mathbf{0.02}$ &$0.07$ & $\mathbf{0.01}$ &$\mathbf{0.02}$ &$0.11$ & $0.08$ & $\mathbf{0.02}$ &$0.07$ & $\mathbf{0.01}$\\\hline
& $PCT$ &$0.7$ & $0.4$ & $0.78$ & $0.34$ & $\mathbf{0.61}$ &$0.49$ & $0.36$ & $0.68$ & $0.88$ & $0.62$ & $0.8$ & $0.72$\\
& & $0.03$ & $0.15$ & $0.09$ & $0.14$ & $0.06$ & $0.05$ & $0.27$ & $0.29$ & $0.11$ & $0.29$ & $0.14$ & $0.21$\\
& $PCT_{Sub}$ &$0.74$ & $0.32$ & $0.74$ & $\mathbf{0.12}$ &$0.67$ & $0.42$ & $0.73$ & $0.33$ & $0.74$ & $0.13$ & $\mathbf{0.67}$ &$0.43$\\
7& & $0.02$ & $0.15$ & $\mathbf{0.07}$ &$\mathbf{0.02}$ &$\mathbf{0.06}$ &$0.02$ & $0.04$ & $0.16$ & $\mathbf{0.06}$ &$0.04$ & $0.06$ & $0.04$\\
& $PCT_{ET}$ &$0.75$ & $0.33$ & $0.78$ & $0.17$ & $0.73$ & $0.45$ & $0.72$ & $0.37$ & $0.79$ & $0.2$ & $0.73$ & $0.47$\\
& & $\mathbf{0.01}$ &$0.12$ & $0.08$ & $0.06$ & $0.08$ & $0.03$ & $0.09$ & $\mathbf{0.08}$ &$0.09$ & $0.13$ & $0.09$ & $0.08$\\
& $PCT_{ROS}$ &$\mathbf{0.75}$ &$\mathbf{0.3}$ &$\mathbf{0.74}$ &$0.12$ & $0.69$ & $\mathbf{0.42}$ &$\mathbf{0.75}$ &$\mathbf{0.3}$ &$\mathbf{0.74}$ &$\mathbf{0.12}$ &$0.69$ & $\mathbf{0.42}$\\
& & $0.02$ & $\mathbf{0.11}$ &$0.08$ & $0.02$ & $0.06$ & $\mathbf{0.02}$ &$\mathbf{0.02}$ &$0.11$ & $0.08$ & $\mathbf{0.02}$ &$\mathbf{0.06}$ &$\mathbf{0.02}$\\\hline

\end{longtable}
\end{footnotesize}
\end{center}

\begin{center}
\begin{footnotesize}
\LTcapwidth=\textwidth
\begin{longtable}[c]{|c|c|c|c|c|c|c|c|c|c|c|c|c|c|} % <-- Replaces \begin{table}, alignment must be 
 \caption{Quality of redescription sets produced on the Slovenian Water dataset using the framework for multi-view redescription mining with a Random Forest supplementing model containing $20$ trees. We denote memory parameters with numbers, $1$ denoting work size of $200$ and maximal memory size of $1700$ and $7$ denoting $3000$, $6000$ memory parameters.}
  \label{tab:Supp2}\\
 \hline
 $M$ & $\mathcal{M}$ & $AJ$ & $Ap_{sc}$ & $AEJ$ &$AAJ$ & $ARC$ & $RSS$& $\underline{AJ}$ & $\underline{Ap_{sc}}$ & $\underline{AEJ}$ & $\underline{AAJ}$ & $\underline{ARC}$ & $\underline{RSS}$ \\  \hline

  \endhead % <--  
& $PCT$ &$0.61$ & $\mathbf{0.67}$ &$\mathbf{0.63}$ &$0.46$ & $0.52$ & $0.53$ & $0.11$ & $0.95$ & $0.96$ & $0.92$ & $0.92$ & $0.93$\\
& & $0.22$ & $0.26$ & $0.35$ & $0.26$ & $0.21$ & $0.16$ & $0.15$ & $0.05$ & $0.06$ & $0.11$ & $0.08$ & $0.09$\\
& $PCT_{Sub}$ &$0.69$ & $0.79$ & $0.68$ & $0.37$ & $0.53$ & $0.54$ & $0.65$ & $0.8$ & $\mathbf{0.7}$ &$0.4$ & $0.55$ & $0.56$\\
1& & $0.02$ & $\mathbf{0.02}$ &$0.05$ & $0.05$ & $0.04$ & $0.02$ & $0.07$ & $\mathbf{0.02}$ &$0.06$ & $0.09$ & $0.07$ & $0.06$\\
& $PCT_{ET}$ &$0.68$ & $0.78$ & $0.71$ & $\mathbf{0.29}$ &$\mathbf{0.47}$ &$\mathbf{0.51}$ &$\mathbf{0.68}$ &$0.78$ & $0.71$ & $\mathbf{0.29}$ &$\mathbf{0.47}$ &$\mathbf{0.51}$\\
& & $\mathbf{0.01}$ &$0.03$ & $\mathbf{0.03}$ &$\mathbf{0.03}$ &$\mathbf{0.03}$ &$\mathbf{0.02}$ &$\mathbf{0.01}$ &$0.03$ & $\mathbf{0.03}$ &$\mathbf{0.03}$ &$\mathbf{0.03}$ &$\mathbf{0.02}$\\
& $PCT_{ROS}$ &$\mathbf{0.69}$ &$0.77$ & $0.71$ & $0.34$ & $0.58$ & $0.54$ & $0.67$ & $\mathbf{0.78}$ &$0.72$ & $0.36$ & $0.59$ & $0.55$\\
& & $0.02$ & $0.04$ & $0.06$ & $0.06$ & $0.08$ & $0.03$ & $0.05$ & $0.05$ & $0.06$ & $0.1$ & $0.1$ & $0.06$\\\hline
& $PCT$ &$0.61$ & $\mathbf{0.67}$ &$\mathbf{0.63}$ &$0.46$ & $0.52$ & $0.53$ & $0.11$ & $0.95$ & $0.96$ & $0.92$ & $0.92$ & $0.93$\\
& & $0.22$ & $0.26$ & $0.35$ & $0.26$ & $0.21$ & $0.16$ & $0.15$ & $0.05$ & $0.06$ & $0.11$ & $0.08$ & $0.09$\\
& $PCT_{Sub}$ &$0.69$ & $0.79$ & $0.68$ & $0.37$ & $0.53$ & $0.54$ & $0.65$ & $0.8$ & $\mathbf{0.7}$ &$0.4$ & $0.55$ & $0.56$\\
2& & $0.02$ & $\mathbf{0.02}$ &$0.05$ & $0.05$ & $0.04$ & $0.02$ & $0.07$ & $\mathbf{0.02}$ &$0.06$ & $0.09$ & $0.07$ & $0.06$\\
& $PCT_{ET}$ &$0.68$ & $0.78$ & $0.71$ & $\mathbf{0.28}$ &$\mathbf{0.46}$ &$\mathbf{0.51}$ &$\mathbf{0.68}$ &$0.78$ & $0.71$ & $\mathbf{0.28}$ &$\mathbf{0.46}$ &$\mathbf{0.51}$\\
& & $\mathbf{0.01}$ &$0.02$ & $\mathbf{0.03}$ &$\mathbf{0.02}$ &$\mathbf{0.02}$ &$\mathbf{0.01}$ &$\mathbf{0.01}$ &$0.02$ & $\mathbf{0.03}$ &$\mathbf{0.02}$ &$\mathbf{0.02}$ &$\mathbf{0.01}$\\
& $PCT_{ROS}$ &$\mathbf{0.7}$ &$0.77$ & $0.71$ & $0.35$ & $0.58$ & $0.54$ & $0.67$ & $\mathbf{0.78}$ &$0.72$ & $0.37$ & $0.59$ & $0.56$\\
& & $0.02$ & $0.04$ & $0.06$ & $0.06$ & $0.09$ & $0.04$ & $0.06$ & $0.05$ & $0.06$ & $0.1$ & $0.11$ & $0.07$\\\hline
& $PCT$ &$0.61$ & $\mathbf{0.67}$ &$\mathbf{0.63}$ &$0.46$ & $0.52$ & $0.53$ & $0.11$ & $0.95$ & $0.96$ & $0.92$ & $0.92$ & $0.93$\\
& & $0.22$ & $0.26$ & $0.35$ & $0.26$ & $0.21$ & $0.16$ & $0.15$ & $0.05$ & $0.06$ & $0.11$ & $0.08$ & $0.09$\\
& $PCT_{Sub}$ &$0.69$ & $0.79$ & $0.68$ & $0.37$ & $0.53$ & $0.54$ & $0.65$ & $0.8$ & $\mathbf{0.7}$ &$0.4$ & $0.55$ & $0.56$\\
3& & $0.02$ & $\mathbf{0.02}$ &$0.05$ & $0.05$ & $0.04$ & $0.02$ & $0.07$ & $0.02$ & $0.06$ & $0.09$ & $0.07$ & $0.06$\\
& $PCT_{ET}$ &$0.68$ & $0.78$ & $0.71$ & $\mathbf{0.27}$ &$\mathbf{0.45}$ &$\mathbf{0.51}$ &$\mathbf{0.68}$ &$0.78$ & $0.71$ & $\mathbf{0.27}$ &$\mathbf{0.45}$ &$\mathbf{0.51}$\\
& & $\mathbf{0.01}$ &$0.02$ & $\mathbf{0.03}$ &$\mathbf{0.02}$ &$\mathbf{0.02}$ &$\mathbf{0.01}$ &$\mathbf{0.01}$ &$\mathbf{0.02}$ &$\mathbf{0.03}$ &$\mathbf{0.02}$ &$\mathbf{0.02}$ &$\mathbf{0.01}$\\
& $PCT_{ROS}$ &$\mathbf{0.7}$ &$0.77$ & $0.72$ & $0.35$ & $0.57$ & $0.54$ & $0.67$ & $\mathbf{0.77}$ &$0.73$ & $0.37$ & $0.58$ & $0.56$\\
& & $0.02$ & $0.04$ & $0.06$ & $0.06$ & $0.09$ & $0.04$ & $0.06$ & $0.05$ & $0.06$ & $0.1$ & $0.11$ & $0.07$\\\hline
& $PCT$ &$0.61$ & $\mathbf{0.67}$ &$\mathbf{0.63}$ &$0.46$ & $0.52$ & $0.53$ & $0.11$ & $0.95$ & $0.96$ & $0.92$ & $0.92$ & $0.93$\\
& & $0.22$ & $0.26$ & $0.35$ & $0.26$ & $0.21$ & $0.16$ & $0.15$ & $0.05$ & $0.06$ & $0.11$ & $0.08$ & $0.09$\\
& $PCT_{Sub}$ &$0.69$ & $0.79$ & $0.68$ & $0.37$ & $0.53$ & $0.54$ & $0.66$ & $0.8$ & $\mathbf{0.69}$ &$0.39$ & $0.55$ & $0.56$\\
4& & $0.02$ & $\mathbf{0.02}$ &$0.05$ & $0.05$ & $0.04$ & $0.02$ & $0.06$ & $\mathbf{0.02}$ &$0.06$ & $0.09$ & $0.07$ & $0.05$\\
& $PCT_{ET}$ &$0.68$ & $0.78$ & $0.71$ & $\mathbf{0.27}$ &$\mathbf{0.45}$ &$\mathbf{0.51}$ &$\mathbf{0.68}$ &$0.78$ & $0.71$ & $\mathbf{0.27}$ &$\mathbf{0.45}$ &$\mathbf{0.51}$\\
& & $\mathbf{0.01}$ &$0.02$ & $\mathbf{0.03}$ &$\mathbf{0.02}$ &$\mathbf{0.02}$ &$\mathbf{0.01}$ &$\mathbf{0.01}$ &$0.02$ & $\mathbf{0.03}$ &$\mathbf{0.02}$ &$\mathbf{0.02}$ &$\mathbf{0.01}$\\
& $PCT_{ROS}$ &$\mathbf{0.7}$ &$0.77$ & $0.71$ & $0.34$ & $0.57$ & $0.54$ & $0.67$ & $\mathbf{0.78}$ &$0.72$ & $0.36$ & $0.58$ & $0.55$\\
& & $0.02$ & $0.04$ & $0.06$ & $0.07$ & $0.1$ & $0.04$ & $0.06$ & $0.05$ & $0.07$ & $0.11$ & $0.11$ & $0.07$\\\hline
& $PCT$ &$0.61$ & $\mathbf{0.67}$ &$\mathbf{0.63}$ &$0.46$ & $0.52$ & $0.53$ & $0.11$ & $0.95$ & $0.96$ & $0.92$ & $0.92$ & $0.93$\\
& & $0.22$ & $0.26$ & $0.35$ & $0.26$ & $0.21$ & $0.16$ & $0.15$ & $0.05$ & $0.06$ & $0.11$ & $0.08$ & $0.09$\\
& $PCT_{Sub}$ &$0.68$ & $0.79$ & $0.68$ & $0.36$ & $0.53$ & $0.54$ & $0.65$ & $0.8$ & $\mathbf{0.69}$ &$0.39$ & $0.55$ & $0.55$\\
5& & $0.02$ & $0.02$ & $0.05$ & $0.05$ & $0.04$ & $0.02$ & $0.06$ & $0.02$ & $0.06$ & $0.09$ & $0.07$ & $0.06$\\
& $PCT_{ET}$ &$0.69$ & $0.77$ & $0.7$ & $\mathbf{0.26}$ &$\mathbf{0.45}$ &$\mathbf{0.5}$ &$0.69$ & $0.77$ & $0.7$ & $\mathbf{0.26}$ &$\mathbf{0.45}$ &$\mathbf{0.5}$\\
& & $0.01$ & $\mathbf{0.02}$ &$\mathbf{0.03}$ &$\mathbf{0.02}$ &$\mathbf{0.03}$ &$\mathbf{0.01}$ &$0.01$ & $\mathbf{0.02}$ &$\mathbf{0.03}$ &$\mathbf{0.02}$ &$\mathbf{0.03}$ &$\mathbf{0.01}$\\
& $PCT_{ROS}$ &$\mathbf{0.7}$ &$0.75$ & $0.71$ & $0.28$ & $0.48$ & $0.5$ & $\mathbf{0.7}$ &$\mathbf{0.75}$ &$0.71$ & $0.28$ & $0.48$ & $0.5$\\
& & $\mathbf{0.01}$ &$0.03$ & $0.04$ & $0.03$ & $0.05$ & $0.01$ & $\mathbf{0.01}$ &$0.03$ & $0.04$ & $0.03$ & $0.05$ & $0.01$\\\hline
& $PCT$ &$0.61$ & $\mathbf{0.67}$ &$\mathbf{0.63}$ &$0.46$ & $0.52$ & $0.53$ & $0.11$ & $0.95$ & $0.96$ & $0.92$ & $0.92$ & $0.93$\\
& & $0.22$ & $0.26$ & $0.35$ & $0.26$ & $0.21$ & $0.16$ & $0.15$ & $0.05$ & $0.06$ & $0.11$ & $0.08$ & $0.09$\\
& $PCT_{Sub}$ &$0.68$ & $0.79$ & $0.68$ & $0.36$ & $0.53$ & $0.54$ & $0.65$ & $0.8$ & $\mathbf{0.69}$ &$0.39$ & $0.55$ & $0.55$\\
6& & $0.02$ & $0.02$ & $0.05$ & $0.05$ & $0.04$ & $0.02$ & $0.06$ & $0.02$ & $0.06$ & $0.09$ & $0.07$ & $0.06$\\
& $PCT_{ET}$ &$0.69$ & $0.77$ & $0.71$ & $\mathbf{0.25}$ &$\mathbf{0.44}$ &$\mathbf{0.5}$ &$0.69$ & $0.77$ & $0.71$ & $\mathbf{0.25}$ &$\mathbf{0.44}$ &$\mathbf{0.5}$\\
& & $\mathbf{0.01}$ &$\mathbf{0.02}$ &$\mathbf{0.02}$ &$\mathbf{0.01}$ &$\mathbf{0.01}$ &$\mathbf{0.01}$ &$\mathbf{0.01}$ &$\mathbf{0.02}$ &$\mathbf{0.02}$ &$\mathbf{0.01}$ &$\mathbf{0.01}$ &$\mathbf{0.01}$\\
& $PCT_{ROS}$ &$\mathbf{0.7}$ &$0.74$ & $0.72$ & $0.28$ & $0.48$ & $0.5$ & $\mathbf{0.7}$ &$\mathbf{0.74}$ &$0.72$ & $0.28$ & $0.48$ & $0.5$\\
& & $0.01$ & $0.03$ & $0.04$ & $0.03$ & $0.05$ & $0.01$ & $0.01$ & $0.03$ & $0.04$ & $0.03$ & $0.05$ & $0.01$\\\hline
& $PCT$ &$0.61$ & $\mathbf{0.67}$ &$\mathbf{0.63}$ &$0.46$ & $0.52$ & $0.53$ & $0.11$ & $0.95$ & $0.96$ & $0.92$ & $0.92$ & $0.93$\\
& & $0.22$ & $0.26$ & $0.35$ & $0.26$ & $0.21$ & $0.16$ & $0.15$ & $0.05$ & $0.06$ & $0.11$ & $0.08$ & $0.09$\\
& $PCT_{Sub}$ &$0.68$ & $0.79$ & $0.68$ & $0.36$ & $0.53$ & $0.54$ & $0.65$ & $0.8$ & $\mathbf{0.69}$ &$0.39$ & $0.55$ & $0.55$\\
7& & $0.02$ & $0.02$ & $0.05$ & $0.05$ & $0.04$ & $0.02$ & $0.06$ & $0.02$ & $0.06$ & $0.09$ & $0.07$ & $0.06$\\
& $PCT_{ET}$ &$0.68$ & $0.77$ & $0.71$ & $\mathbf{0.24}$ &$\mathbf{0.43}$ &$\mathbf{0.49}$ &$0.68$ & $0.77$ & $0.71$ & $\mathbf{0.24}$ &$\mathbf{0.43}$ &$\mathbf{0.49}$\\
& & $\mathbf{0.01}$ &$\mathbf{0.02}$ &$\mathbf{0.02}$ &$\mathbf{0.01}$ &$\mathbf{0.02}$ &$\mathbf{0.0}$ &$\mathbf{0.01}$ &$\mathbf{0.02}$ &$\mathbf{0.02}$ &$\mathbf{0.01}$ &$\mathbf{0.02}$ &$\mathbf{0.0}$\\
& $PCT_{ROS}$ &$\mathbf{0.7}$ &$0.74$ & $0.72$ & $0.28$ & $0.48$ & $0.5$ & $\mathbf{0.7}$ &$\mathbf{0.74}$ &$0.72$ & $0.28$ & $0.48$ & $0.5$\\
& & $0.01$ & $0.03$ & $0.04$ & $0.03$ & $0.05$ & $0.01$ & $0.01$ & $0.03$ & $0.04$ & $0.03$ & $0.05$ & $0.01$\\\hline

\end{longtable}
\end{footnotesize}
\end{center}

\begin{center}
\begin{footnotesize}
\LTcapwidth=\textwidth
\begin{longtable}[c]{|c|c|c|c|c|c|c|c|c|c|c|c|c|c|} % <-- Replaces \begin{table}, alignment must be 
 \caption{Quality of redescription sets produced on the Phenotype dataset using the framework for multi-view redescription mining with a Random Forest supplementing model containing $20$ trees. We denote memory parameters with numbers, $1$ denoting work size of $200$ and maximal memory size of $1700$ and $7$ denoting $3000$, $6000$ memory parameters.}
  \label{tab:Supp3}\\
 \hline
 $M$ & $\mathcal{M}$ & $AJ$ & $Ap_{sc}$ & $AEJ$ &$AAJ$ & $ARC$ & $RSS$& $\underline{AJ}$ & $\underline{Ap_{sc}}$ & $\underline{AEJ}$ & $\underline{AAJ}$ & $\underline{ARC}$ & $\underline{RSS}$ \\  \hline

  \endhead % <--  
& $PCT$ &$0.34$ & $\mathbf{0.36}$ &$\mathbf{0.06}$ &$\mathbf{0.03}$ &$\mathbf{0.16}$ &$\mathbf{0.25}$ &$0.0$ & $0.99$ & $0.99$ & $0.99$ & $0.99$ & $0.99$\\
& & $0.37$ & $0.42$ & $0.12$ & $0.07$ & $0.17$ & $0.09$ & $\mathbf{0.0}$ &$\mathbf{0.0}$ &$\mathbf{0.0}$ &$\mathbf{0.01}$ &$\mathbf{0.0}$ &$\mathbf{0.0}$\\
& $PCT_{Sub}$ &$0.73$ & $0.84$ & $0.61$ & $0.04$ & $0.41$ & $0.43$ & $\mathbf{0.68}$ &$\mathbf{0.85}$ &$\mathbf{0.64}$ &$\mathbf{0.11}$ &$\mathbf{0.45}$ &$\mathbf{0.47}$\\
1& & $0.03$ & $0.03$ & $0.06$ & $\mathbf{0.01}$ &$\mathbf{0.02}$ &$0.01$ & $0.16$ & $0.03$ & $0.08$ & $0.2$ & $0.13$ & $0.12$\\
& $PCT_{ET}$ &$0.72$ & $0.86$ & $0.64$ & $0.07$ & $0.45$ & $0.46$ & $0.35$ & $0.93$ & $0.82$ & $0.54$ & $0.74$ & $0.74$\\
& & $0.03$ & $0.01$ & $0.06$ & $0.04$ & $0.06$ & $\mathbf{0.01}$ &$0.2$ & $0.04$ & $0.09$ & $0.26$ & $0.13$ & $0.14$\\
& $PCT_{ROS}$ &$\mathbf{0.73}$ &$0.86$ & $0.65$ & $0.07$ & $0.44$ & $0.46$ & $0.52$ & $0.9$ & $0.74$ & $0.32$ & $0.6$ & $0.61$\\
& & $\mathbf{0.03}$ &$\mathbf{0.01}$ &$\mathbf{0.06}$ &$0.05$ & $0.04$ & $0.02$ & $0.19$ & $0.04$ & $0.11$ & $0.26$ & $0.14$ & $0.15$\\\hline
& $PCT$ &$0.34$ & $\mathbf{0.36}$ &$\mathbf{0.06}$ &$\mathbf{0.03}$ &$\mathbf{0.16}$ &$\mathbf{0.25}$ &$0.0$ & $0.99$ & $0.99$ & $0.99$ & $0.99$ & $0.99$\\
& & $0.37$ & $0.42$ & $0.12$ & $0.07$ & $0.17$ & $0.09$ & $\mathbf{0.0}$ &$\mathbf{0.0}$ &$\mathbf{0.0}$ &$\mathbf{0.01}$ &$\mathbf{0.0}$ &$\mathbf{0.0}$\\
& $PCT_{Sub}$ &$\mathbf{0.73}$ &$0.84$ & $0.6$ & $0.04$ & $0.41$ & $0.43$ & $\mathbf{0.67}$ &$\mathbf{0.85}$ &$\mathbf{0.64}$ &$\mathbf{0.11}$ &$\mathbf{0.45}$ &$\mathbf{0.48}$\\
2& & $0.03$ & $0.04$ & $0.07$ & $\mathbf{0.01}$ &$\mathbf{0.02}$ &$0.02$ & $0.18$ & $0.03$ & $0.09$ & $0.23$ & $0.15$ & $0.13$\\
& $PCT_{ET}$ &$0.72$ & $0.86$ & $0.64$ & $0.07$ & $0.45$ & $0.46$ & $0.34$ & $0.93$ & $0.83$ & $0.55$ & $0.74$ & $0.74$\\
& & $\mathbf{0.03}$ &$0.02$ & $\mathbf{0.06}$ &$0.04$ & $0.06$ & $\mathbf{0.01}$ &$0.21$ & $0.04$ & $0.1$ & $0.27$ & $0.13$ & $0.15$\\
& $PCT_{ROS}$ &$0.73$ & $0.86$ & $0.65$ & $0.07$ & $0.44$ & $0.46$ & $0.52$ & $0.9$ & $0.74$ & $0.33$ & $0.6$ & $0.61$\\
& & $0.03$ & $\mathbf{0.01}$ &$0.06$ & $0.05$ & $0.04$ & $0.02$ & $0.2$ & $0.04$ & $0.11$ & $0.27$ & $0.15$ & $0.15$\\\hline
& $PCT$ &$0.34$ & $\mathbf{0.36}$ &$\mathbf{0.06}$ &$\mathbf{0.03}$ &$\mathbf{0.16}$ &$\mathbf{0.25}$ &$0.0$ & $0.99$ & $0.99$ & $0.99$ & $0.99$ & $0.99$\\
& & $0.37$ & $0.42$ & $0.12$ & $0.07$ & $0.17$ & $0.09$ & $\mathbf{0.0}$ &$\mathbf{0.0}$ &$\mathbf{0.0}$ &$\mathbf{0.01}$ &$\mathbf{0.0}$ &$\mathbf{0.0}$\\
& $PCT_{Sub}$ &$0.73$ & $0.84$ & $0.6$ & $0.04$ & $0.41$ & $0.43$ & $\mathbf{0.67}$ &$\mathbf{0.85}$ &$\mathbf{0.64}$ &$\mathbf{0.11}$ &$\mathbf{0.45}$ &$\mathbf{0.48}$\\
3& & $0.03$ & $0.03$ & $0.07$ & $\mathbf{0.01}$ &$\mathbf{0.02}$ &$0.02$ & $0.17$ & $0.03$ & $0.09$ & $0.22$ & $0.14$ & $0.13$\\
& $PCT_{ET}$ &$0.72$ & $0.86$ & $0.64$ & $0.07$ & $0.44$ & $0.46$ & $0.35$ & $0.93$ & $0.83$ & $0.54$ & $0.74$ & $0.74$\\
& & $0.03$ & $0.02$ & $0.06$ & $0.04$ & $0.05$ & $\mathbf{0.01}$ &$0.23$ & $0.04$ & $0.11$ & $0.29$ & $0.15$ & $0.16$\\
& $PCT_{ROS}$ &$\mathbf{0.73}$ &$0.86$ & $0.65$ & $0.07$ & $0.44$ & $0.46$ & $0.48$ & $0.9$ & $0.76$ & $0.38$ & $0.63$ & $0.64$\\
& & $\mathbf{0.02}$ &$\mathbf{0.01}$ &$\mathbf{0.05}$ &$0.05$ & $0.04$ & $0.02$ & $0.2$ & $0.04$ & $0.1$ & $0.27$ & $0.16$ & $0.15$\\\hline
& $PCT$ &$0.34$ & $\mathbf{0.36}$ &$\mathbf{0.06}$ &$\mathbf{0.03}$ &$\mathbf{0.16}$ &$\mathbf{0.25}$ &$0.0$ & $0.99$ & $0.99$ & $0.99$ & $0.99$ & $0.99$\\
& & $0.37$ & $0.42$ & $0.12$ & $0.07$ & $0.17$ & $0.09$ & $\mathbf{0.0}$ &$\mathbf{0.0}$ &$\mathbf{0.0}$ &$\mathbf{0.01}$ &$\mathbf{0.0}$ &$\mathbf{0.0}$\\
& $PCT_{Sub}$ &$0.73$ & $0.84$ & $0.6$ & $0.04$ & $0.4$ & $0.43$ & $\mathbf{0.67}$ &$\mathbf{0.85}$ &$\mathbf{0.64}$ &$\mathbf{0.11}$ &$\mathbf{0.45}$ &$\mathbf{0.48}$\\
4& & $0.03$ & $0.03$ & $0.06$ & $\mathbf{0.01}$ &$\mathbf{0.02}$ &$0.02$ & $0.17$ & $0.03$ & $0.09$ & $0.22$ & $0.14$ & $0.13$\\
& $PCT_{ET}$ &$0.72$ & $0.86$ & $0.64$ & $0.06$ & $0.45$ & $0.46$ & $0.33$ & $0.93$ & $0.83$ & $0.57$ & $0.75$ & $0.75$\\
& & $0.03$ & $0.01$ & $0.05$ & $0.03$ & $0.05$ & $\mathbf{0.01}$ &$0.19$ & $0.03$ & $0.1$ & $0.25$ & $0.13$ & $0.14$\\
& $PCT_{ROS}$ &$\mathbf{0.73}$ &$0.86$ & $0.65$ & $0.07$ & $0.44$ & $0.46$ & $0.48$ & $0.9$ & $0.76$ & $0.38$ & $0.62$ & $0.64$\\
& & $\mathbf{0.02}$ &$\mathbf{0.01}$ &$\mathbf{0.05}$ &$0.03$ & $0.04$ & $0.01$ & $0.2$ & $0.04$ & $0.1$ & $0.26$ & $0.16$ & $0.15$\\\hline
& $PCT$ &$0.34$ & $\mathbf{0.36}$ &$\mathbf{0.06}$ &$\mathbf{0.03}$ &$\mathbf{0.16}$ &$\mathbf{0.25}$ &$0.0$ & $0.99$ & $0.99$ & $0.99$ & $0.99$ & $0.99$\\
& & $0.37$ & $0.42$ & $0.12$ & $0.07$ & $0.17$ & $0.09$ & $\mathbf{0.0}$ &$\mathbf{0.0}$ &$\mathbf{0.0}$ &$\mathbf{0.01}$ &$\mathbf{0.0}$ &$\mathbf{0.0}$\\
& $PCT_{Sub}$ &$\mathbf{0.73}$ &$0.84$ & $0.6$ & $0.04$ & $0.4$ & $0.43$ & $\mathbf{0.67}$ &$\mathbf{0.85}$ &$\mathbf{0.64}$ &$\mathbf{0.11}$ &$\mathbf{0.45}$ &$\mathbf{0.47}$\\
5& & $0.03$ & $0.03$ & $0.06$ & $\mathbf{0.01}$ &$\mathbf{0.02}$ &$0.02$ & $0.17$ & $0.03$ & $0.09$ & $0.23$ & $0.14$ & $0.13$\\
& $PCT_{ET}$ &$0.72$ & $0.86$ & $0.64$ & $0.06$ & $0.45$ & $0.46$ & $0.36$ & $0.93$ & $0.82$ & $0.53$ & $0.73$ & $0.73$\\
& & $0.03$ & $0.01$ & $0.05$ & $0.04$ & $0.05$ & $\mathbf{0.01}$ &$0.23$ & $0.04$ & $0.12$ & $0.3$ & $0.16$ & $0.17$\\
& $PCT_{ROS}$ &$0.72$ & $0.86$ & $0.65$ & $0.07$ & $0.43$ & $0.46$ & $0.51$ & $0.9$ & $0.74$ & $0.34$ & $0.59$ & $0.61$\\
& & $\mathbf{0.03}$ &$\mathbf{0.01}$ &$\mathbf{0.05}$ &$0.03$ & $0.05$ & $0.01$ & $0.19$ & $0.04$ & $0.1$ & $0.26$ & $0.16$ & $0.15$\\\hline
& $PCT$ &$0.34$ & $\mathbf{0.36}$ &$\mathbf{0.06}$ &$\mathbf{0.03}$ &$\mathbf{0.16}$ &$\mathbf{0.25}$ &$0.0$ & $0.99$ & $0.99$ & $0.99$ & $0.99$ & $0.99$\\
& & $0.37$ & $0.42$ & $0.12$ & $0.07$ & $0.17$ & $0.09$ & $\mathbf{0.0}$ &$\mathbf{0.0}$ &$\mathbf{0.0}$ &$\mathbf{0.01}$ &$\mathbf{0.0}$ &$\mathbf{0.0}$\\
& $PCT_{Sub}$ &$\mathbf{0.73}$ &$0.84$ & $0.6$ & $0.04$ & $0.4$ & $0.43$ & $\mathbf{0.67}$ &$\mathbf{0.85}$ &$\mathbf{0.64}$ &$\mathbf{0.11}$ &$\mathbf{0.45}$ &$\mathbf{0.47}$\\
6& & $0.03$ & $0.03$ & $0.06$ & $\mathbf{0.01}$ &$\mathbf{0.02}$ &$0.02$ & $0.17$ & $0.03$ & $0.09$ & $0.23$ & $0.14$ & $0.13$\\
& $PCT_{ET}$ &$0.72$ & $0.86$ & $0.64$ & $0.06$ & $0.45$ & $0.46$ & $0.36$ & $0.93$ & $0.82$ & $0.53$ & $0.73$ & $0.73$\\
& & $0.03$ & $0.01$ & $0.05$ & $0.03$ & $0.05$ & $\mathbf{0.01}$ &$0.23$ & $0.04$ & $0.12$ & $0.3$ & $0.16$ & $0.17$\\
& $PCT_{ROS}$ &$0.72$ & $0.86$ & $0.65$ & $0.07$ & $0.43$ & $0.46$ & $0.51$ & $0.9$ & $0.74$ & $0.34$ & $0.59$ & $0.61$\\
& & $\mathbf{0.03}$ &$\mathbf{0.01}$ &$\mathbf{0.05}$ &$0.03$ & $0.05$ & $0.01$ & $0.19$ & $0.04$ & $0.1$ & $0.26$ & $0.16$ & $0.15$\\\hline
& $PCT$ &$0.34$ & $\mathbf{0.36}$ &$\mathbf{0.06}$ &$\mathbf{0.03}$ &$\mathbf{0.16}$ &$\mathbf{0.25}$ &$0.0$ & $0.99$ & $0.99$ & $0.99$ & $0.99$ & $0.99$\\
& & $0.37$ & $0.42$ & $0.12$ & $0.07$ & $0.17$ & $0.09$ & $\mathbf{0.0}$ &$\mathbf{0.0}$ &$\mathbf{0.0}$ &$\mathbf{0.01}$ &$\mathbf{0.0}$ &$\mathbf{0.0}$\\
& $PCT_{Sub}$ &$\mathbf{0.73}$ &$0.84$ & $0.6$ & $0.04$ & $0.4$ & $0.43$ & $\mathbf{0.67}$ &$\mathbf{0.85}$ &$\mathbf{0.63}$ &$\mathbf{0.11}$ &$\mathbf{0.45}$ &$\mathbf{0.47}$\\
7& & $0.03$ & $0.03$ & $0.06$ & $\mathbf{0.01}$ &$\mathbf{0.02}$ &$0.02$ & $0.17$ & $0.03$ & $0.09$ & $0.23$ & $0.14$ & $0.13$\\
& $PCT_{ET}$ &$0.72$ & $0.86$ & $0.64$ & $0.06$ & $0.45$ & $0.46$ & $0.36$ & $0.93$ & $0.82$ & $0.53$ & $0.73$ & $0.73$\\
& & $\mathbf{0.03}$ &$0.01$ & $\mathbf{0.05}$ &$0.03$ & $0.05$ & $\mathbf{0.01}$ &$0.23$ & $0.04$ & $0.12$ & $0.3$ & $0.16$ & $0.17$\\
& $PCT_{ROS}$ &$0.72$ & $0.86$ & $0.65$ & $0.07$ & $0.43$ & $0.46$ & $0.51$ & $0.9$ & $0.74$ & $0.34$ & $0.59$ & $0.61$\\
& & $0.03$ & $\mathbf{0.01}$ &$0.05$ & $0.03$ & $0.05$ & $0.01$ & $0.19$ & $0.04$ & $0.1$ & $0.26$ & $0.16$ & $0.15$\\\hline

\end{longtable}
\end{footnotesize}
\end{center}

We can see from results presented in Tables \ref{tab:Supp1}, \ref{tab:Supp2} and \ref{tab:Supp3} that multi-view framework with supplementing model containing Random forest with $20$ trees behaves similarly as this model with $50$ trees, presented in the main manuscript. The best performance on a World Country dataset (see Table \ref{tab:Supp1}) is achieved when using ROS in a supplementing model, although performance is divided between random attribute subspace selection (Sub) and ROS. On Slovenian Water dataset (see Table \ref{tab:Supp2}), the framework for multi-view redescription mining achieves the best performance when used in combination with a supplementing model consisting of Extra trees, whereas on Phenotype dataset (see Table \ref{tab:Supp3}) the framework using random attribute subspace selection in the supplementing model outperforms other approaches. Again, PCT model has lower scores with respect to many measures due to a small number of produced redescriptions, but the true difference is visible in $\underline{score}$ scores which take the deviation in number of produced redescriptions from the user-defined number into account. With the exception of Slovenian Water dataset (on several intervals), the framework achieves worse performance scores with $20$ trees than with $50$ trees.  

The corresponding comparative plot of a total redescription score $\underline{R_{score}}$ achieved using $20$ trees can be seen in Figure \ref{fig:SM}.

\begin{figure}[H]
\centerline{\includegraphics[width=1.0\textwidth]{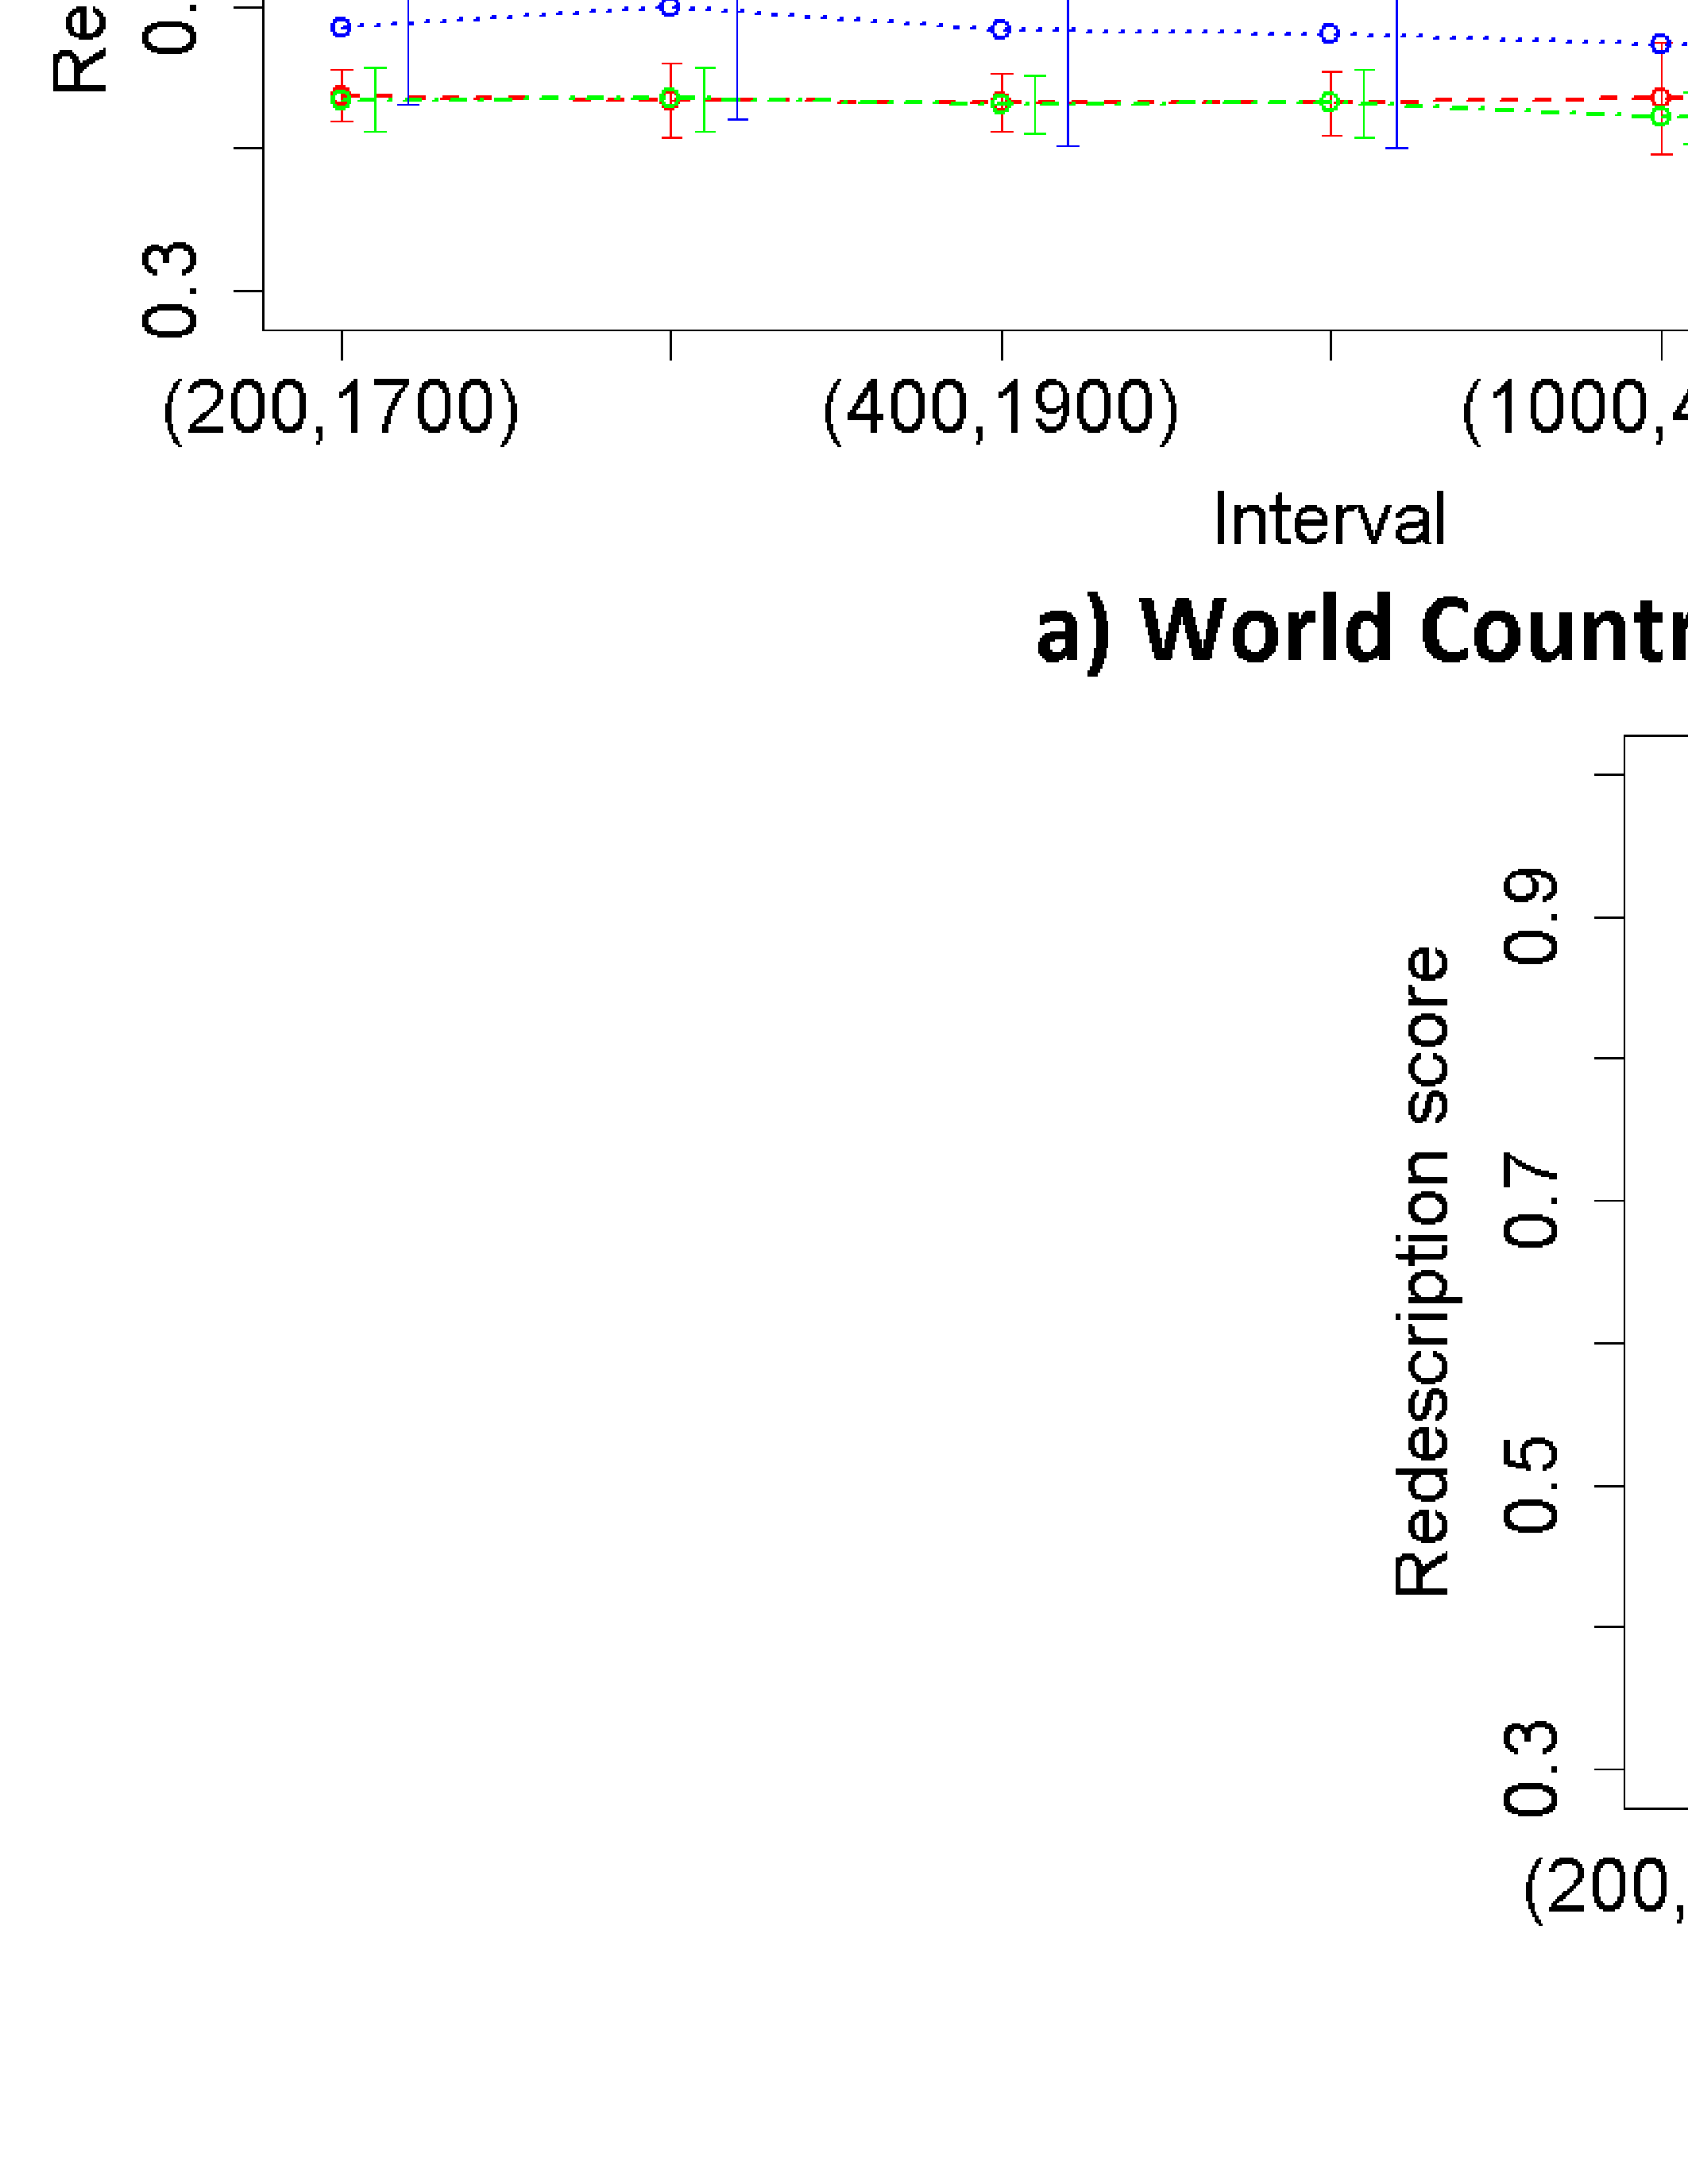}}\caption{Overall redescription set score $\underline{total_{sc}}(\mathcal{R})$ obtained using a single rule-generating PCT model and a supplementing model containing $20$ trees with different memory parameters.}
\label{fig:SM}
\end{figure}

\subsection{Extra trees as a main rule generation model}

In this section, we consider the overall performance of a framework for multi-view redescription mining when using one or more Extra multi-target PCTs as a main rule-generating model as compared to using one Predictive Clustering tree as a main rule-generating model.

The experiments presented in Table \ref{tab:ETGen} demonstrate that using a few Extra multi-target PCTs as the main rule-generating model in the proposed multi-view redescription mining framework can significantly outperform using one main rule-generating PCT model. Using the Extra multi-target PCTs as a main rule-generating model increases the overall performance, accuracy, diversity and the number of produced redescriptions (given a set of predefined constraints defined in Section VII of the main manuscript). This is visible from the $\underline{underline}$ scores and corresponding standard deviations. Since a PCT and $ET_{1T},\ ET_{2T}$ models often produce empty redescription sets (having $0$ score for all measures), the average score across $10$ runs is unrealistically small. On the Country dataset, the difference is visible when using $4$ or more Extra multi-target PCTs as the main rule-generating model, on the Slovenian Water dataset the difference is already visible when using one Extra multi-target PCTs, whereas on the Phenotype dataset this difference is visible when using $4$ or more Extra multi-target PCTs as a main rule-generating model. The obtained results are important, since using Extra multi-target PCTs as a main-rule generating model reduces the overall computational complexity of the framework (see Section V of the main manuscript). Since favourable results are achieved using a small number of Extra multi-target PCTs, it might be advantageous to use them instead of PCTs on datasets containing a large number of entities. Given the fact that learning multiple Extra multi-target PCTs in parallel can be achieved easily on any modern PC, the overall gain can be substantial.

\begin{center}
\begin{footnotesize}
\LTcapwidth=\textwidth
\begin{longtable}[c]{|c|c|c|c|c|c|c|c|c|c|c|c|c|c|} % <-- Replaces \begin{table}, alignment must be 
 \caption{The framework's performance using one main PCT rule-generating model compared to using $1,\ 2,\ 4$ or $6$ Extra multi-target PCTs as a main rule-generating model. A working set size of at most $3000$ and a maximal memory size of $6000$ are used in all experiments.}
  \label{tab:ETGen}\\
 \hline
 $\mathcal{D}$ & $\mathcal{M}$ & $AJ$ & $Ap_{sc}$ & $AEJ$ &$AAJ$ & $ARC$ & $RSS$& $\underline{AJ}$ & $\underline{Ap_{sc}}$ & $\underline{AEJ}$ & $\underline{AAJ}$ & $\underline{ARC}$ & $\underline{RSS}$ \\  \hline
 
   \endfirsthead

\multicolumn{14}{c}%
        {{\textbf{Table \thetable\ } Continued from previous page}} \\
        \hline 
 $\mathcal{D}$ & $\mathcal{M}$ & $AJ$ & $Ap_{sc}$ & $AEJ$ &$AAJ$ & $ARC$ & $RSS$& $\underline{AJ}$ & $\underline{Ap_{sc}}$ & $\underline{AEJ}$ & $\underline{AAJ}$ & $\underline{ARC}$ & $\underline{RSS}$ \\  \hline 
 
  \endhead % <--  
& $PCT$ &$0.71$ & $0.35$ &$0.74$ &$0.29$ & $0.70$ &$0.47$ &$0.49$ & $0.56$ & $0.82$ & $0.50$ & $\mathbf{0.80}$ & $0.64$\\
& & $0.03$ & $0.11$ & $0.11$ & $0.10$ & $0.07$ & $0.05$ & $0.27$ &$0.26$ &$0.11$ &$0.29$ & $0.11$ &$0.20$\\
& $ET_{1T}$ &$0.07$ &$\mathbf{0.04}$ & $\mathbf{0.09}$ & $\mathbf{0.06}$ &$\mathbf{0.08}$ & $\mathbf{0.24}$ & $0.01$ &$0.99$ &$0.99$ &$0.99$ &$0.99$ &$0.99$\\
C& & $0.21$ &$0.14$ & $0.29$ & $0.18$ &$0.27$ &$0.13$ & $0.03$ & $\mathbf{0.03}$ & $\mathbf{0.0}$ & $0.02$ &$\mathbf{0.01}$ & $0.02$\\
& $ET_{2T}$ &$0.42$ & $0.34$ & $0.36$ & $0.18$ & $0.49$ & $0.39$ & $0.10$ & $0.93$ & $0.96$ & $0.90$ & $0.98$ & $0.93$\\
& & $0.36$ & $0.30$ &$0.38$ &$0.20$ & $0.43$ & $0.17$ &$0.22$ & $0.15$ & $0.09$ & $0.22$ & $0.04$ & $0.14$\\
& $ET_{4T}$ &$0.71$ & $0.36$ & $0.74$ & $0.16$ & $0.83$ & $0.48$ & $0.69$ & $0.37$ & $0.75$ & $0.19$ & $0.84$ & $0.49$\\
& & $0.02$ & $0.11$ & $\mathbf{0.01}$ & $0.03$ & $0.06$ & $0.03$ & $0.08$ & $0.14$ & $0.08$ & $0.09$ & $0.07$ & $0.06$\\
& $ET_{6T}$ &$\mathbf{0.75}$ & $0.32$ & $0.70$ & $0.13$ & $0.81$ & $0.44$ & $\mathbf{0.75}$ & $\mathbf{0.32}$ & $\mathbf{0.70}$ & $\mathbf{0.13}$ & $0.81$ & $\mathbf{0.44}$\\
& & $\mathbf{0.01}$ & $\mathbf{0.05}$ & $0.06$ & $\mathbf{0.01}$ & $\mathbf{0.05}$ & $\mathbf{0.02}$ & $\mathbf{0.01}$ & $0.05$ & $0.06$ & $\mathbf{0.01}$ & $0.05$ & $\mathbf{0.02}$\\\hline
& $PCT$ &$0.61$ & $\mathbf{0.67}$ &$\mathbf{0.63}$ &$0.46$ & $0.52$ &$0.53$ &$0.11$ & $0.95$ & $0.96$ & $0.92$ & $0.92$ & $0.93$\\
& & $0.22$ & $0.26$ & $0.35$ & $0.26$ & $0.21$ & $0.16$ & $0.15$ &$0.05$ &$0.06$ &$0.11$ & $0.08$ &$0.09$\\
& $ET_{1T}$ &$0.66$ &$0.80$ & $0.84$ & $0.49$ &$0.45$ & $0.58$ & $0.34$ &$0.89$ &$0.91$ &$0.71$ &$0.7$ &$0.77$\\
W& & $0.01$ &$0.04$ & $0.05$ & $0.10$ &$0.04$ &$0.03$ & $0.23$ & $0.08$ & $0.06$ & $0.20$ &$0.21$ & $0.15$\\
& $ET_{2T}$ &$0.67$ & $0.78$ & $0.77$ & $0.37$ & $0.45$ & $0.54$ & $0.63$ & $0.79$ & $0.78$ & $0.41$ & $0.48$ & $0.57$\\
& & $0.01$ & $0.03$ &$0.02$ &$0.04$ & $0.03$ & $0.02$ &$0.10$ & $0.05$ & $0.05$ & $0.11$ & $0.09$ & $0.08$\\
& $ET_{4T}$ &$0.68$ & $0.73$ & $0.73$ & $0.30$ & $0.45$ & $0.51$ & $0.68$ & $0.73$ & $0.73$ & $0.30$ & $0.45$ & $0.51$\\
& & $0.01$ & $0.03$ & $0.02$ & $0.03$ & $\mathbf{0.02}$ & $0.01$ & $0.01$ & $0.02$ & $0.03$ & $0.03$ & $\mathbf{0.02}$ & $0.01$\\
& $ET_{6T}$ &$\mathbf{0.68}$ & $0.70$ & $0.73$ & $\mathbf{0.27}$ & $\mathbf{0.42}$ & $\mathbf{0.49}$ & $\mathbf{0.68}$ & $\mathbf{0.70}$ & $\mathbf{0.73}$ & $\mathbf{0.27}$ & $\mathbf{0.42}$ & $\mathbf{0.49}$\\
& & $\mathbf{0.01}$ & $\mathbf{0.02}$ & $\mathbf{0.02}$ & $\mathbf{0.02}$ & $0.02$ & $\mathbf{0.01}$ & $\mathbf{0.01}$ & $\mathbf{0.02}$ & $\mathbf{0.02}$ & $\mathbf{0.02}$ & $0.02$ & $\mathbf{0.01}$\\
\hline
& $PCT$ &$0.54$ & $0.63$ &$0.44$ &$0.26$ & $0.37$ &$0.43$ &$0.03$ & $0.99$ & $0.97$ & $0.96$ & $0.97$ & $0.97$\\
& & $0.24$ & $0.35$ & $0.25$ & $0.17$ & $0.15$ & $0.16$ & $0.03$ &$0.01$ &$0.02$ &$0.04$ &$0.03$ &$0.03$\\
& $ET_{1T}$ &$0.12$ &$\mathbf{0.17}$ & $\mathbf{0.07}$ & $\mathbf{0.03}$ &$\mathbf{0.08}$ & $\mathbf{0.25}$ & $0.0$ &$0.99$ &$0.99$ &$0.99$ &$0.99$ &$0.99$\\
P& & $0.25$ &$0.36$ & $0.24$ & $0.10$ &$0.17$ &$0.11$ & $\mathbf{0.01}$ & $\mathbf{0.0}$ & $\mathbf{0.0}$ & $0.01$ & $0.01$ & $0.01$\\
& $ET_{2T}$ &$0.44$ & $0.70$ & $0.28$ & $0.12$ & $0.30$ & $0.39$ & $0.01$ & $0.99$ & $0.99$ & $0.98$ & $0.99$ & $0.99$\\
& & $0.25$ & $0.37$ &$0.26$ &$0.13$ & $0.22$ & $0.12$ & $0.01$ & $0.0$ & $0.01$ & $0.01$ & $\mathbf{0.01}$ & $0.01$\\
& $ET_{4T}$ &$\mathbf{0.62}$ & $0.87$ & $0.61$ & $0.11$ & $0.49$ & $0.49$ & $0.30$ & $0.93$ & $0.82$ & $0.58$ & $0.78$ & $0.76$\\
& & $0.07$ & $0.0$ & $0.06$ & $0.04$ & $0.12$ & $0.03$ &$0.18$ & $0.03$ & $0.09$ & $0.23$ & $0.10$ & $0.12$\\
& $ET_{6T}$ &$0.61$ & $0.86$ & $0.50$ & $0.05$ & $0.45$ & $0.45$ & $\mathbf{0.61}$ & $\mathbf{0.86}$ & $\mathbf{0.50}$ & $\mathbf{0.05}$ & $\mathbf{0.45}$ & $\mathbf{0.45}$\\
& & $\mathbf{0.03}$ & $\mathbf{0.0}$ & $\mathbf{0.03}$ & $\mathbf{0.0}$ & $\mathbf{0.02}$ & $\mathbf{0.0}$ &$0.03$ & $0.0$ & $0.03$ & $\mathbf{0.0}$ & $0.02$ & $\mathbf{0.0}$\\
\hline
\end{longtable}
\end{footnotesize}
\end{center}  

\subsection{View random subset projections}
The proposed framework applies the CLUS-RM algorithm to each pair of available views and then completes the obtained incomplete redescriptions using rules produced on the remaining views. Although less computationally complex than the naive generalization of redescription mining algorithms, this approach requires performing $n \choose 2$ CLUS-RM applications and the same number of redescription completions (where $n$ denotes the number of available views). We test how much is lost by using and completing only a fixed size subset of pairs of initial views - performing random view subset projection. In the experiments performed to obtain results presented in Table \ref{tab:RSProj}, we used $2$ pairs of initial views to create redescriptions. Thus, performing such a random view subset projection executes $3$ times faster on the World Country dataset and $33\%$ faster on the Slovenian Water and the Phenotype dataset as compared to a regular run of the multi-view redescription mining framework.

The results presented in Table \ref{tab:RSProj} show that, expectedly the full run of the multi-view redescription mining framework outperforms the random view subset projection runs. However, the difference in average redescription set score (after performing $10$ runs) is $0.1$ ($10\%$ of redescription set score range, or full run obtains a set that has $\sim 18\%$ better score than obtained by projection) on the World Country dataset, $0.06$ ($6\%$ of redescription set score range, or $\sim 7\%$ better) on the Slovenian Water dataset and $0.01$ ($1\%$ of redescription set score range, or $\sim 3\%$ better) on the Phenotype dataset. Higher deviation between runs when using projection (approx. $2\times$ on Country, $5\times$ on Water and almost identical on Phenotype dataset) must be taken into account. However, if multiple runs are used, as was done in this experiment (to reduce the effects of  deviation), random view subspace projection may  be used as a technique to alleviate the curse of dimensionality in multi-view redescription mining.

\begin{center}
\begin{footnotesize}
\LTcapwidth=\textwidth
\begin{longtable}[c]{|c|c|c|c|c|c|c|c|c|c|c|c|c|c|} % <-- Replaces \begin{table}, alignment must be 
 \caption{The evaluation of redescription sets created using two pairs of initial views on the World Country (C), Water Quality (W) and Phenotype (P) datasets.}
  \label{tab:RSProj}\\
 \hline
 $\mathcal{D}$ & $\mathcal{M}$ & $AJ$ & $Ap_{sc}$ & $AEJ$ &$AAJ$ & $ARC$ & $RSS$& $\underline{AJ}$ & $\underline{Ap_{sc}}$ & $\underline{AEJ}$ & $\underline{AAJ}$ & $\underline{ARC}$ & $\underline{RSS}$ \\  \hline
  \endhead % <--  
& $PCT_{full}$ &$\mathbf{0.72}$ & $0.24$ &$0.67$ &$\mathbf{0.19}$ & $0.70$ &$0.42$ &$\mathbf{0.67}$ & $\mathbf{0.29}$ & $\mathbf{0.69}$ & $\mathbf{0.24}$ & $\mathbf{0.71}$ & $\mathbf{0.45}$\\
C & & $\mathbf{0.02}$ & $\mathbf{0.10}$ & $\mathbf{0.07}$ & $\mathbf{0.03}$ & $\mathbf{0.06}$ & $\mathbf{0.03}$ & $\mathbf{0.15}$ &$\mathbf{0.20}$ &$\mathbf{0.09}$ &$\mathbf{0.18}$ & $\mathbf{0.09}$ &$\mathbf{0.13}$\\
& $PCT_{proj}$ &$0.62$ &$\mathbf{0.23}$ & $\mathbf{0.62}$ & $0.24$ &$\mathbf{0.51}$ & $\mathbf{0.40}$ & $0.54$ &$0.40$ &$0.79$ &$0.42$ &$0.66$ &$0.55$\\
& & $0.22$ &$0.15$ & $0.28$ & $0.10$ &$0.19$ &$0.09$ & $0.28$ & $0.34$ & $0.14$ & $0.30$ &$0.18$ & $0.24$\\\hline
& $PCT_{full}$ &$\mathbf{0.68}$ & $0.80$ & $\mathbf{0.64}$ & $\mathbf{0.38}$ & $0.57$ & $0.54$ & $\mathbf{0.68}$ & $0.80$ & $\mathbf{0.64}$ & $\mathbf{0.38}$ & $0.57$ & $\mathbf{0.54}$\\
W & & $\mathbf{0.02}$ & $\mathbf{0.04}$ &$\mathbf{0.05}$ &$\mathbf{0.07}$ & $\mathbf{0.05}$ & $\mathbf{0.03}$ &$\mathbf{0.02}$ & $\mathbf{0.04}$ & $\mathbf{0.05}$  & $\mathbf{0.07}$ & $\mathbf{0.05}$ & $\mathbf{0.03}$\\
& $PCT_{proj}$ &$0.62$ & $\mathbf{0.76}$ & $0.66$ & $0.40$ & $\mathbf{0.50}$ & $\mathbf{0.54}$ & $0.57$ & $\mathbf{0.78}$ & $0.68$ & $0.44$ & $\mathbf{0.55}$ & $0.58$\\
& & $0.05$ & $0.06$ & $0.08$ & $0.08$ & $0.08$ & $0.04$ & $0.20$ & $0.09$ & $0.13$ & $0.20$ & $0.17$ & $0.15$\\\hline
& $PCT_{full}$ &$\mathbf{0.21}$ & $\mathbf{0.77}$ & $\mathbf{0.10}$ & $\mathbf{0.04}$ & $0.40$ & $\mathbf{0.42}$ & $\mathbf{0.21}$ & $\mathbf{0.77}$ & $\mathbf{0.10}$ & $\mathbf{0.04}$ & $0.40$ & $\mathbf{0.42}$\\
P & & $0.03$ & $\mathbf{0.02}$ & $\mathbf{0.01}$ & $\mathbf{0.01}$ & $0.03$ & $\mathbf{0.01}$ & $0.03$ & $\mathbf{0.02}$ & $\mathbf{0.01}$ & $\mathbf{0.01}$ & $0.03$ & $\mathbf{0.01}$\\
& $PCT_{proj}$ &$0.18$ & $0.78$ &$0.12$ &$0.07$ & $\mathbf{0.37}$ &$0.43$ &$0.18$ & $0.78$ & $0.12$ & $0.07$ & $\mathbf{0.37}$ & $0.43$\\
& & $\mathbf{0.03}$ & $0.03$ & $0.02$ & $0.03$ & $\mathbf{0.02}$ & $0.01$ & $0.03$ &$0.03$ &$0.02$ &$\mathbf{0.03}$ & $\mathbf{0.02}$ &$0.01$\\\hline
\end{longtable}
\end{footnotesize}
\end{center}

\section{Effects of iterations and memory constraints on redescription set quality}

We study the effects of increasing the number of iterations inside the GCLUS-RM algorithm on the difference in redescription set quality when different memory setting is used during redescription construction.

\begin{figure}[H]
\centerline{\includegraphics[width=1.0\textwidth]{Figures/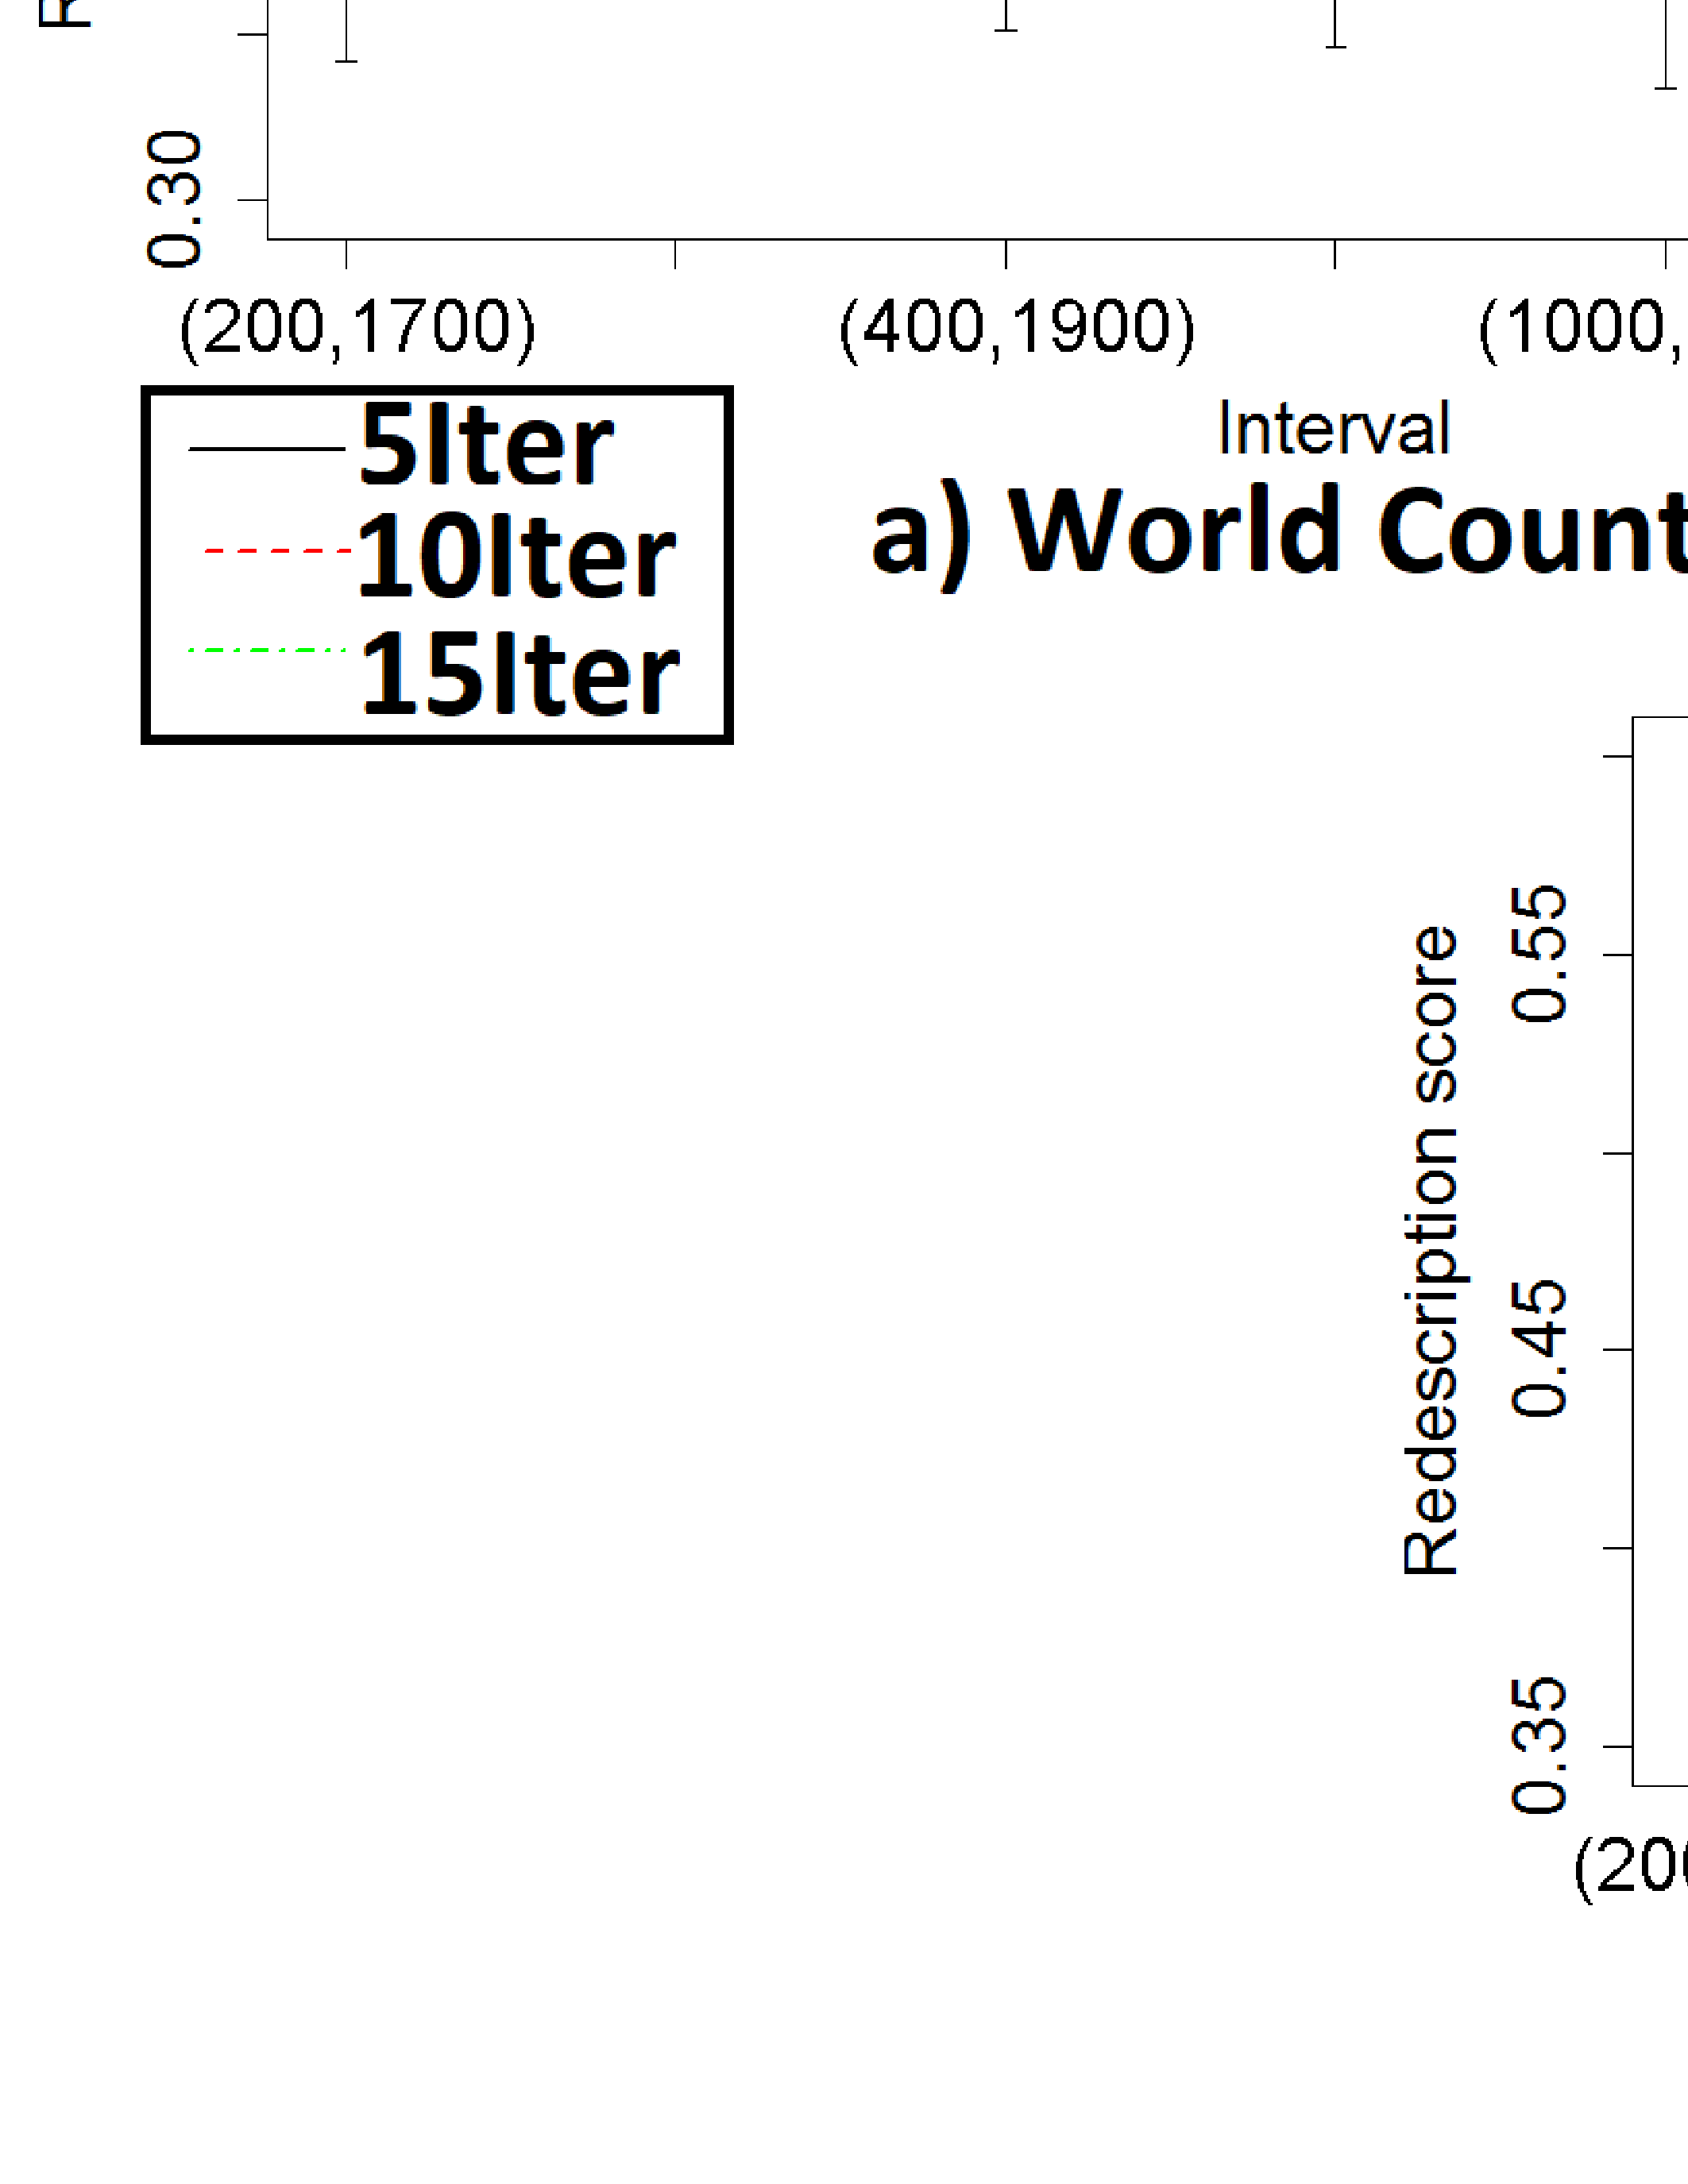}}\caption{Overall redescription set score $\underline{total_{sc}}(\mathcal{R})$ obtained using a single rule-generating PCT model with different memory parameters and different number of iterations of the GCLUS-RM algorithm.}
\label{fig:IterVsMem}
\end{figure}

We use the same parameters as to perform the experiments with a single generating PCT (presented in the main manuscript, see Table $2.$ QP/VRSP) but change the number of iterations used to create (incomplete) two-view redescriptions in the GCLUS-RM algorithm.

As it can be seen from Figure \ref{fig:IterVsMem}, increasing the number of iterations inside the GCLUS-RM algorithm mostly improves the overall performance of the framework. The only exception is the Slovenian Water dataset where the framework performed better using $10$ iterations than $15$ iterations. This can happen when higher number of produced patters (due to higher number of iterations) necessitates multiple consecutive calls of the generalized redescription set procedure. Although there is quite high standard deviation on the Slovenian Water dataset even with $10$ or $15$ iterations of the GCLUS-RM algorithm. The difference in accuracy is statistically significant, according to one-sided Wilcoxon signed-rank test \cite{Wilcoxon1992}, between the first ($200,\ 1700$) and the last ($3000,\ 6000$) memory configuration on the Country dataset with $10$ ($p=9.77\cdot 10^{-4}$) and $15$ ($p=0.0244$) iterations and on the Phenotype dataset with $10$ ($p=0.049$), $15$ ($p=0.032$) and $20$ ($p=0.003$) iterations. Although the difference is not significant on the Slovenian Water datset, increasing the number of iterations increases the difference in accuracy between the first and the last memory configuration.

%\begin{figure}[H]
%\begin{center}
% \includegraphics[width=0.75\linewidth]{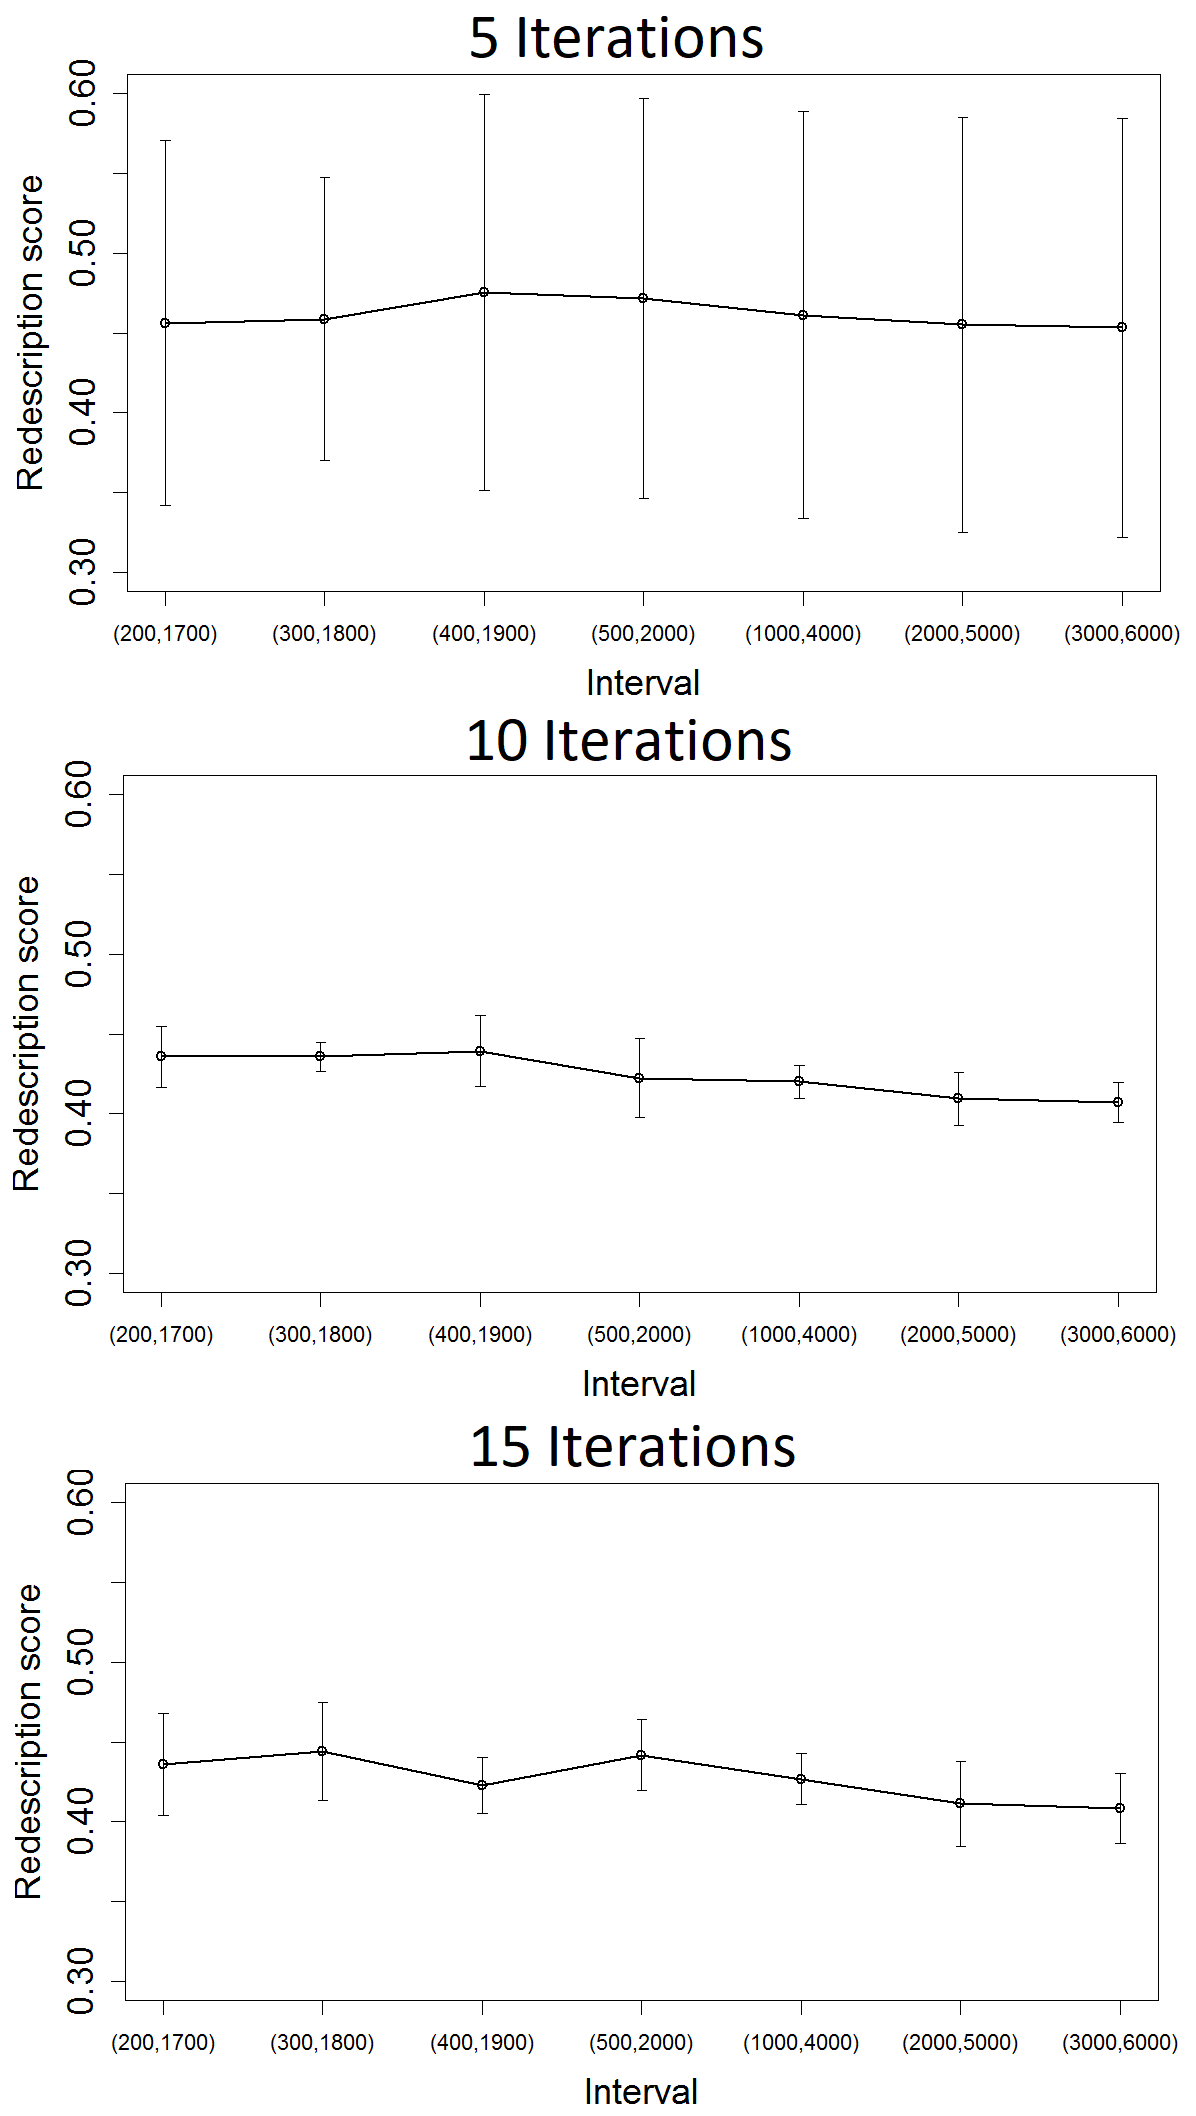}
% \end{center}  
%\caption{Overall score \underline{$\mathcal{R}_{score}$} using different number of iterations inside the GCLUS-RM algorithm and different memory intervals on the Country dataset.}
%\label{fig:MItCountry}
%\end{figure}
%
%\begin{figure}[H]
%\begin{center}
% \includegraphics[width=0.75\linewidth]{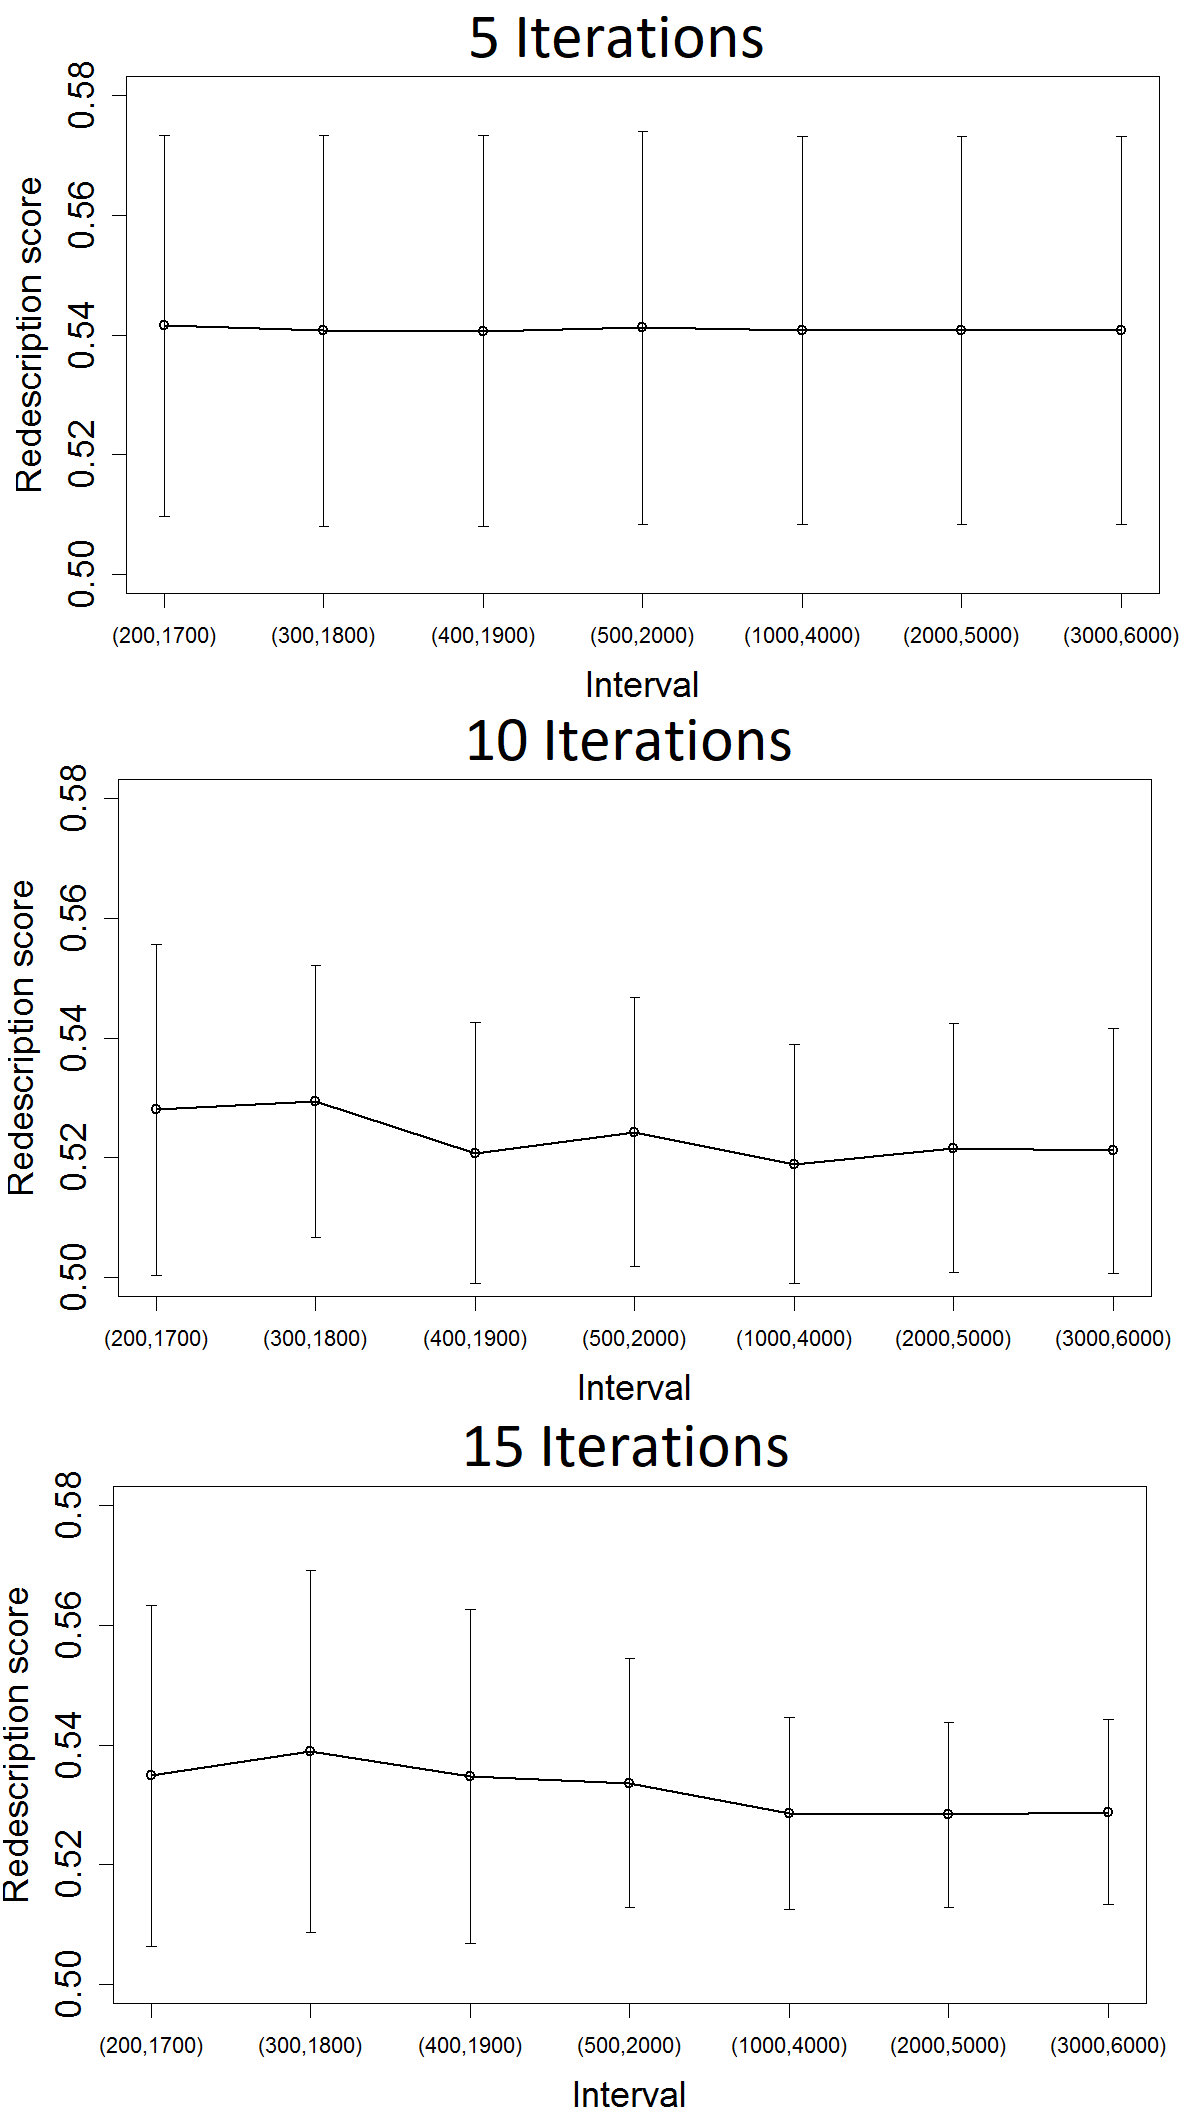}
% \end{center}  
%\caption{Overall score \underline{$\mathcal{R}_{score}$} using different number of iterations inside the GCLUS-RM algorithm and different memory intervals on the Water dataset.}
%\label{fig:MItWater}
%\end{figure}
%
%\begin{figure}[H]
%\begin{center}
% \includegraphics[width=0.75\linewidth]{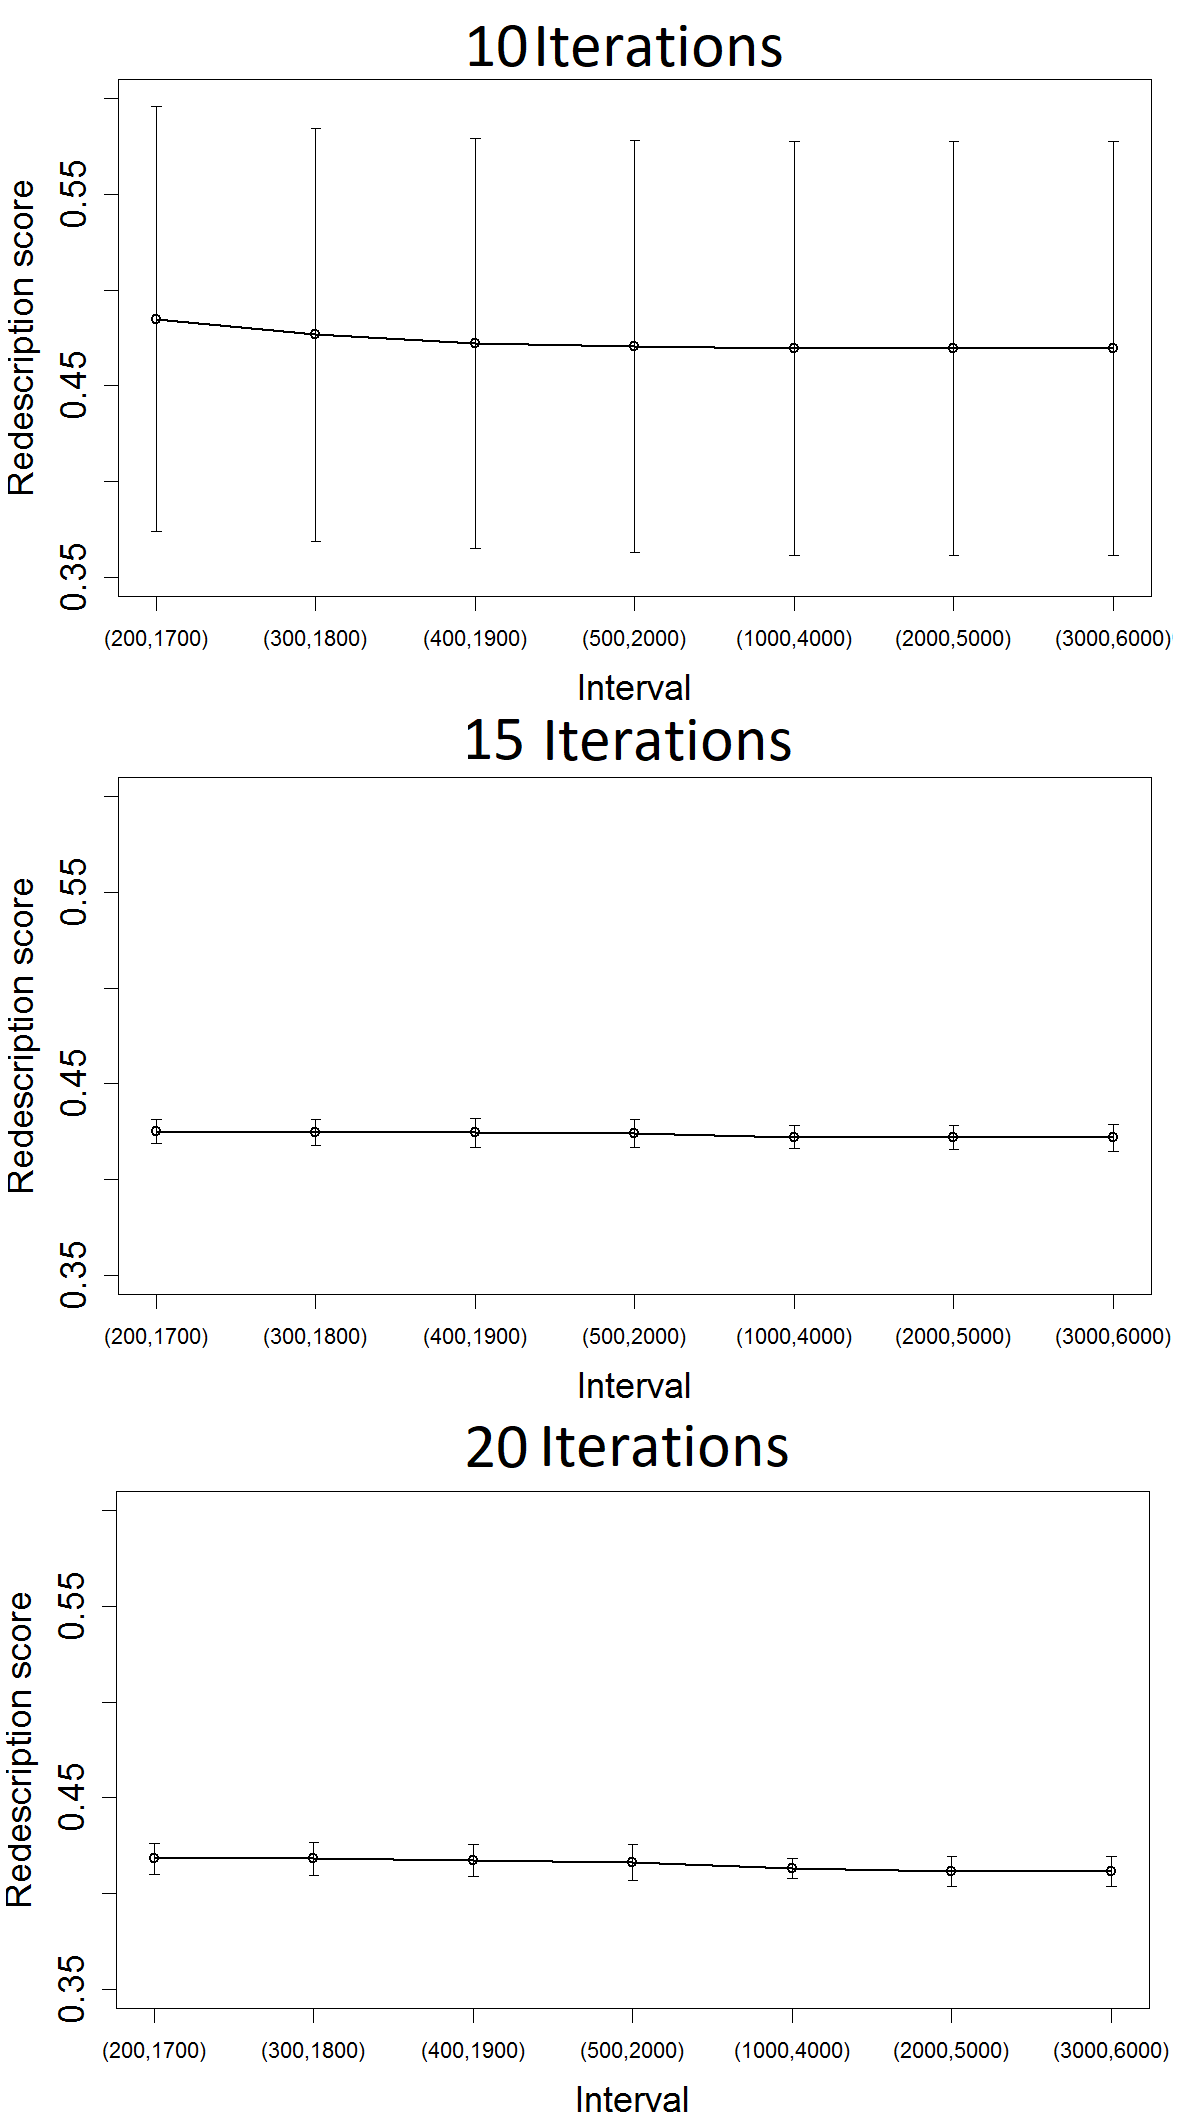}
% \end{center}  
%\caption{Overall score \underline{$\mathcal{R}_{score}$} using different number of iterations inside the GCLUS-RM algorithm and different memory intervals on the Phenotype dataset.}
%\label{fig:MItPhenotype}
%\end{figure}

\section{Execution time of the framework for multi-view redescription mining}

This section contains the empirical execution times of the framework for multi-view redescription mining that uses $1$ generating PCT model. We used the same algorithm parameters as presented in the main manuscript (see Table $2.$ QP/VRSP) with the exception of using $5$ iterations of the GCLUS-RM algorithm on all datasets and using only  $(1000,\ 4000)$ memory configuration. We create redescriptions using $2$ views ($W_1$ and $W_2$), $3$ views ($W_1$, $W_2$, $W_3$) and on Country dataset $4$ views ($W_1$, $W_2$, $W_3$ and $W_4$).

Execution times provided in Figure \ref{fig:ExTime} show a considerable increase in execution time when increasing the number of views used to create redescriptions. On the Country dataset, the framework executes in around $10^{-1} = 0.1$ minutes or $6$ seconds when $2$ views are used, around $10^{0} = 1$ minute or $60$ seconds when $3$ views are used and around $10^{1} = 10$ minutes or $600$ seconds when $4$ views are used. Similarly, the framework executes for slightly less than $10^{-0.5} = 0.32$ minutes or $19$ seconds when $2$ views are used, around $10^{1} = 10$ minutes or $600$ seconds when $3$ views are used on the Slovenian Water dataset. Execution times are smaller on the Phenotype dataset, cca. $10^{-0.8} = 0.16$ minutes or  $9.5$ seconds when $2$ views are used and cca. $10^{0.2} = 1.58$ minutes or $95$ seconds when $3$ views are used to create redescriptions. Such increase in execution time is expected since using two-views necessitates performing $2$ initialization applications of a PCT followed by $2\cdot numIter$ applications of a PCT in the GCLUS-RM iterations. 

\begin{figure}[H]
\centerline{\includegraphics[width=0.8\textwidth]{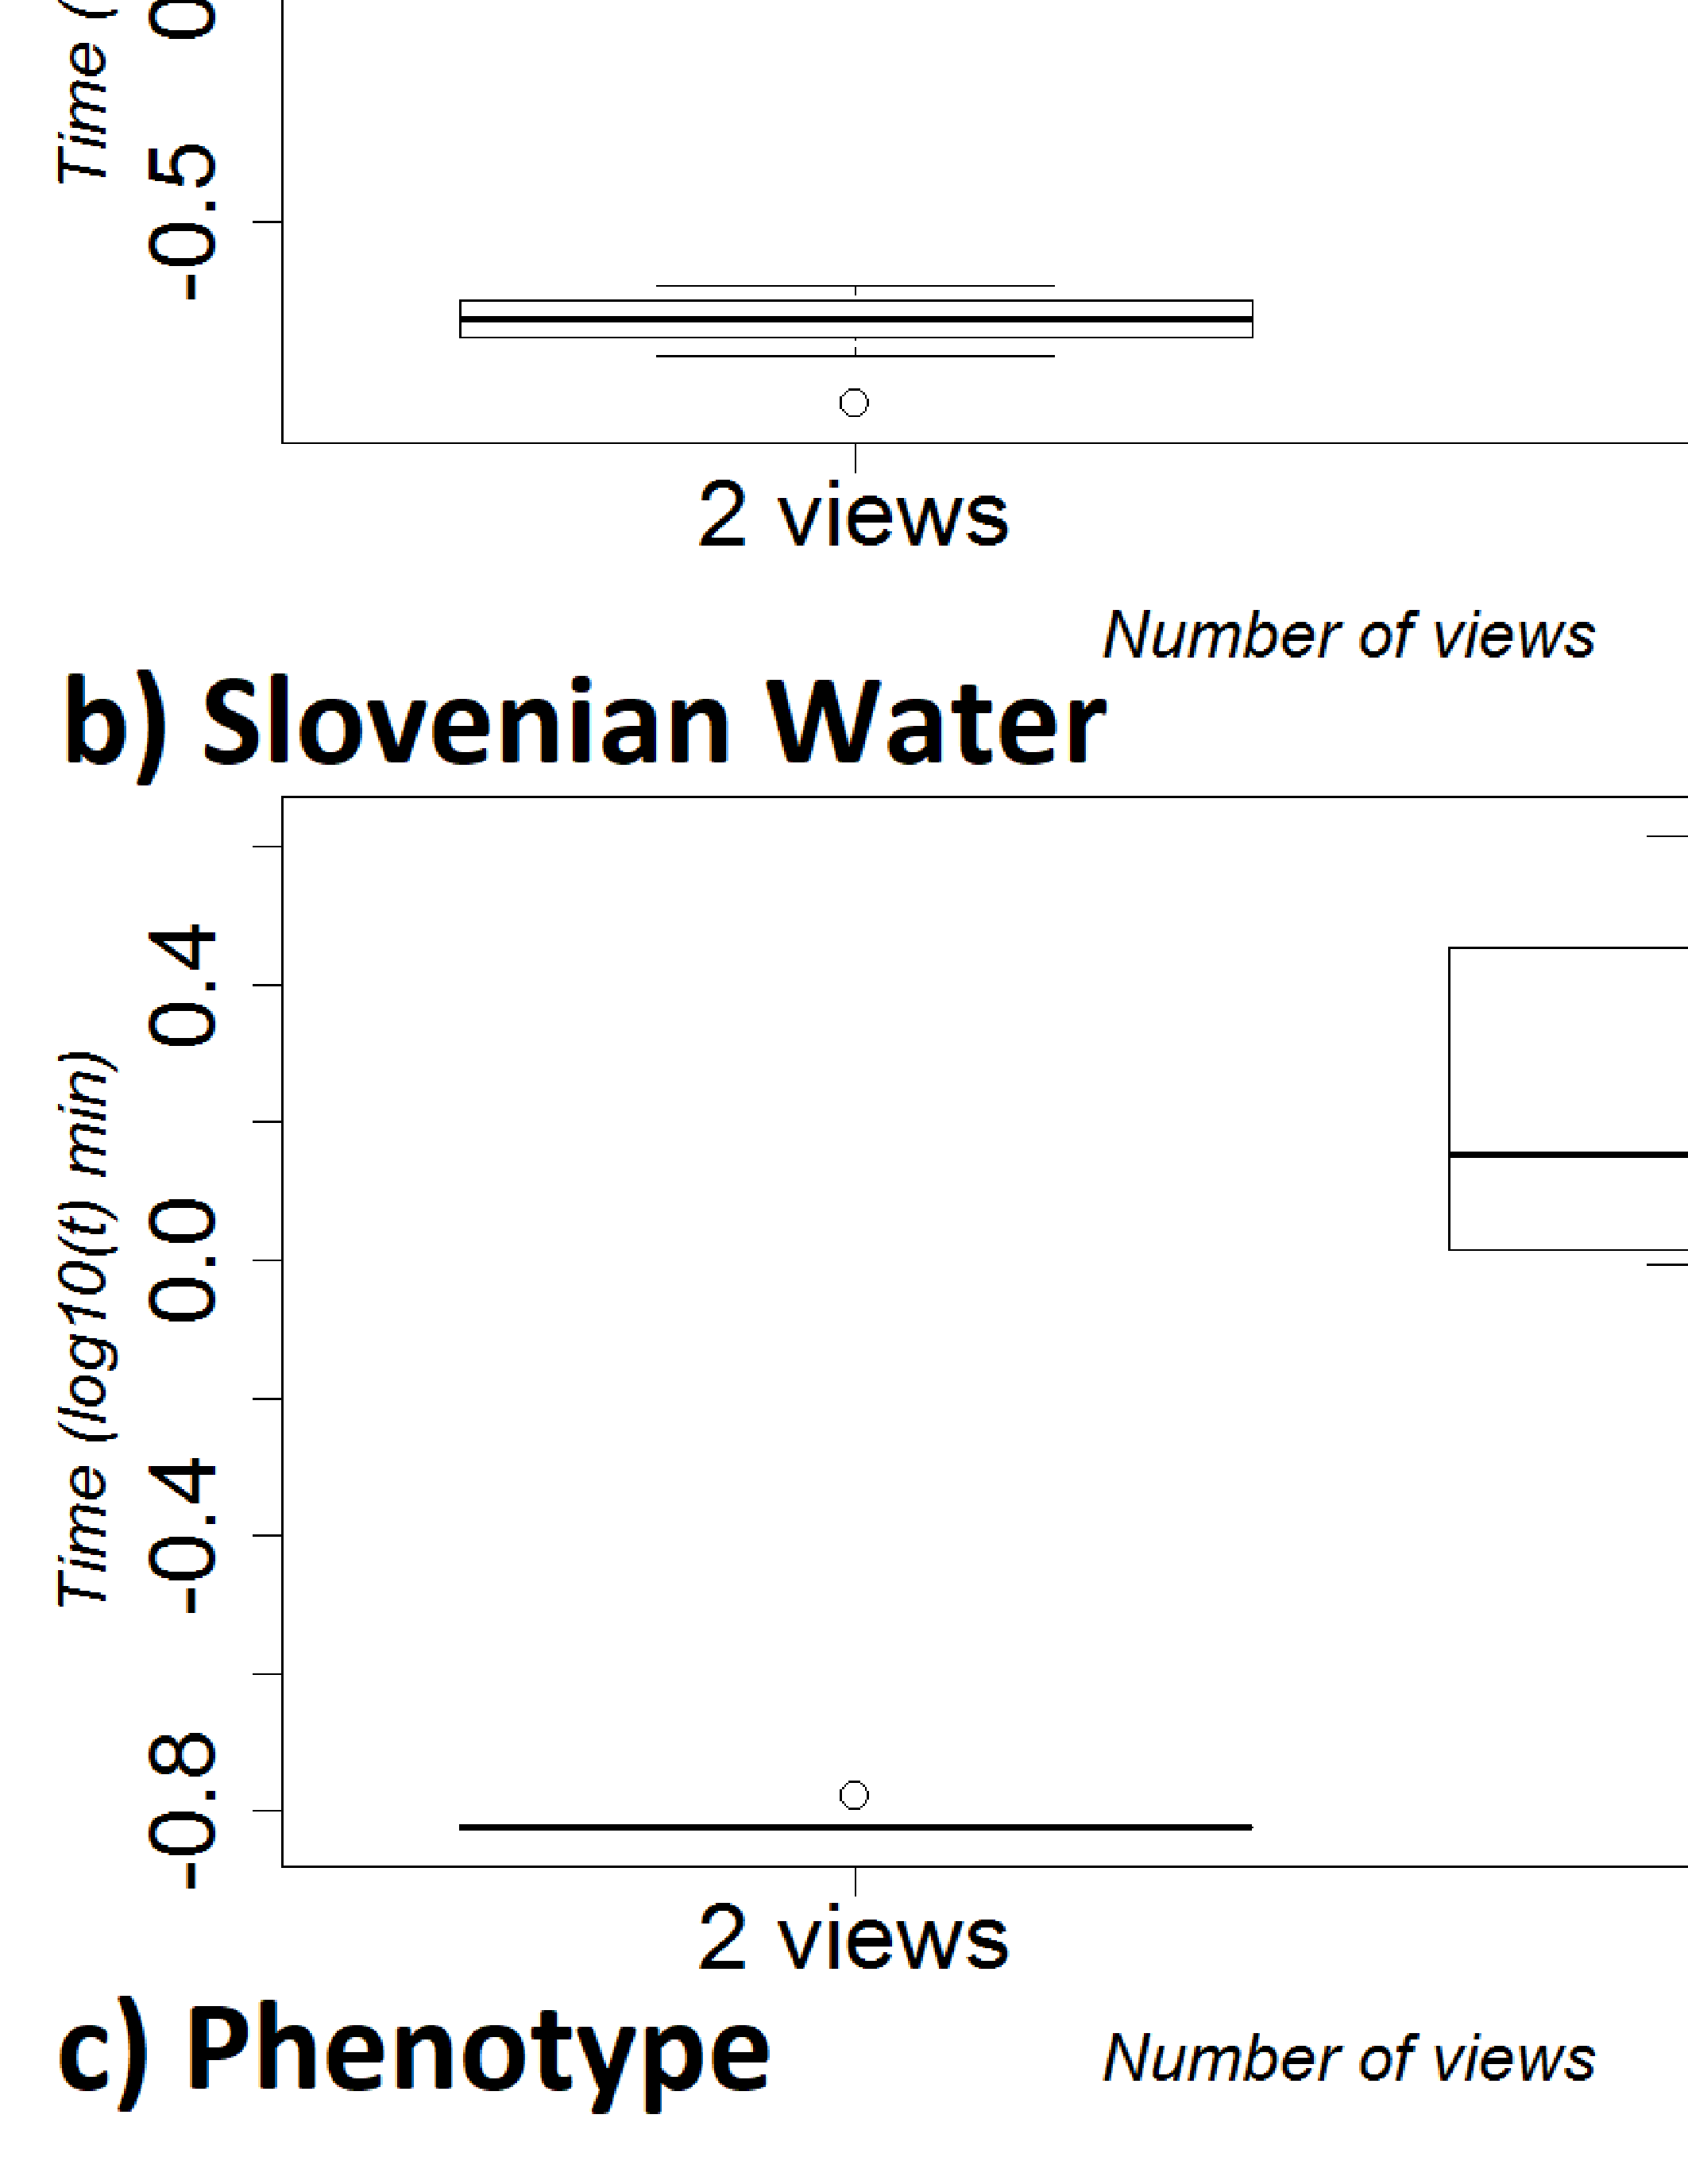}}\caption{$log_{10}$ transformed execution time (in minutes) of a framework for multi-view redescription mining.}
\label{fig:ExTime}
\end{figure}

\noindent Having $3$ views increases the required number of initial applications to $3$ and the following $2\cdot numIter$ applications are repeated $3$ times. After computing redescriptions on two initial views, redescription completion procedure needs to call PCTs on one view $\lceil\frac{|\mathcal{R}|}{nt}\rceil$ times, where $nt$ is the size of a target variable batch ($nt=100$ in all performed experiments). The number of applications further increases when $4$ views are used, since it requires performing $6$ initial applications and the following $2\cdot numIter$ applications are repeated $6$ times. After obtaining pairwise views, redescription completion procedure needs to call PCTs on two views $\lceil\frac{|\mathcal{R}|}{nt}\rceil$ times.
%mention other things, increased number of patterns, more memory management
In addition to the increased number of calls to the PCT algorithm, using larger number of views mostly implies larger number of incomplete redescriptions which burdens memory management and increases the usage of various refinement techniques.

Execution times from Figure \ref{fig:ExTime} have been computed on a PC running $64$-bit Windows $8.1$Pro on Intel Core I7 $4770$ CPU with $3.4$GHz clock speed and $16$GB of RAM ($15.8$GB usable). 

\section{Execution time and memory consumption comparison between the framework and the naive implementation}

In this section we describe the server configuration used to perform the experiments.

Execution time and memory consumption comparison between the proposed framework for multi-view redescription mining and the naive implementation were performed on a server running Debian GNU Linux $10$, having Intel Xeon $E5-2620$ CPU with $2,1$ GHz and $128$ GB of RAM memory. 

The naive multi-view algorithm using ReReMi algorithm has been partially executed in Python and partially in Java. The authors acknowledge that this has partially negative impact on the execution time of this method. For transparency we write the execution times separately for Python and separately for Java for each dataset for the aforementioned method. 

\begin{itemize}
    \item Country dataset: Python - $25958$s , Java - $85393$s 
    \item Slovenian Water dataset: Python - $353$s , Java - $0$s
    \item Phenotype dataset: Python - $20298$s , Java - $8$s
\end{itemize}

\section{ReReMi parameters used to perform the experiments}

In this section we specify the values of parameters used in the experiments that are specific to the ReReMi algorithm.

In all performed experiments we used the \emph{max\_overlap\_area} $= 0.99$ and \emph{max\_red} $= 1000$. \emph{batch\_out} $ = 10$, \emph{batch\_cap} $= 100$ were used on the $\mathcal{C}_{i,j}$ and $P_{i,j},\ (i,j)\neq (2,3)$.On $\mathcal{P}_{2,3}$ we use \emph{batch\_out} $ = 1$, \emph{batch\_cap} $= 10$. Multiple combinations were tried on the Slovenian Water dataset.

\begin{center}
\begin{footnotesize}
\LTcapwidth=\textwidth
\begin{longtable}[c]{|c|c|c|c|c|c|c|c|c|c|c|} % <-- Replaces \begin{table}, alignment must be 
 \caption{Parameters used to obtain redescription sets using the ReReMi $2$-view redescription mining algorithm.}
  \label{tab:ReReMiParams}\\
 \hline
 $\mathcal{D}$ & $MaxSeg$ & $MaxAgg$ & $MaxSideBuck$ & $MaxProdBuck$ \\  \hline 
 
  \endhead % <--  
$\mathcal{C}_{i,j},\ i<j,\ (i,j)\neq (1,2) $ & $40$ & $30$ & $40$ &$100$  \\
$\mathcal{C}_{1,2}$ & $20$ &$15$ & $20$ &$50$ \\
$\mathcal{W}$\footnote{Multiple configurations tried unsuccessfully.} & $100$ &$100$ & $400$ &$1000$  \\
$\mathcal{P}_{i,j},\ i<j,\ (i,j)\neq (2,3)$ & $40$ &$30$ & $40$ &$100$  \\
$\mathcal{P}_{2,3}$ & $10$ &$10$ & $10$ &$10$ \\
\hline
\end{longtable}
\end{footnotesize}
\end{center}

\section{Entity and attribute coverage of redescription sets}
In this section, we present entity and attribute coverage of redescription sets evaluated in Section \ref{sec:quality} with corresponding quality measures presented in Table \ref{tab:res1}.

The entity coverage is the fraction of all entities contained in the dataset that are described by at least one redescription from the redescription set. Similarly, the attribute coverage is the fraction of all attributes used in redescription queries of at least one redescription from the redescription set. 

As in all previous experiments, we provide the average values and the corresponding standard deviations for the proposed framework for multi-view redescription mining and the naive extension using two-view CLUS-RM algorithm, whereas we provide the obtained (single) value for the naive approach using the two-view ReReMi algorithm.

\begin{center}
\begin{footnotesize}
\LTcapwidth=\textwidth
\begin{longtable}[c]{|c|c|c|c|c|c|c|c|c|c|c|c|c|c|} % <-- Replaces
%\begin{table}[H]
%\footnotesize
\caption{Comparative results, with respect to entity/attribute coverage, of a framework for multi-view redescription mining and naive implementations of multi-view redescription mining (NCLUS-RM, NReReMi) on three different datasets (C,W,P). Framework uses a single PCT model as a rule-generating model with different sizes of the working and maximal available memory. The $M$ column contains the name of the naive method or the memory configuration for the proposed framework.}%row -> measures, row+1->deviation
\label{tab:res1}\\
%\centering
%\begin{tabular}{ |c|c|c|c|c|c|c|c|c|c|c|c|c|c| }
\hline
$\mathcal{D}$ & $M$ & $EntCov$ & $EntCovStd$ & $AttCov$ &$AttCovStd$& $Av|\mathcal{R}|$ & $|\mathcal{R}|Std$ \\
\hline

\endfirsthead

\multicolumn{6}{c}%
        {{\textbf{ Table \thetable\ } Continued from previous page}} \\
        \hline

$\mathcal{D}$ & $M$ & $EntCov$ & $EntCovStd$ & $AttCov$ &$AttCovStd$ \\
\hline

\endhead % <-- 
& NLUS-RM & $0.97$ & $0.07$ & $0.27$ & $\mathbf{0.05}$ & $413.4$ & $274.54$ \\
& NReReMi & $\mathbf{1.0}$ & - & $0.27$ & - & $438$ & -  \\
& $200$, $1700$ & $0.99$ & $0.03$ & $0.37$ & $0.09$ & $188.2$ & $37.31$  \\
& $300$, $1800$ & $0.99$ & $\mathbf{0.03}$ & $0.37$ & $0.09$ & $191$ & $28.46$ \\
C & $400$, $1900$ & $0.99$ & $\mathbf{0.03}$ & $0.38$ & $0.09$ & $186.6$ & $42.37$ \\
 & $500$, $2000$ & $0.99$ & $\mathbf{0.03}$ & $0.39$ & $0.08$ & $186.6$ & $42.37$ \\
& $1000$, $4000$ & $0.99$ & $0.03$ & $0.39$ & $0.09$ & $186.6$ & $42.37$ \\
& $2000$, $5000$ &  $0.99$ & $0.03$ & $0.39$ & $0.09$ & $186.6$ & $42.37$ \\
& $3000$, $6000$ & $0.99$ & $0.03$ & $\mathbf{0.39}$& $0.10$ & $186.6$ & $42.37$  \\ \hline
& NCLUS-RM & $\mathbf{1.0}$ & $\mathbf{0.01}$ & $\mathbf{0.96}$ & $\mathbf{0.04}$  & $106$ & $34.42$ \\
& NReReMi & $0.0$ & - & $0.0$ & - & $0$ & -  \\
& $200$, $1700$ & $1.0$ & $0.01$ & $0.94$ & $0.06$ & $200$ & $0.0$ \\
& $300$, $1800$ & $1.0$ & $0.01$ & $0.94$ & $0.06$ & $200$ & $0.0$ \\
W & $400$, $1900$ & $1.0$ & $0.01$ & $0.94$ & $0.06$ & $200$ & $0.0$ \\
& $500$, $2000$ & $1.0$ & $0.01$ & $0.93$ & $0.06$ & $200$ & $0.0$\\
& $1000$, $4000$ & $1.0$ & $0.01$ & $0.93$ & $0.06$ & $200$ & $0.0$ \\ 
& $2000$, $5000$ & $1.0$ & $0.01$ & $0.93$ & $0.06$ & $200$ & $0.0$ \\
& $3000$, $6000$ & $1.0$ & $0.01$ & $0.93$ & $0.06$ & $200$ & $0.0$ \\ \hline
& NCLUS-RM & $0.98$ & $0.03$ & $\mathbf{0.19}$ & $\mathbf{0.01}$ & $3948.8$ & $1570$ \\
& NReReMi & $0.99$ & - & $0.06$ & -& $476$ & - \\
& $200$, $1700$ & $\mathbf{1.0}$ & $\mathbf{0.0}$ & $0.12$ & $0.02$ & $200$ & $0$ \\
& $300$, $1800$ & $\mathbf{1.0}$ & $\mathbf{0.0}$ & $0.13$ & $0.02$& $200$ & $0$ \\
P & $400$, $1900$ & $\mathbf{1.0}$ & $\mathbf{0.0}$ & $0.13$ & $0.02$& $200$ & $0$ \\
 & $500$, $2000$ & $\mathbf{1.0}$ & $\mathbf{0.0}$ & $0.12$ & $0.02$ & $200$ & $0$ \\
& $1000$, $4000$ & $\mathbf{1.0}$& $\mathbf{0.0}$ & $0.14$ & $0.02$ & $200$ & $0$ \\
& $2000$, $5000$ & $\mathbf{1.0}$ & $\mathbf{0.0}$ & $0.14$ & $0.03$ & $200$ & $0$ \\
& $3000$, $6000$ & $\mathbf{1.0}$ & $\mathbf{0.0}$ & $0.14$ & $0.03$ & $200$ & $0$ \\ \hline
%\end{tabular}
%\end{table} 
\end{longtable}
\end{footnotesize}
\end{center}

\bibliographystyle{spbasic}   
\bibliography{vis} 

\end{document}
