# Supplementary material for: Approaches For Multi-View Redescription Mining
Source: arXiv:2006.12227 source file (2020-11-17)
Supplement: Supplementary file 2 [file EM2.pdf]

# Supplementary material to - Targeted and contextual redescription set exploration

Matej Mihelčić, Tomislav Šmuc
Ruđer Bošković Institute
Bijenička cesta 54, 10000 Zagreb, Croatia
{matej.mihelcic, tomislav.smuc}@irb.hr

June 7, 2018

This document contains supplementary information for the manuscript *Targeted and contextual redescription set exploration* submitted to the Journal of Machine Learning.

## 1 Visualizations available in the Siren tool

The Siren tool allows several visualizations focused on the analyses of individual redescriptions. The parallel coordinates plot, allows visualizing values of entities from redescription support, entities not contained in the support but described by some redescription query and entities not described by either redescription query. The decision tree visualization depicts associations between different queries contained in the redescription (especially useful for analyses of redescriptions created by tree-based approaches). The entity scatter plot allows correlation analysis by comparing values of described entities based on two different attributes. If geographical locations are described by redescriptions, the tool is able to represent the locations described by redescription queries on a map. Siren contains several entity visualization techniques based on projections and embeddings. The isomap and locally linear embedding are a non-linear dimensionality reduction techniques. These techniques use different information about neighbourhood of points

to embed them in lower dimensional space. Isomap utilizes multi dimensional scaling whereas locally linear embedding computes eigenvalues and corresponding eigenvectors of the original data matrix to find the embedding vectors. Multi dimensional scaling performs non-linear embedding but tries to preserve distances between points observed in higher dimensional space in a projected (lower-dimensional) space. Randomized PCA projection uses randomized version of singular value decomposition to obtain eignevectors (top $k$ eigenvectors are used to represents entities in a lower dimensional space). Sparse random projection utilizes a sparse random matrix to reduce dimensionality. Spectral embedding uses affinity matrix to create a graph Laplacian which is decomposed using singular value decomposition and the resulting (predefined) number of eigenvectors is used to perform dimensionality reduction. Totally random trees method constructs a forest of random trees and encodes each entity based on its occurrence in different leafs of these trees. This procedure produces a sparse dataset that can be embedded in lower dimensional space using some dimensionality reduction technique (e.g. singular value decomposition).

# 2 Experimental setup

We used the following parameters in CLUS-RM to produce redescriptions used in the presented use cases. $\forall R \in \mathcal{R}_{Country},\ J(R) \geq 0.5,\ p(R) \leq 0.01,\ supp(R) \geq 10,\ |R_{Country}| = 5448,\ max|q_1| = max\ |q_2| = 8,\ \forall R \in \mathcal{R}_{DBLP},\ J(R) \geq 0.2,\ p(R) \leq 0.01,\ supp(R) \geq 10,\ |R_{DBLP}| = 3674,\ max\ |q_1| = max\ |q_2| = 8$ and $\forall R \in \mathcal{R}_{Phenotype},\ J(R) \geq 0.6,\ p(R) \leq 0.01,\ supp(R) \in [10, 650],\ |R_{Phenotype}| = 6200,\ max\ |q_1| = max\ |q_2| = 6$. We performed 800 iterations of the CLUS-RM algorithm on the Country dataset and 120 iterations on the DBLP dataset. On the Phenotype dataset, we used two different initial clusterings (runs) with 40 iterations of the CLUS-RM algorithm each, augmented with random forest containing 100 trees [7]. On this dataset, we restrict query language to the use of only conjunction and literal level negation logical operators (to get descriptions of properties shared between all bacterial species from redescription support set).

# 3 Redescription set exploration using InterSet

In this section, we provide a detailed description of functionality of the InterSet tool.

## 3.1 Entity-based exploration

The entity-based exploration aspect allows exploring redescription set based on support sets of redescriptions. Entities are arranged in SOM clusters using information about their occurrence in redescription support sets. Cluster marked with a red square box in Figure 1 ($C_{sel}$) contains 11 European countries: Austria, Belgium, Denmark, Finland, France, Germany, Italy, Spain, Sweden, Switzerland and United Kingdom. The $|r(C_{sel})| = 2737$, since 2737 redescriptions from $\mathcal{R}$ describe at least one country from $C_{sel}$.

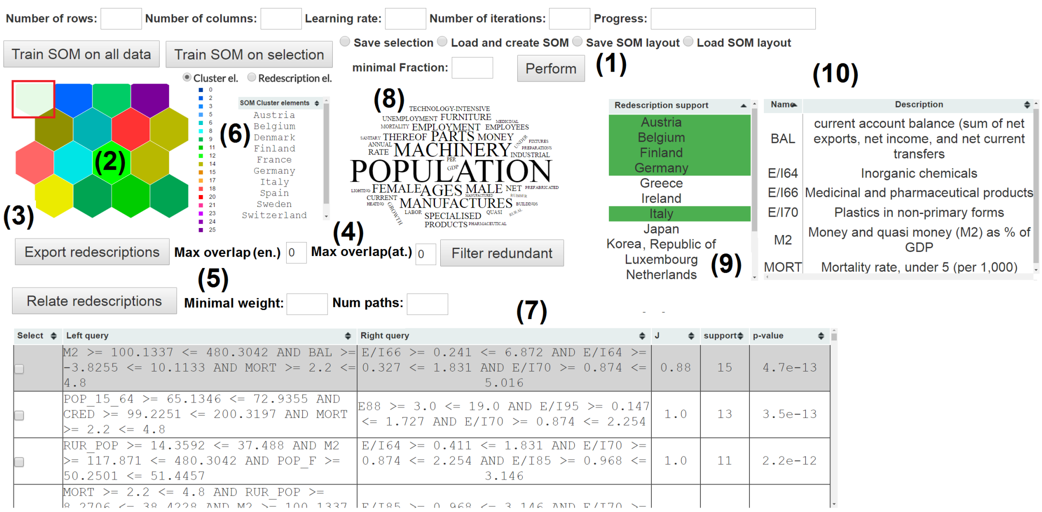


Figure 1: The entity based interface of the InterSet tool.

If the SOM has not been built in the pre-processing stage and displayed with the *load SOM layout* option, it has to be built from within the application. Controls (1) enable specifying required parameters, SOM layout dimensions (with a default setting $4 \times 4$), learning rate (with a default setting 0.1) and number of iterations (with a default setting 100), for the SOM construction. The option *train on all data* allows creating the SOM map on the whole redescription set $\mathcal{R}$. The layout of SOM is customizable and can be easily

experimented with. The color of each hexagon reflects the number of entities contained in each group, displayed on the legend. Cluster $C_{sel}$ is coloured green since it contains 11 entities. The average homogeneity of a cluster can be used as an additional cluster selection criteria. $avHom(C_{sel}) = 0.34$. Selecting an arbitrary SOM cluster $C_i$ from the SOM (Control 2) displays the entities contained in the cluster (Table 6) and additional controls for in depth exploration (Table 7, Control 8). By observing information about all entities contained in the selected hexagon (Table 6) and a Word net (8) displaying words most commonly used in attribute descriptors contained in redescription queries describing at least one entity from the SOM cluster, users can determine if it is of interest to explore all redescriptions associated with the selected cluster (Table 7). The most common words occurring in a Word net when $C_{sel}$ is selected are: *population, machinery, parts, male, female, ages, manufactures, money, rate, products, technology-intense* which may indicate high development of countries contained within it. Entity based exploration aspect also allows creating SOM map on the subsets of redescriptions (Controls 1). Control *train SOM on selection* allows training SOM only on redescriptions from some cluster $C_i$. It can cluster all entities described by at least one selected redescription (option *Redescription el.*), using all redescriptoins from $r(C_i)$ or only entities from a selected cluster (option *Cluster el.*), using redescriptions from $r(C_i)$. By creating the SOM only on redescriptions connected with a particular cluster, users can remove the influence of all other unconnected redescriptions on the SOM construction and obtain potentially more fine grained clusters and subdivisions among selected redescriptions. The Control *load and create SOM* allows creating SOM map on arbitrary subset of redescriptions saved in the database. The last option also allows training SOM map only on redescriptions with higher connectivity to the selected cluster $C_i$. This is obtained by specifying the *minimal fraction* option. For a given parameter $perc$, the tool constructs a set of redescriptions $r(C_i)_{perc}$ defined as:

$$r(C_i)_{perc} = \{R_i \in r(C_i),\ \frac{|supp(R)\ \cap\ C_i|}{|supp(R)|} \geq perc\} \quad (1)$$

For instance, we may be interested in exploring only redescriptions whose support set contains at least 50% of entities from $C_{sel}$. In that case, a redescription with support 5 would need to describe at least 3 countries from $C_{sel}$ and a redescription with support 20 at least 10 to be included into a

redescription set used for SOM construction. Redescriptions can be analysed further on the query and the attribute level (described in Section 6.6 of the manuscript) where Table (9) provides information about the entities described by the selected redescription (members of the SOM cluster are highlighted in green color) and Table (10) provides additional descriptions of compact attribute codes. It is possible to export (Control 3) or filter (Control 4) redescriptions contained in Table (7). The filtering process, described in Algorithm 1, allows reducing the number of redundant redescriptions based on redescription support sets and attributes used in redescription queries. Filtering of redescriptions associated with cluster $C_{sel}$ with parameters *maximal overlap entity* = 30 and *maximal overlap attribute* = 30 results in a set containing 5 redescriptions. Control (5) allows relating redescriptions contained in a selected sequence of redescriptions (described in Section 6.5 of the manuscript).

**Algorithm 1** The filtering algorithm

**Require:** Redescription set $\mathcal{R}$, max entity overlap $\varepsilon_{el}$, max attribute overlap $\varepsilon_{at}$

**Ensure:** Filtered redescription set $\mathcal{R}'$

1: **procedure** FILTER
2: $\quad$ $criteria \leftarrow ((J, desc), (attJ, asc), (supp, desc), (elemJ, asc))$
3: $\quad$ $\mathcal{R} \leftarrow \text{sort}(\mathcal{R},\ criteria)$
4: $\quad$ **for** $i = 0;\ i < |\mathcal{R}| - 1;\ i++$ **do**
5: $\quad\quad$ **for** $j = i + 1;\ j < |\mathcal{R}|;\ j++$ **do**
6: $\quad\quad\quad$ **if** $elemJ(\mathcal{R}[i], \mathcal{R}[j]) \geq \varepsilon_{el}\ \vee\ attJ(\mathcal{R}[i], \mathcal{R}[j]) \geq \varepsilon_{at}$ **then**
7: $\quad\quad\quad\quad$ $\mathcal{R} \leftarrow \mathcal{R}.\text{delete}(\mathcal{R}[j])$
8: $\quad$ **return** $\mathcal{R}$

Criteria array from line 2 in Algorithm 1 contains pairs of redescription quality criteria and sorting direction: desc - descending, asc - ascending. Redescriptions with preferred values of quality criteria are selected and used iteratively to eliminate all redescriptions with unacceptably high entity or attribute Jaccard with the selected redescription. For instance, if $R_{ex}$ is currently selected redescription and *maximal overlap entity* is set to 20 and *maximal overlap attribute* to 10, the algorithm removes all redescriptions such that $J(supp(R_{ex}), supp(R_i)) \geq 0.2$ or $J(attrs(R_{ex}), attrs(R_i)) \geq 0.1$. The pairwise redescription entity and attribute Jaccard index is computed once for all pairs of redescriptions and then saved into the database. Af-

ter that, filtering only requires loading precomputed values which makes it computationally efficient. This filtering is very strict, since it constructs sets containing redescriptions such that there is no pair of redescriptions breaking the defined constraints.

## 3.2 Attribute-based exploration

This section provides additional information about the attribute based redescription set exploration using heatmap (Control 2 in Figure 2). Heatmap is a $k \times k$ matrix where columns represent $k$ attributes from the first view and rows $k$ attributes from the second view. $k$ is defined from Control (1). The heatmap can be created using all redescriptions from $\mathcal{R}$ with *create heatmap on all data* from Control (1), on redescriptions containing a selected pair of attributes with *create heatmap on selection* or on arbitrary redescription selection with *load and create heatmap* option. For a selected pair of attributes $(a_i, b_j)$ and a set of redescriptions $\mathcal{R}$, $\mathcal{R}_{a_i,b_j} \subseteq \mathcal{R}$ denotes a set of redescriptions:

$$\mathcal{R}_{a_i,b_j} = \{R = (q_1, q_2) \in \mathcal{R}|\ a_i \in attrs(q_1)\ \wedge\ b_j \in attrs(q_2)\} \quad (2)$$

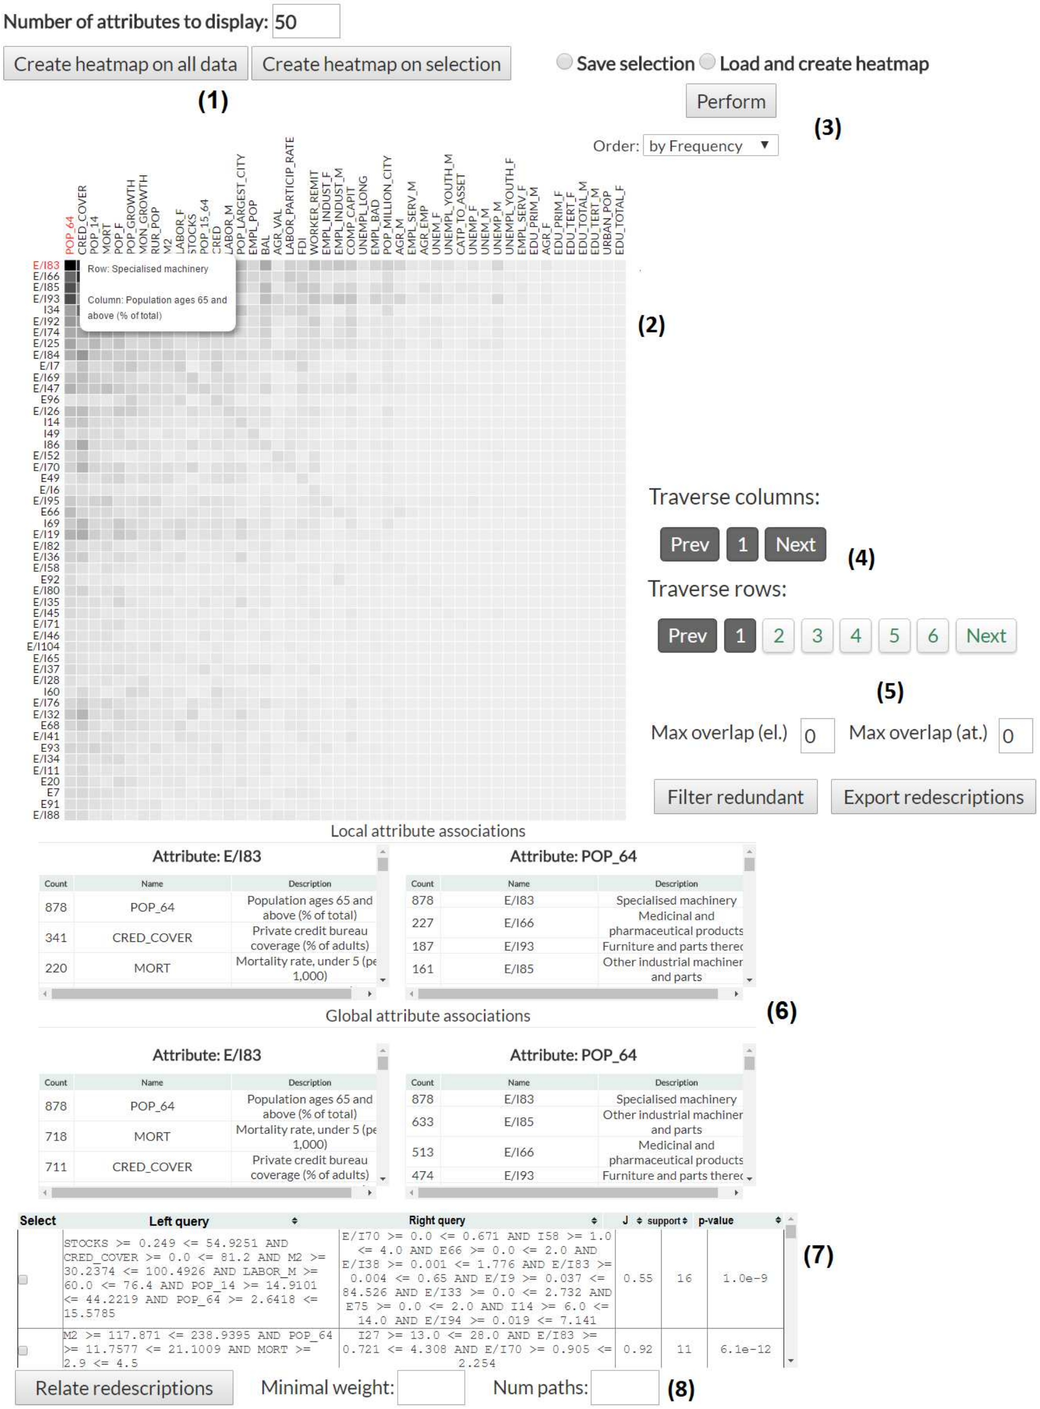


Figure 2: The attribute based interface of the InterSet tool.

Control (3) allows choosing different row-column layouts: 1) *Ordered by name*, 2) *Ordered by frequency* and 3) *Ordered by co-occurrence*. Ordered by name (useful for domain experts) option sorts rows and columns by the attribute code, *Ordered by frequency* places more frequently occurring attributes closer to the top left corner of the heatmap and *Ordered by co-occurrence* layout arranges rows and columns so that it sorts the heatmap diagonal in descending order by attribute co-occurrence frequency. The heatmap is adopted to work with larger number of attributes by loading smaller submatrices (achieved with Control 4) of the potentially large cross-view attribute matrix, whose rows are all attributes from the first view and columns all attributes from the second view. The gray color denotes the co-occurrence level of the attribute pair and Table 7 lists all redescriptions from the redescription set containing the selected attribute pair in their queries. Analysis of the selected redescription is described in Section 6.6 of the manuscript, redescription filtering (Control 5), (Algorithm 1) in Section 3.1, redescription export (Control 5) is described in Section 3.1 of this document and redescription relation (Control 8) in Section 6.5 of the manuscript. Combination of various attribute pair arrangements with redescription exploration and filtering allows better understanding of the attribute interactions. Control (6) allows focused examination of associations of selected attributes (each attribute from a pair) and its top $k$ co-occurring attributes (sorted in decreasing order by co-occurrence): a) globally, b) locally. Global associations are obtained by counting its co-occurrences with other attributes based on all redescriptions contained within set $\mathcal{R}$, whereas local associations are obtained by counting attribute co-occurrences in all redescriptions from the selection (some redescription set $\mathcal{R}_s \subset \mathcal{R}$). In the example presented in Figure 2, the selected subset of redescriptions is $\mathcal{R}_{E/I_{83},POP_{64}}$. We can see that for attribute $E/I_{83}$ the second most frequently co-occurring attribute is $CRED\_COVER$ in the set $\mathcal{R}_{E/I_{83},POP_{64}}$, however the second most frequently co-occurring attribute in $\mathcal{R}$ is $MORT$. Selecting an attribute from a table of globally associated attributes has similar effect as selecting a pair of attributes on a heatmap. It creates a set of redescriptions $\mathcal{R}_{a_i,b_j}$. Selecting an attribute from the local associations table, constrains the currently selected redescription set to only those redescriptions containing the newly selected attribute. For instance, if we start from a set $\mathcal{R}_{a_i,b_j}$, selecting an attribute $b_k$ from the list of local associations creates a new redescription set $\mathcal{R}_{a_i,b_j \wedge b_k}$. All selections of attributes from the local table are saved, allowing users to backtrack and change selections as attribute exploration progresses.

## 3.3 Property-based exploration

The property-based exploration aspect allows filtering based on different redescription and redescription set properties (see Figure 3).

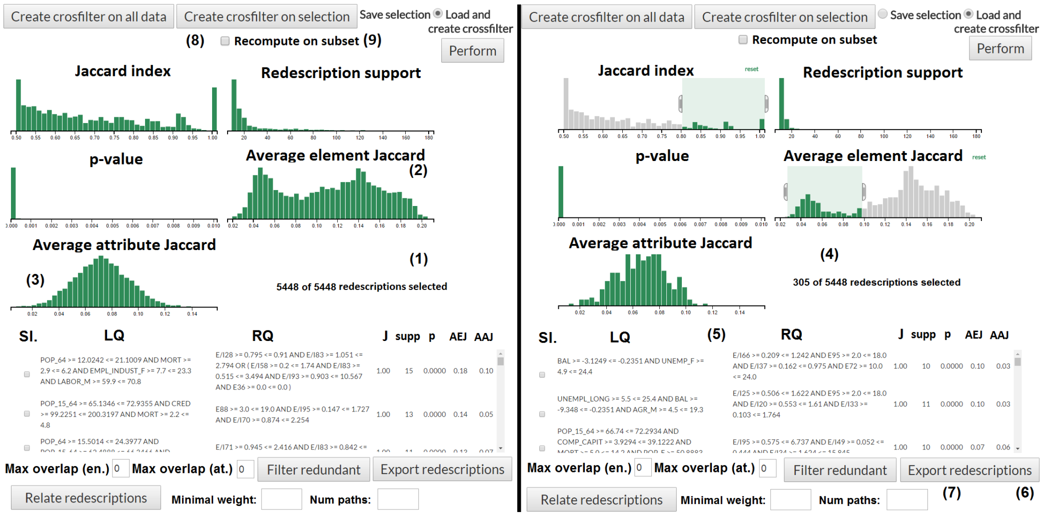


Figure 3: The InterSet interface based on redescription properties. Initial configuration is shown in the left and the filtering step in the right part of the Figure.

This exploration aspect uses sliders and a crossfilter (Control 1 in Figure 3) and displays value distribution of various redescription quality measures (Controls 2 and 3). It instantaneously displays value distribution of different quality criteria for redescriptions contained in the filtered redescription set (Control 4) and allows exploration of redescriptions through a Table 5. Analysis of the selected redescription is described in Section 6.6 of the manuscript, redescription filtering (Control 6), (Algorithm 1) in Section 3.1, redescription export (Control 6) is described in Section 3.1 of this document and redescription relation (Control 7) in Section 6.5 of the manuscript.

It is possible to create a crossfilter using all redescriptions from $\mathcal{R}$ or any selected subset by using Controls 8. Control (9) allows recomputing currently defined measures on a selected subset of redescriptions. Suppose we save a redescription set $\mathcal{R}_s \subset \mathcal{R}$ into a database and load it using *load and create crossfilter* option. The crossfilter will be created and display value distributions of different measures based on the whole redescription set $\mathcal{R}$ (that is

measures $AEJ$ and $AAJ$ will display the redundancy based on all redescriptions contained in $\mathcal{R}$). This is often useful when searching for redescriptions that are very different or very similar to many other redescriptions in the set $\mathcal{R}$. However, sometimes it is also desired to find such knowledge based on the information contained in the selected subset of redescriptions $\mathcal{R}_s$. For instance, we select only those redescriptions containing some pair of attributes and would like to find those redescriptions that describe very different subsets of entities compared to majority of other redescriptions in that set. This is possible by using control (9). We will denoted such filtering as $\mathcal{F}_{R_s}$.

# 4 Using interaction between different aspects in InterSet

Here, we provide one example of using interaction between aspects to enhance the redescription set exploration. Assuming that the exploration step started on the input redescription set $\mathcal{R}$ and that as the initial exploration aspect, the user chooses entity based exploration. Further, let's assume that it is interesting to examine redescriptions describing entities from the cluster $C_k$, obtain by SOM. The selected set of redescriptions can be further reduced to include those containing a minimal percentage of entities from this cluster in the support set which produces the $r(C_k)_{perc}$. This selection must be saved into database to expand the exploration by using other exploration aspects. If $A = r(C_k)_{perc}$ is loaded into the property based exploration aspect, we can filter this set further by selecting (for instance) only highly accurate redescriptions ($\mathcal{F} = \{J \in [0.9, 1.0]\}$), obtaining $A_{\mathcal{F}}$. Again, this set needs to be saved to allow the attribute association analysis. If we denote the loaded set as $B = A_{\mathcal{F}}$, the obtained redescription set, after selecting the attribute pair $(a_i, b_j)$, $B_{a_i,b_j}$ can be explored on the individual redescription level, or some additional associations can be explored. Exploring associations between multiple attribute pairs can be obtained by creating the sequence of redescription sets: $D = B_{a_i,b_j},\ E = D_{a_k,b_j},\ F = E_{a_k,b_c}$ etc. by iteratively saving the selected subsets of redescriptions, creating new attribute heatmap on this selection and making further selections.

# 5 Individual redescription analysis

In this section, we describe the notched box plot visualization to analyse entity value distribution of individual redescriptions. All components of this visualization can be seen in Figure 4. It visualizes the entity distribution for redescription $R_{new_1}$ presented in Table 1.

Table 1: Redescription $R_{new_1}$.

| | |
|---|---|
| $R_{new1}$ : | $(q_{1_{new1}}, q_{2_{new1}})$ |
| $q_{1_{new1}}$ : | $15.5 \leq \texttt{POP}_{64} \leq 21.1 \;\wedge\; -0.4 \leq \texttt{FDI} \leq 5.4 \;\wedge\; 0.1 \leq \texttt{POP. GROWTH} \leq 1.3$ |
| $q_{2_{new1}}$ : | $0.56 \leq \texttt{E/I}_2 \leq 1.5 \;\wedge\; 0.2 \leq \texttt{E/I}_{93} \leq 0.7 \;\wedge\; 0.76 \leq \texttt{E/I}_{85} \leq 1.57 \;\vee$ |
| | $(0.9 \leq \texttt{E/I}_{93} \leq 3.5 \;\wedge\; 0.95 \leq \texttt{E/I}_{71} \leq 1.9)$ |
| $supp(R_{new1})$ : | Austria, Belgium, Denmark, Finland, France, Germany, Italy |
| | Netherlands, Norway, Spain, Sweden, Switzerland, United Kingdom |
| quality: | $J(R_e) = 0.93,\; \lvert supp(R_e)\rvert = 13,\; p(R_e) = 9.3 \cdot 10^{-13}$ |

The visualization presented in Figure 4 contains notched box plots instead of violin plots which enable visualizing the confidence interval of the median and the outliers. The trend plots allow visualizing the difference between quartiles between different groups of interest.

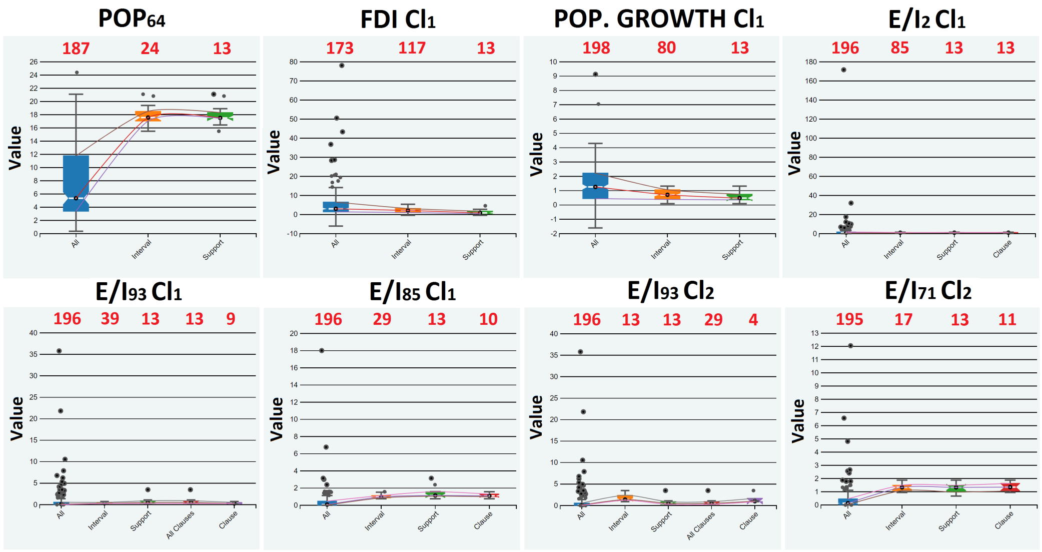


Figure 4: Comparative notched box plots with trend lines for $R_{new1}$.

# 6 Applications

In this section we provide additional explanations connected to usecase examples presented in the manuscript.

## 6.1 DBLP dataset

We present a description of all SOM clusters with homogeneity larger than 0.2 (see Figure 10 of the manuscript and Figure 5).

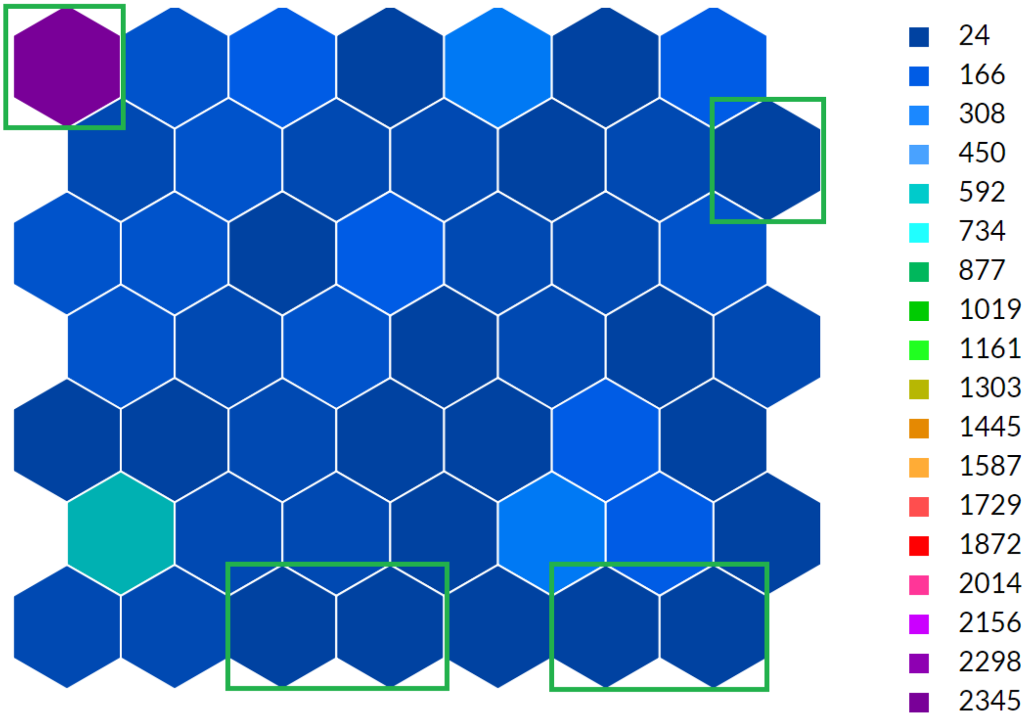


Figure 5: SOM obtained on the DBLP dataset. Clusters with average homogeneity > 0.2 are encircled in green color.

Discovered clusters with homogeneity larger than 0.2 describe authors that publish majority of papers on the following conferences (clusters are enumerated from left to right, top to bottom):

1. Conference on Learning Theory (COLT), International Conference on Machine Learning (ICML).

2. International Conference on Computer Aided Design (ICCAD), International Conference on Computer Aided Verification (CAV), Design Automation Conference (DAC).

3. Symposium on computational geometry, Canadian Conference on Computational Geometry (CCCG), ACM-SIAM Symposium on Discrete Algorithms (SODA), Algorithms and Data Structures Symposium (WADS).

4. Symposium on computational geometry, Canadian Conference on Computational Geometry (CCCG), ACM-SIAM Symposium on Discrete Algorithms (SODA), Symposium on the Theory of Computing (STOC).

5. Symposium on computational geometry, IEEE conference on computational complexity, Annual International Cryptology Conference (CRYPTO), Annual IEEE Symposium on Foundations of Computer Science (FOCS), Symposium on the Theory of Computing (STOC)

6. IEEE conference on computational complexity, Annual International Cryptology Conference (CRYPTO), Annual IEEE Symposium on Foundations of Computer Science (FOCS), Symposium on the Theory of Computing (STOC), International Conference on the Theory and Application of Cryptographic Techniques (EUROCRYPT)

## 6.2 Phenotype dataset

In this section we list all SOM clusters obtained on the Phenotype dataset with average homogeneity larger than $> 0.5$. Clusters are presented from left to right, top to bottom (see Figure 6).

1. This cluster has average homogeneity 0.52 and contains 33 bacterial species. The most common phenotypic traits are: *unicellular*, *photosystem*, *photosynthesis*, *ocean*, *fixat*. From these phenotypes, we see that these bacteria are mostly unicellular capable of performing photosynthesis and that they mostly live in the ocean. The main representatives of this cluster are *Synechococcus*, *Cyanothece* and *Nostoc* genus of cyanobacteria.

2. The second cluster of interest has average homogeneity 0.71 and it contains 17 bacterial species. The most common discovered phenotypic traits are: *haloarchaea*, *hypersalin*, *archaeal*, *seafood*, *NaCl*. The

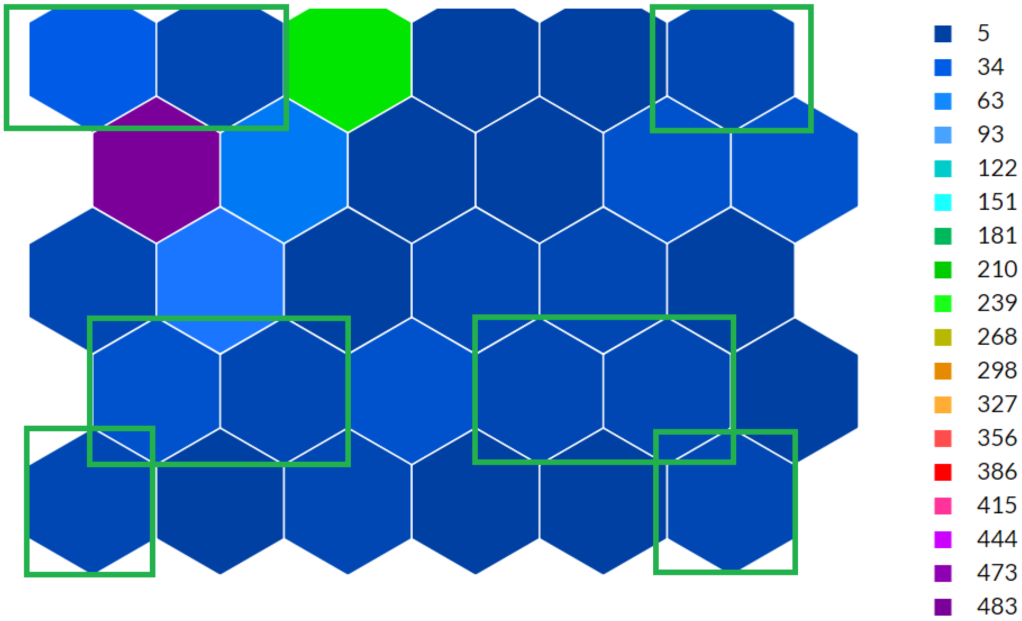


Figure 6: SOM obtained on the Phenotype dataset. Clusters with average homogeneity > 0.5 are encircled in green color.

haloarchea (previously referred to as halobacteria), leave in the extreme environments (which is evident from the phenotype hypersalin) [4]. This also explains the further two phenotypes seafood (since it is often found in salted fish) and NaCl because of the fact that high salinity attracts the haloarchea [8].

3. The third cluster, with average homogeneity 0.63 contains 14 bacterial species. These species are characterized with the following phenotypic traits: *habitat free living*, *shape tailed*, *(aerial, mycelium, spore, hypha, soil)*, *sporulation* and *gram stain positive*. These bacteria are abundant in soil and are able to produce aerial spores to preserve their genetic material[1]. The most known representative is *Streptomyces*. Streptomyces is a gram-positive bacteria, meaning that it has a very thick cell wall made of a protein *peptidoglycan*.

[1] `https://www.sciencedirect.com/topics/immunology-and-microbiology/aerial-hypha`

4. This cluster has average homogeneity 0.68 and contains 20 species characterized with the following phenotypic traits: *oxygen request strict aero*, *infect patient pathogen viral opportunist* and *biotic relationship symbiotic*. The most notable representative are *Rickettsia* [1] - pathogens found in many animal species, ticks, lies, flees, causes various disease in humans, *Anaplasma* [10] - pathogenic bacteria causing disease in farm animals and to a leaser degree in humans and *Wolbachia* which is mostly transmited by and infects antrophod spicies, such as mosquitos [3]. It is a parasitic organism.

5. The fifth cluster of interest has the average homogeneity 0.67 and contains 16 entities. The most important phenotypic traits are: *hydrogen sulfide*, *host marine invertebrates*, *cell arrangement pairs* and *(Fe, acceptor, dissimilatori, metal, donor)*. This cluster contains various species of bacteria from genus *Shewanella*. This bacteria shares many characteristics with bacterial species from the previous cluster, such as the fact that it inhabits other species (marine invertebrates), even causing disease in some species, such as trout. It can use oxygen for respiration, but can also reduce iron [11]. It produces hydrogen sulfide [13] and is a gram-negative bacteria. As opposed to the gram-positive bacteria, gram-negative bacteria have thin, but very strong membrane.

6. This cluster, with average homogeneity 0.53, contains 19 species of a bacterial genus called *Lactobacillus*. The highly occurring discovered phenotypic traits are: *(lactic, cheese, food, ferment, milk)*, *cell arrangement chains*, *gram stain positive*, *oxygen requirement facultative*. Bacteria of this genus are gram positive, found in human intestines and used in production of various fermented products (such as yoghurt and cheese)[2].

7. This cluster, with average homogeneity 0.7, contains 15 different species of genus *Mycobacterium*. The most common phenotypic traits discovered are: *metabolism PAH degrading* and *gram stain positive*. These gram stain positive bacteria are involved in degradation of Polycyclic Aromatic Hydrocarbons (PAHs) [2], which are by itself large pollutants and hazardous for human health. Many species from this group can cause disease in mammals and in humans. Most notably tuberculosis

[2] https://www.sciencedirect.com/topics/immunology-and-microbiology/lactobacillus

caused by *Mycobacterium tuberculosis*, and leprosy caused by *Mycobacterium leprae.*

8. This cluster has the average homogeneity 0.62 and contains 13 different bacterial species. It contains bacterial species from genus *Mesorhizobium*, *Bradyrhizobium*, *Sinorhizobium* and *Rhizobium.* The most common phenotypic characteristics are: *known habitats root nodule* and *(soy bean, legum, max, rhizobia, fast grow).* Many bacterial species from the aformentioned genus fix nitrogen and reside in root nodules of plants. Soy beans are legum that can form a symbiotic relationship with bacteria Rhizobium[3].

9. With the average homogeneity of 0.57, this cluster contains 15 bacterial species. The most common phenotypic properties are: *oxygen request strict anaero*, *(vent, hydrotherm, deep sea, chemo, litho, autotroph, sulfuroxid)*, *temperature range hyperthermophilic*, *(ecosystem, subtype, hydrothermal vents).* From aforementioned phenotypic traits, we may deduce that these bacterial species live in high temperatures, near sources of heat such as hydrothermal vents. Bacterial species contained within this cluster belong to three different bacterial genus: *Pyrococcus*, *Methanocaldococcus* and *Thermococcus.* Members of the Pyroccocus and Thermoccocus genus are all thermophilic, meaning that they thrive in high temperatures. Bacteria in genus Methanocaldococcus are mostly meshopiles (live on temperatures less than 45 degrees), however species contained within a cluster are all thermophilic.

Using redescriptions describing bacterial species contained in the second SOM cluster, we analysed attributes highly associated with phenotypic traits *(haloarchaea, hypersalin, archaeal, sea food, NaCl).* These interesting discoveries were found:

1. There is a number of uncharacterised proteins whose study should be conducted in order to understand their potential connection with the given phenotype (e.g. $COG_{3361}$, $COG_{4044}$, $COG_{4749}$ $COG_{1873}$ etc. ).

2. $COG_{1121}$ (ABC-type Mn/Zn transport systems, ATPase component). This cluster of genes is a part of mechanisms aimed at increasing

[3]https://www.sciencedirect.com/topics/agricultural-and-biological-sciences/rhizobium

haloarchea tolerance to different metals soluble in water of high salinity (which is one of the phenotypic traits of these orgnisms). The overview of such mechanisms, including ATPase and ABC transporters is provided in [5].

3. $COG_{843}$ (Heme/copper-type cytochrom e/quinol oxidases, subunit 1) is involved in reduction of $O_2$ into water. As described in [12], Halobacteria use this mechanism (equally type B and type A1 enzymes).

4. $COG_{578}$ (glycerol-3-phosphate dehydrogenase). It has been shown on the example of *Haloferax volcanii* [9] that glycerol-3-phosphate dehydrogenase has a role in catabolization of glycerol (a primary source of energy for heterotrophic haloarchaea).

# 7 Time complexity analysis of the InterSet tool

In this analysis, we focus on the time complexity of different algorithms and visualizations used within InterSet. The analysis is divided to algorithms and visualizations on the client side and data access on the server.

## 7.1 Analysis of computational cost on the client side

The computational complexity of training a Kohonen map (SOM) of dimensions $n \times n,\ n \in \mathbb{N}$ on a data set containing $|E|$ entities equals $O(n^2)$, with the currently used algorithm. This can be reduced by using some of the more optimised versions with worst time complexity $O(n \cdot log(n))$, $O(n)$, $O(log(n))$ and $O(log_2(n))$ (for more details see [6]). This analysis holds if the number of features used in SOM construction is very small and represents a constant in the algorithm complexity. In our case, however, this is not true. In fact, the number of features equals $|\mathcal{R}|$ and is a dominating factor in the algorithm. Because of this, given that $n^2 << |\mathcal{R}|$ as in our case, the learning of SOM will have a worst time complexity of $O(|\mathcal{R}|)$ or $O(|\mathcal{R}| \cdot |E|)$ if all entities from a dataset are used in training. Visualizing SOM map has complexity $O(|\mathcal{R}|)$. Selecting any SOM cluster requires displaying all redescriptions contained in the redescription set. It also requires displaying a table of entities contained in the cluster and creating a WordNet visualization. WordNet creation has worst time complexity $O(|\mathcal{R}_{C_i}| \cdot |s|)$ (the creation of WordNet also requires parsing strings corresponding to the attribute descriptions contained within

their queries. We assume the maximal size $|s|$ of these descriptions). Creation of a table containing all redescriptions associated with a selected SOM cluster has time complexity $O(|\mathcal{R}_{C_i}|)$ whereas creating a table containing all entities contained within a cluster has a time complexity $O(|C_i|)$. The overall time complexity of this step is $O(|\mathcal{R}_{C_i}| \cdot |s| + |C_i|)|$.

Since heatmap visualizes only a part of attribute space ($dim \times dim$ for some $dim \in \mathbb{N}$), its time complexity on the client side, when created for all redescriptions is $O(1)$. If all attribute pairs are displayed at once (which is very incomprehensible and opposite to the paginating nature of the exploration aspect), then the complexity is $O(|V_1| \times |V_2|)$. When created on the selected subset of redescriptions, we must re-compute the attribute co-occurrences for the selected subset of redescriptions which has complexity $O(|\mathcal{R}_{sel}|)$. Selecting any pair of attributes requires creating a table containing all redescriptions contained in the subset, thus it has time complexity $O(|R_{a,b}|)$.

Crossfilter has the worst time complexity $O(|\mathcal{R}| \cdot log(|\mathcal{R}|))$, since it sorts redescriptions using heap sort after selection. However, this occurs only if no prior selection of redescriptions is made (when first constraint in crosfilter is defined), otherwise only redescriptions from the current selection are sorted.

The complexity of redescription filtering procedure available in InterSet is $O(|\mathcal{R}|^2)$, however this occurs only in case of very mild filtering constraints (that eliminate very small amount of redescriptions). In practice, stricter constraints result in faster algorithm execution. In such cases, the algorithm complexity is $O(|\mathcal{R}| \cdot log(|\mathcal{R}|))$.

The redescription relation graph has the worst time computational complexity $O(|\mathcal{R}|^3)$, however, due to the threshold imposed on the minimal weight of the edge during the search for shortest paths, the algorithm executes considerably faster since it does not need to traverse the whole graph.

Individual redescription analysis has a time complexity $O(|E|^2)$ due to kernel density estimation procedure used to visualize volin plots. In this step, different representative sub samples can be used to visualize approximation of data distribution for datasets containing very large number of entities.

All upper bounds on asymptotic execution were given under the assumption that visualizations or the incorporated algorithms are run on the whole redescription set $\mathcal{R}$. Using any of the selected methods on the whole redescription set occurs very rarely, since the whole point of exploration is to allow using different interesting subsets.

## 7.2 Analysis of computational cost on the server side

Depending on the task, operations on a database have worst time complexity $O(|E|)$ (when saving entity coverage into database), $O(|\mathcal{R}|)$ (when saving, loading redescription set into or from database), $O(|\mathcal{R}| \cdot |E|)$ (in case all redescriptions describe very large subsets of entities, this is however very rarely the case), $O(|\mathcal{R}| \cdot log(|\mathcal{R}|))$ (for loading redescriptions connected with a SOM cluster), $O(log(|E|))$ (to get entities associated with a SOM cluster). The most complex queries have worst time complexity $O(log((|V_1|+|V_2|)^2) \cdot log(|V_1|+|V_2|)^2) = O(log(|V_1|+|V_2|)^3)$ (to obtain all attribute co-occurrences and related information) and $O(|\mathcal{R}|^2)$ to get necessary entity and attribute Jaccard indexes for all pairs of redescriptions when performing filtering or creating a redescription relation graph.

Data about entity and attribute Jaccard index are loaded once and used from memory throughout user session.

# 8 Detecting associations with InterSet

As an example of detecting associations, we show how our approach can detect correlated attributes. Let's assume that $At$ and $Bt$ are two perfectly (positively) correlated attributes on a set of entities contained in the dataset. This means that for each pair of entities $e_i,\ e_j \in E$, if $At(e_i) \geq At(e_j)$ then $Bt(e_i) \geq Bt(e_j)$. Thus, if $At_a^b$ occurs in one redescription query, the perfect match $Bt_c^d$ can be obtained by finding entity $e_1$ such that $At(e_1) \simeq a$ and $e_2$ such that $At(e_2) \simeq b$ and computing $c = Bt(e_1)$ and $d = Bt(e_2)$. Assuming correct function of redescription mining algorithms, $Bt$ should occur frequently in the second redescription query given that $At$ occurs in the first query because it increases redescription accuracy (the subset of entities described by the first query can be perfectly described with the second query). Analogous case is valid for negatively correlated attributes. Thus, highly co-occurring attributes in redescription queries could indicate but do not guarantee attribute correlations.

# References

[1] Samuel Baron. *Epidemiology–Rickettsiae.* University of Texas Medical Branch at Galveston, 1996.

[2] Debajyoti Ghosal, Shreya Ghosh, Tapan K Dutta, and Youngho Ahn. Current state of knowledge in microbial degradation of polycyclic aromatic hydrocarbons (pahs): a review. *Frontiers in microbiology*, 7, 2016.

[3] Francis M. Jiggins. The spread of wolbachia through mosquito populations. *PLOS Biology*, 15(6):1–6, 06 2017.

[4] Sean P Kennedy, Wailap Victor Ng, Steven L Salzberg, Leroy Hood, and Shiladitya DasSarma. Understanding the adaptation of halobacterium species nrc-1 to its extreme environment through computational analysis of its genome sequence. *Genome research*, 11(10):1641–1650, 2001.

[5] Meenal Kowshik. Mechanisms of metal resistance and homeostasis in haloarchaea. *Archaea*, 2013, 2013.

[6] H. Kusumoto and Y. Takefuji. $o(log_2 m)$ self-organizing map algorithm without learning of neighborhood vectors. *IEEE Transactions on Neural Networks*, 17(6):1656–1661, Nov 2006.

[7] Matej Mihelcic, Saso Dzeroski, Nada Lavrac, and Tomislav Smuc. Redescription mining augmented with random forest of multi-target predictive clustering trees. *Journal of Intelligent Information Systems*, 50(1):63–96, 2018.

[8] Afef Najjari, Mostafa S Elshahed, Ameur Cherif, and Noha H Youssef. Patterns and determinants of halophilic archaea (class halobacteria) diversity in tunisian endorheic salt lakes and sebkhet systems. *Applied and environmental microbiology*, 81(13):4432–4441, 2015.

[9] Katherine S Rawls, Jonathan H Martin, and Julie A Maupin-Furlow. Activity and transcriptional regulation of bacterial protein-like glycerol-3-phosphate dehydrogenase of the haloarchaea in haloferax volcanii. *Journal of bacteriology*, 193(17):4469–4476, 2011.

[10] A Rymaszewska and S Grenda. Bacteria of the genus anaplasma–characteristics of anaplasma and their vectors: a review. *Vet Med*, 53(11):573–584, 2008.

[11] Daad Saffarini, Ken Brockman, Alex Beliaev, Rachida Bouhenni, and Sheetal Shirodkar. Shewanella oneidensis and extracellular electron

transfer to metal oxides. In *Bacteria-Metal Interactions*, pages 21–40. Springer, 2015.

[12] Filipa L Sousa, Renato J Alves, Miguel A Ribeiro, José B Pereira-Leal, Miguel Teixeira, and Manuela M Pereira. The superfamily of heme–copper oxygen reductases: types and evolutionary considerations. *Biochimica et Biophysica Acta (BBA)-Bioenergetics*, 1817(4):629–637, 2012.

[13] Genfu Wu, Ning Li, Yinting Mao, Guangqi Zhou, and Haichun Gao. Endogenous generation of hydrogen sulfide and its regulation in shewanella oneidensis. *Frontiers in Microbiology*, 6:374, 2015.
